# Supplementary material for: Spatiotemporal dynamics of ionic reorganization near biological membrane interfaces
Source: arXiv:2407.11947 ancillary file (2024-07-16)
Supplement: Supplementary file 1 [file SM.pdf]

# Supplementary Material

## Spatiotemporal dynamics of ionic reorganization near biological membrane interfaces

Hyeonjoo Row<sup>1,2</sup>, Joshua B. Fernandes<sup>1</sup>, and Kranthi K. Mandadapu<sup>1,3</sup>, and Karthik Shekhar<sup>1,2,4</sup>

<sup>1</sup> Department of Chemical and Biomolecular Engineering, University of California, Berkeley, CA 94720, USA

<sup>2</sup> Helen Wills Neuroscience Institute, California Institute for Quantitative Biosciences, QB3, Center for Computational Biology, University of California, Berkeley, CA 94720, USA

<sup>3</sup> Chemical Sciences Division, Lawrence Berkeley National Laboratory, CA 94720, USA

<sup>4</sup> Biological Systems Division, Lawrence Berkeley National Laboratory, Berkeley, CA 94720, USA

### Contents

|                                                                        |           |
|------------------------------------------------------------------------|-----------|
| <b>I. System description and key modeling assumptions</b>              | <b>2</b>  |
| <b>II. Numerical methods</b>                                           | <b>3</b>  |
| 1. Weak formulation . . . . .                                          | 3         |
| 2. Finite element approximation . . . . .                              | 5         |
| 3. Finite element method implementation details . . . . .              | 8         |
| (a). Uniform pumping . . . . .                                         | 8         |
| (b). Localized pumping . . . . .                                       | 9         |
| <b>III. Spatially uniform pumping</b>                                  | <b>10</b> |
| 1. Application of Gauss’s law . . . . .                                | 11        |
| 2. Perturbation expansion . . . . .                                    | 11        |
| 3. Derivation of analytical solutions . . . . .                        | 14        |
| 4. The charging dynamics ( $0 < \bar{t} \leq \bar{\tau}^0$ ) . . . . . | 15        |
| 5. Maximum pumping rate . . . . .                                      | 17        |
| 6. The relaxation dynamics ( $\bar{t} > \bar{\tau}^0$ ) . . . . .      | 17        |
| <b>IV. Spatially localized pumping</b>                                 | <b>18</b> |
| 1. Point charge approximation . . . . .                                | 18        |
| (a). Derivation of exact solution . . . . .                            | 18        |
| (b). Image charge representation . . . . .                             | 20        |
| (c). Multipole expansion and asymptotic limits . . . . .               | 21        |
| (d). Solution for charge density at early times . . . . .              | 23        |
| 2. Near-field approximation . . . . .                                  | 25        |
| (a). Point charge spreading . . . . .                                  | 25        |
| (b). Application to channel problem . . . . .                          | 26        |
| (c). Maximal pumping rate and potential difference . . . . .           | 27        |
| 3. Long-time asymptotics . . . . .                                     | 29        |
| (a). Derivation of transformed solution . . . . .                      | 29        |
| (b). Expansion for large distances and times . . . . .                 | 30        |
| 4. Analysis of second moments . . . . .                                | 32        |
| (a). Early times . . . . .                                             | 32        |
| (b). Late times . . . . .                                              | 34        |
| 5. Relaxation dynamics . . . . .                                       | 35        |
| <b>V. Supplementary Movies</b>                                         | <b>36</b> |
| <b>References</b>                                                      | <b>36</b> |

This document is organized as follows. In Section I, we review the setup of the problem, the governing Poisson-Nernst-Planck (PNP) equations, boundary conditions, and key modeling assumptions introduced in the main text. Section II describes aspects of the finite element method (FEM) to obtain numerical solutions for the nonlinear PNP equations, including the derivations of the weak forms, and details underlying the implementation and convergence analysis. Section III considers the problem of spatially uniform pumping, and uses the linearized equations to derive analytical solutions for the charging and relaxation dynamics. Finally, in Section IV, we derive the analytical solutions to describe the charging and discharging dynamics for the problem of spatially localized pumping. We also consider the asymptotic limits to derive the early and late time behaviors both near and far from the transporter.

## I. System description and key modeling assumptions

As outlined in Sec. II of the main text, we consider the case of selective ion pumping through a lipid membrane that separates two large domains  $\bar{\Omega}^\alpha$  ( $\alpha \in \{I, II\}$ ) containing a symmetric monovalent electrolyte at equal concentration. The boundary of domain  $\bar{\Omega}^\alpha$  is denoted  $\partial\bar{\Omega}^\alpha$ . The system and notations used are summarized in Fig. S1.

We provide a summary of the non-dimensionalized governing equations and boundary conditions, i.e. Eqs. (4a)-(5d) of the main text. The non-dimensionalized PNP equations are

$$\frac{\partial \bar{\rho}^\alpha}{\partial t} + \bar{\nabla} \cdot \bar{\mathbf{j}}_\rho^\alpha = 0, \quad (\text{S.1})$$

$$\frac{\partial \bar{C}^\alpha}{\partial t} + \bar{\nabla} \cdot \bar{\mathbf{j}}_C^\alpha = 0, \quad (\text{S.2})$$

$$\bar{\nabla} \cdot \bar{\mathbf{D}}^\alpha = \bar{\rho}^\alpha, \quad (\text{S.3})$$

$$\bar{\nabla} \cdot \bar{\mathbf{D}}^M = 0, \quad (\text{S.4})$$

for domains  $\alpha \in \{I, II\}$  and membrane M, with the following constitutive laws

$$\bar{\mathbf{j}}_\rho^\alpha = -\bar{\nabla} \bar{\rho}^\alpha - (1 + \bar{C}^\alpha) \bar{\nabla} \bar{\phi}^\alpha, \quad (\text{S.5})$$

$$\bar{\mathbf{j}}_C^\alpha = -\bar{\nabla} \bar{C}^\alpha - \bar{\rho}^\alpha \bar{\nabla} \bar{\phi}^\alpha, \quad (\text{S.6})$$

$$\bar{\mathbf{D}}^\alpha = -\bar{\nabla} \bar{\phi}^\alpha, \quad (\text{S.7})$$

$$\bar{\mathbf{D}}^M = -\frac{1}{\bar{\Gamma}} \bar{\nabla} \bar{\phi}^M. \quad (\text{S.8})$$

The boundary conditions at the membrane-fluid interfaces  $\bar{S}^\alpha$  are given by

$$\bar{\phi}^\alpha = \bar{\phi}^M \quad \text{on } \bar{S}^\alpha, \quad \alpha \in \{I, II\}, \quad (\text{S.9})$$

$$\bar{\mathbf{D}}^\alpha \cdot \mathbf{n}^\alpha = \bar{\mathbf{D}}^M \cdot \mathbf{n}^\alpha \quad \text{on } \bar{S}^\alpha, \quad \alpha \in \{I, II\}, \quad (\text{S.10})$$

$$\bar{\mathbf{j}}_\rho^I \cdot \mathbf{n}^I = \bar{\mathbf{j}}_C^I \cdot \mathbf{n}^I = \bar{j}^o(\bar{x}, \bar{y}, \bar{t}) \quad \text{on } \bar{S}^I, \quad (\text{S.11})$$

$$\bar{\mathbf{j}}_\rho^{II} \cdot \mathbf{n}^{II} = \bar{\mathbf{j}}_C^{II} \cdot \mathbf{n}^{II} = -\bar{j}^o(\bar{x}, \bar{y}, \bar{t}) \quad \text{on } \bar{S}^{II}. \quad (\text{S.12})$$

We briefly comment on the boundary conditions at the other system boundaries  $\partial\bar{\Omega}^\alpha \setminus \bar{S}^\alpha$  (Fig. S1). The boundary conditions (S.11) and (S.12) specify the fluxes of the charge density and salt concentration at  $\bar{S}^\alpha$ . At all points  $\partial\bar{\Omega}^\alpha \setminus \bar{S}^\alpha$  we impose the conditions  $\bar{\mathbf{j}}_i^\alpha \cdot \mathbf{n}^\alpha = 0$  and  $\bar{\mathbf{D}}^\alpha \cdot \mathbf{n}^\alpha = 0$ . For an infinite system, these conditions imply a vanishing of the flux and the normal components of the electric fields at distances far from the site of ion transport. For a finite system, these conditions correspond to the system being closed and the system boundaries being electrically insulated. Equation (S.10) results from Gauss's law and the assumption of no surface charges on the membrane. We also assume  $\bar{\mathbf{D}}^M \cdot \mathbf{n}^M = 0$  on the boundary  $\partial\bar{\Omega}^M \setminus (\bar{S}^I \cup \bar{S}^{II})$ , corresponding to electrical insulation.

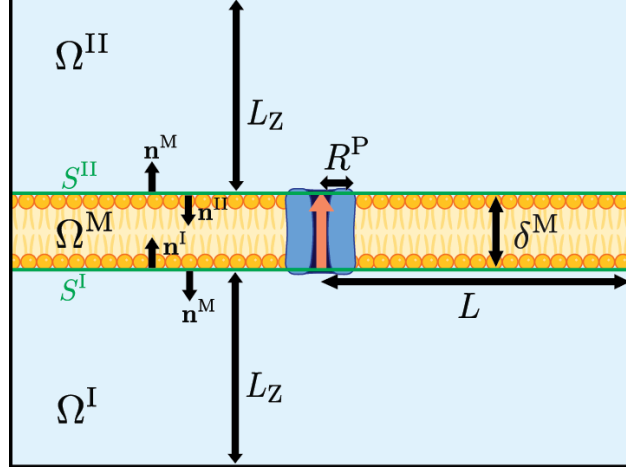

Figure S1: A schematic of the setup of the problem with all quantities labeled. Note that  $\bar{L}$  and  $\bar{R}^P$  enter only in the spatially localized pumping problem.

## II. Numerical methods

Equations (S.1)-(S.4) and the associated boundary conditions form a nonlinear system of partial differential equations (PDEs). We numerically solve these equations using the finite element method (FEM). To do so, we first derive the weak form of the PDEs in subsection II.1. Next, in subsection II.2, we obtain a discrete Galerkin approximation of the weak form and derive the equations governing the parameters of the approximation. We end with a description of the implementation details, the meshing strategy, and convergence studies in subsection II.3. The formalism presented here is drawn from Ref. [8].

### 1. Weak formulation

To derive the weak form of our problem, each Eq. (S.1)-(S.4) is multiplied by a test function corresponding to an *admissible variation*, integrated over its domain, and all the integrals are summed. This results in

$$\sum_{\alpha \in \{I, II\}} \left[ \int_{\bar{\Omega}^\alpha} \left( \frac{\partial \bar{\rho}^\alpha}{\partial t} + \bar{\nabla} \cdot \bar{\mathbf{j}}_\rho^\alpha \right) \delta \bar{\rho}^\alpha dv + \int_{\bar{\Omega}^\alpha} \left( \frac{\partial \bar{C}^\alpha}{\partial t} + \bar{\nabla} \cdot \bar{\mathbf{j}}_C^\alpha \right) \delta \bar{C}^\alpha dv + \int_{\bar{\Omega}^\alpha} (\bar{\nabla} \cdot \bar{\mathbf{D}}^\alpha - \bar{\rho}^\alpha) \delta \bar{\phi}^\alpha dv \right] + \int_{\bar{\Omega}^M} (\bar{\nabla} \cdot \bar{\mathbf{D}}^M) \delta \bar{\phi}^M dv = 0, \quad (\text{S.13})$$

where  $\delta \bar{\rho}^\alpha$ ,  $\delta \bar{C}^\alpha$ ,  $\delta \bar{\phi}^\alpha$ , and  $\delta \bar{\phi}^M$  are admissible variations. Recall that the electric displacement fields  $\bar{\mathbf{D}}^\alpha$  and  $\bar{\mathbf{D}}^M$  are related to the potentials  $\bar{\phi}^\alpha$  and  $\bar{\phi}^M$  through Eqs. (S.7)-(S.8). In what follows, we consider a single continuous potential field  $\bar{\phi}$  defined on  $\Omega$  together with an associated continuous variation  $\delta \bar{\phi}$ . This is tantamount to strongly enforcing the boundary condition (S.9), thereby automatically satisfying the continuity of the electric potential. The remaining boundary conditions (S.10)-(S.12) will be weakly enforced.

We now assume that all variations are sufficiently regular so that we can apply integration by parts to terms involving the fluxes  $\bar{\mathbf{j}}_\rho^\alpha$ ,  $\bar{\mathbf{j}}_C^\alpha$  and displacement fields  $\bar{\mathbf{D}}^\alpha$  and  $\bar{\mathbf{D}}^M$  in Eq. (S.13). To that end, we consider

$$\bar{\rho}^\alpha \in \mathcal{H}^1(\bar{\Omega}^\alpha), \quad \bar{C}^\alpha \in \mathcal{H}^1(\bar{\Omega}^\alpha), \quad \bar{\phi} \in \mathcal{H}^1(\bar{\Omega}), \quad (\text{S.14})$$

$$\delta \bar{\rho}^\alpha \in \mathcal{H}^1(\bar{\Omega}^\alpha), \quad \delta \bar{C}^\alpha \in \mathcal{H}^1(\bar{\Omega}^\alpha), \quad \delta \bar{\phi} \in \mathcal{H}^1(\bar{\Omega}), \quad (\text{S.15})$$

where  $\mathcal{H}^1(\bar{\Omega})$  denotes the first-order Sobolev space of functions on  $\bar{\Omega}$ . Drawing the admissible variations from these functional spaces guarantees that the integrals in the weak form are well-defined. Thus, replacing  $\delta \bar{\phi}^\alpha$  and  $\delta \bar{\phi}^M$  with  $\delta \bar{\phi}$  in the weak form as mentioned before and integrating by parts, Eq. (S.13) yields

$$\begin{aligned}
\sum_{\alpha \in \{I, II\}} & \left[ \int_{\bar{\Omega}^\alpha} \frac{\partial \bar{\rho}^\alpha}{\partial t} \delta \bar{\rho}^\alpha dv + \int_{\partial \bar{\Omega}^\alpha} (\bar{\mathbf{j}}_\rho^\alpha \cdot \mathbf{n}^\alpha) \delta \bar{\rho}^\alpha da - \int_{\bar{\Omega}^\alpha} \bar{\mathbf{j}}_\rho^\alpha \cdot \bar{\nabla} \delta \bar{\rho}^\alpha dv \right. \\
& + \int_{\bar{\Omega}^\alpha} \frac{\partial \bar{C}^\alpha}{\partial t} \delta \bar{C}^\alpha dv + \int_{\partial \bar{\Omega}^\alpha} (\bar{\mathbf{j}}_C^\alpha \cdot \mathbf{n}^\alpha) \delta \bar{C}^\alpha da - \int_{\bar{\Omega}^\alpha} \bar{\mathbf{j}}_C^\alpha \cdot \bar{\nabla} \delta \bar{C}^\alpha dv \\
& + \int_{\partial \bar{\Omega}^\alpha} (\bar{\mathbf{D}}^\alpha \cdot \mathbf{n}^\alpha) \delta \bar{\phi} da - \int_{\bar{\Omega}^\alpha} \bar{\mathbf{D}}^\alpha \cdot \bar{\nabla} \delta \bar{\phi} dv - \int_{\bar{\Omega}^\alpha} \bar{\rho}^\alpha \delta \bar{\phi} dv \Big] \\
& + \int_{\partial \bar{\Omega}^M} (\bar{\mathbf{D}}^M \cdot \mathbf{n}^M) \delta \bar{\phi} da - \int_{\bar{\Omega}^M} \bar{\mathbf{D}}^M \cdot \bar{\nabla} \delta \bar{\phi} dv = 0, \quad (\text{S.16})
\end{aligned}$$

for all admissible  $\delta \bar{\rho}^\alpha$ ,  $\delta \bar{C}^\alpha$ , and  $\delta \bar{\phi}$ . Rearranging Eq. (S.16) by grouping terms corresponding to the bulk and the boundaries we obtain

$$\begin{aligned}
& \left\{ \sum_{\alpha \in \{I, II\}} \left[ \int_{\bar{\Omega}^\alpha} \frac{\partial \bar{\rho}^\alpha}{\partial t} \delta \bar{\rho}^\alpha dv - \int_{\bar{\Omega}^\alpha} \bar{\mathbf{j}}_\rho^\alpha \cdot \bar{\nabla} \delta \bar{\rho}^\alpha dv + \int_{\bar{\Omega}^\alpha} \frac{\partial \bar{C}^\alpha}{\partial t} \delta \bar{C}^\alpha dv \right. \right. \\
& \quad \left. \left. - \int_{\bar{\Omega}^\alpha} \bar{\mathbf{j}}_C^\alpha \cdot \bar{\nabla} \delta \bar{C}^\alpha dv - \int_{\bar{\Omega}^\alpha} \bar{\mathbf{D}}^\alpha \cdot \bar{\nabla} \delta \bar{\phi} dv - \int_{\bar{\Omega}^\alpha} \bar{\rho}^\alpha \delta \bar{\phi} dv \right] - \int_{\bar{\Omega}^M} \bar{\mathbf{D}}^M \cdot \bar{\nabla} \delta \bar{\phi} dv \right\} \\
& + \underbrace{\left\{ \sum_{\alpha \in \{I, II\}} \left[ \int_{\partial \bar{\Omega}^\alpha} (\bar{\mathbf{j}}_\rho^\alpha \cdot \mathbf{n}^\alpha) \delta \bar{\rho}^\alpha da + \int_{\partial \bar{\Omega}^\alpha} (\bar{\mathbf{j}}_C^\alpha \cdot \mathbf{n}^\alpha) \delta \bar{C}^\alpha da \right] \right\}}_{\text{Boundary terms (flux)}} \\
& + \underbrace{\left\{ \sum_{\alpha \in \{I, II\}} \int_{\partial \bar{\Omega}^\alpha} (\bar{\mathbf{D}}^\alpha \cdot \mathbf{n}^\alpha) \delta \bar{\phi} da + \int_{\partial \bar{\Omega}^M} (\bar{\mathbf{D}}^M \cdot \mathbf{n}^M) \delta \bar{\phi} da \right\}}_{\text{Boundary terms (potential)}}. \quad (\text{S.17})
\end{aligned}$$

Consider the flux boundary terms in Eq. (S.17). Note that the integrals over  $\partial \bar{\Omega}^\alpha$  and  $\partial \bar{\Omega}^M$  can be split as

$$\int_{\partial \bar{\Omega}^\alpha} (\cdot) = \int_{\bar{S}^\alpha} (\cdot) + \int_{\partial \bar{\Omega}^\alpha \setminus \bar{S}^\alpha} (\cdot), \quad \text{for } \alpha \in \{I, II\}, \quad (\text{S.18})$$

$$\int_{\partial \bar{\Omega}^M} (\cdot) = \int_{\bar{S}^I} (\cdot) + \int_{\bar{S}^{II}} (\cdot) + \int_{\partial \bar{\Omega}^M \setminus (\bar{S}^I \cup \bar{S}^{II})} (\cdot). \quad (\text{S.19})$$

As  $\bar{\mathbf{j}}_i^\alpha \cdot \mathbf{n}^\alpha = 0$  on  $\partial \bar{\Omega}^\alpha \setminus \bar{S}^\alpha$ , this leads to

$$\int_{\partial \bar{\Omega}^I} (\bar{\mathbf{j}}_\rho^I \cdot \mathbf{n}^I) \delta \bar{\rho}^I da = \int_{\bar{S}^I} \bar{j}^\circ \delta \bar{\rho}^I da, \quad \int_{\partial \bar{\Omega}^{II}} (\bar{\mathbf{j}}_\rho^{II} \cdot \mathbf{n}^{II}) \delta \bar{\rho}^{II} da = - \int_{\bar{S}^{II}} \bar{j}^\circ \delta \bar{\rho}^{II} da, \quad (\text{S.20})$$

$$\int_{\partial \bar{\Omega}^I} (\bar{\mathbf{j}}_C^I \cdot \mathbf{n}^I) \delta \bar{C}^I da = \int_{\bar{S}^I} \bar{j}^\circ \delta \bar{C}^I da, \quad \int_{\partial \bar{\Omega}^{II}} (\bar{\mathbf{j}}_C^{II} \cdot \mathbf{n}^{II}) \delta \bar{C}^{II} da = - \int_{\bar{S}^{II}} \bar{j}^\circ \delta \bar{C}^{II} da, \quad (\text{S.21})$$

for the flux boundary terms. Note that  $\bar{j}^\circ \equiv \bar{j}^\circ(\bar{x}, \bar{y}, \bar{t})$  as defined in Eqs. (S.11) and (S.12). For the electric potential boundary terms in Eq. (S.17), the conditions  $\bar{\mathbf{D}}^\alpha \cdot \mathbf{n}^\alpha = 0$  on  $\partial \bar{\Omega}^\alpha \setminus \bar{S}^\alpha$  and  $\bar{\mathbf{D}}^M \cdot \mathbf{n}^M = 0$  on  $\partial \bar{\Omega}^M \setminus (\bar{S}^I \cup \bar{S}^{II})$  lead to

$$\int_{\partial \bar{\Omega}^\alpha} (\bar{\mathbf{D}}^\alpha \cdot \mathbf{n}^\alpha) \delta \bar{\phi} da = \int_{\bar{S}^\alpha} (\bar{\mathbf{D}}^\alpha \cdot \mathbf{n}^\alpha) \delta \bar{\phi} da, \quad \text{for } \alpha \in \{I, II\}, \quad (\text{S.22})$$

$$\int_{\partial \bar{\Omega}^M} (\bar{\mathbf{D}}^M \cdot \mathbf{n}^M) \delta \bar{\phi} da = \int_{\bar{S}^I} (\bar{\mathbf{D}}^M \cdot \mathbf{n}^M) \delta \bar{\phi} da + \int_{\bar{S}^{II}} (\bar{\mathbf{D}}^M \cdot \mathbf{n}^M) \delta \bar{\phi} da. \quad (\text{S.23})$$

Adding the above equations, noting that  $\delta \bar{\phi}$  is continuous at the interfaces  $\bar{S}^\alpha$  and  $\mathbf{n}^M = -\mathbf{n}^\alpha$  (Fig. S1), we

obtain

$$\begin{aligned} \sum_{\alpha \in \{I, II\}} \int_{\partial\Omega^\alpha} (\bar{\mathbf{D}}^\alpha \cdot \mathbf{n}^\alpha) \delta\bar{\phi} da + \int_{\partial\Omega^M} (\bar{\mathbf{D}}^M \cdot \mathbf{n}^M) \delta\bar{\phi} da \\ = \sum_{\alpha \in \{I, II\}} \int_{\bar{S}^\alpha} ((\bar{\mathbf{D}}^\alpha - \bar{\mathbf{D}}^M) \cdot \mathbf{n}^\alpha) \delta\bar{\phi} da = 0, \end{aligned} \quad (\text{S.24})$$

from boundary conditions in Eq. (S.10). Thus, the potential boundary terms in Eq. (S.17) can be set to zero.

With Eqs. (S.20), (S.21), and (S.24), the total weak form Eq. (S.17) reduces to

$$\begin{aligned} \sum_{\alpha \in \{I, II\}} \left[ \int_{\bar{\Omega}^\alpha} \frac{\partial \bar{\rho}^\alpha}{\partial t} \delta\bar{\rho}^\alpha dv - \int_{\bar{\Omega}^\alpha} \bar{\mathbf{J}}_\rho^\alpha \cdot \bar{\nabla} \delta\bar{\rho}^\alpha dv + \int_{\bar{\Omega}^\alpha} \frac{\partial \bar{C}^\alpha}{\partial t} \delta\bar{C}^\alpha dv - \int_{\bar{\Omega}^\alpha} \bar{\mathbf{J}}_C^\alpha \cdot \bar{\nabla} \delta\bar{C}^\alpha dv - \int_{\bar{\Omega}^\alpha} \bar{\rho}^\alpha \delta\bar{\phi} dv \right] \\ - \int_{\bar{\Omega}} \bar{\mathbf{D}} \cdot \bar{\nabla} \delta\bar{\phi} dv + \int_{\bar{S}^I} \bar{j}^\circ \delta\bar{\rho}^I da + \int_{\bar{S}^I} \bar{j}^\circ \delta\bar{C}^I da - \int_{\bar{S}^{II}} \bar{j}^\circ \delta\bar{\rho}^{II} da - \int_{\bar{S}^{II}} \bar{j}^\circ \delta\bar{C}^{II} da = 0, \end{aligned} \quad (\text{S.25})$$

where we combine the three integrals of  $\bar{\mathbf{D}} \cdot \bar{\nabla} \delta\bar{\phi}$  over each domain. Equation (S.25) completes the weak formulation of the problem.

## 2. Finite element approximation

We now describe the FEM approximation of the solution to the PNP equations based on the weak form in Eq. (S.25). In FEM, each solution field (e.g.  $\bar{\rho}^\alpha(\mathbf{x}, t)$ ) and its associated admissible variation (e.g.  $\delta\bar{\rho}^\alpha(\mathbf{x}, t)$ ) are restricted to a specific spatial domain (e.g.  $\bar{\Omega}^\alpha$ ). We then choose suitable sets of basis functions to approximate the field and its variation, respectively, in the corresponding domain. In this work, we use the *same* basis function set to approximate all solution fields and their associated variations in a given domain, corresponding to the so-called *Bubnov-Galerkin* approach.

The fields  $\bar{\rho}^\alpha$  and  $\bar{C}^\alpha$  in the domain  $\bar{\Omega}^\alpha$  ( $\alpha \in \{I, II\}$ ) are approximated using the spatial basis functions  $N_I^\alpha(\mathbf{x})$  for  $I = 1, \dots, N$ , with  $N$  being the number of nodes in the corresponding domain. For approximating  $\bar{\phi}$  throughout the domain  $\bar{\Omega}$ , we use a different basis set denoted by  $P_I(\mathbf{x})$  for  $I = 1, \dots, P$ , with  $P$  being the number of nodes in the entire system. Both  $N$  and  $P$  increase with the spatial resolution of the discretization, and specific choices of  $N_I^\alpha(\mathbf{x})$  and  $P_I(\mathbf{x})$  are discussed in the following section.

The FEM approximations for  $\bar{\rho}^\alpha$ ,  $\bar{C}^\alpha$ , and  $\bar{\phi}$  are

$$\bar{\rho}^\alpha(\mathbf{x}, t) = \sum_{I=1}^N \bar{\rho}_I^\alpha(t) N_I^\alpha(\mathbf{x}), \quad \bar{C}^\alpha(\mathbf{x}, t) = \sum_{I=1}^N \bar{C}_I^\alpha(t) N_I^\alpha(\mathbf{x}), \quad \bar{\phi}(\mathbf{x}, t) = \sum_{I=1}^P \bar{\phi}_I(t) P_I(\mathbf{x}), \quad (\text{S.26})$$

where  $\bar{\rho}_I^\alpha$ ,  $\bar{C}_I^\alpha$ , and  $\bar{\phi}_I$  are temporally-varying coefficients that we solve for. We use the same basis sets to represent the corresponding variations in the fields

$$\delta\bar{\rho}^\alpha(\mathbf{x}, t) = \sum_{I=1}^N \delta\bar{\rho}_I^\alpha(t) N_I^\alpha(\mathbf{x}), \quad \delta\bar{C}^\alpha(\mathbf{x}, t) = \sum_{I=1}^N \delta\bar{C}_I^\alpha(t) N_I^\alpha(\mathbf{x}), \quad \delta\bar{\phi}(\mathbf{x}, t) = \sum_{I=1}^P \delta\bar{\phi}_I(t) P_I(\mathbf{x}), \quad (\text{S.27})$$

for any coefficients  $\delta\bar{\rho}_I^\alpha$ ,  $\delta\bar{C}_I^\alpha$ , and  $\delta\bar{\phi}_I$  ( $\alpha \in \{I, II\}$ ).

Substituting the expressions for the variations in Eq. (S.27) into Eq. (S.25) results in

$$\begin{aligned} \sum_{\alpha \in \{I, II\}} \sum_{I=1}^N \left[ \delta\bar{\rho}_I^\alpha \left( \int_{\bar{\Omega}^\alpha} \frac{\partial \bar{\rho}^\alpha}{\partial t} N_I^\alpha dv - \int_{\bar{\Omega}^\alpha} \bar{\mathbf{J}}_\rho^\alpha \cdot \bar{\nabla} N_I^\alpha dv \pm \int_{\bar{S}^\alpha} \bar{j}^\circ N_I^\alpha da \right) \right. \\ \left. + \delta\bar{C}_I^\alpha \left( \int_{\bar{\Omega}^\alpha} \frac{\partial \bar{C}^\alpha}{\partial t} N_I^\alpha dv - \int_{\bar{\Omega}^\alpha} \bar{\mathbf{J}}_C^\alpha \cdot \bar{\nabla} N_I^\alpha dv \pm \int_{\bar{S}^\alpha} \bar{j}^\circ N_I^\alpha da \right) \right] \\ + \sum_{I=1}^P \delta\bar{\phi}_I \left( - \int_{\bar{\Omega}} \bar{\mathbf{D}} \cdot \bar{\nabla} P_I dv - \int_{\bar{\Omega}^I} \bar{\rho}^I P_I dv - \int_{\bar{\Omega}^{II}} \bar{\rho}^{II} P_I dv \right) = 0, \end{aligned} \quad (\text{S.28})$$

where the  $\pm$  in the summation is  $+$  for the integral in domain I and  $-$  for the integral in domain II. Since the above equation should hold for all variations  $\delta\bar{\rho}_I^\alpha(t)$ ,  $\delta\bar{C}_I^\alpha(t)$ , and  $\delta\bar{\phi}_I(t)$ , each of which is independent, we have the following system of  $4N + P$  equations:

$$\int_{\bar{\Omega}^I} \frac{\partial \bar{\rho}^I}{\partial t} N_I^I dv - \int_{\bar{\Omega}^I} \bar{\mathbf{j}}_\rho^I \cdot \bar{\nabla} N_I^I dv + \int_{\bar{S}^I} \bar{j}^\circ N_I^I da = 0, \quad I = 1, \dots, N \quad (\text{S.29})$$

$$\int_{\bar{\Omega}^I} \frac{\partial \bar{C}^I}{\partial t} N_I^I dv - \int_{\bar{\Omega}^I} \bar{\mathbf{j}}_C^I \cdot \bar{\nabla} N_I^I dv + \int_{\bar{S}^I} \bar{j}^\circ N_I^I da = 0, \quad I = 1, \dots, N \quad (\text{S.30})$$

$$\int_{\bar{\Omega}^{II}} \frac{\partial \bar{\rho}^{II}}{\partial t} N_I^{II} dv - \int_{\bar{\Omega}^{II}} \bar{\mathbf{j}}_\rho^{II} \cdot \bar{\nabla} N_I^{II} dv - \int_{\bar{S}^{II}} \bar{j}^\circ N_I^{II} da = 0, \quad I = 1, \dots, N \quad (\text{S.31})$$

$$\int_{\bar{\Omega}^{II}} \frac{\partial \bar{\rho}^{II}}{\partial t} N_I^{II} dv - \int_{\bar{\Omega}^{II}} \bar{\mathbf{j}}_\rho^{II} \cdot \bar{\nabla} N_I^{II} dv - \int_{\bar{S}^{II}} \bar{j}^\circ N_I^{II} da = 0, \quad I = 1, \dots, N \quad (\text{S.32})$$

$$- \int_{\bar{\Omega}} \bar{\mathbf{D}} \cdot \bar{\nabla} P_I dv - \int_{\bar{\Omega}^I} \bar{\rho}^I P_I dv - \int_{\bar{\Omega}^{II}} \bar{\rho}^{II} P_I dv = 0, \quad I = 1, \dots, P \quad (\text{S.33})$$

where the unknowns are the functions  $\bar{\rho}^\alpha$ ,  $\bar{C}^\alpha$ , and  $\bar{\phi}$ . We then substitute the basis representations of the unknown fields from Eq. (S.26) to express the equations in terms of the time-dependent coefficients. This gives

$$\sum_{J=1}^N \frac{d\bar{\rho}_J^I}{dt} \int_{\bar{\Omega}^I} N_J^I N_I^I dv - \int_{\bar{\Omega}^I} \bar{\mathbf{j}}_\rho^I \cdot \bar{\nabla} N_I^I dv + \int_{\bar{S}^I} \bar{j}^\circ N_I^I da = 0, \quad I = 1, \dots, N \quad (\text{S.34})$$

$$\sum_{J=1}^N \frac{d\bar{C}_J^I}{dt} \int_{\bar{\Omega}^I} N_J^I N_I^I dv - \int_{\bar{\Omega}^I} \bar{\mathbf{j}}_C^I \cdot \bar{\nabla} N_I^I dv + \int_{\bar{S}^I} \bar{j}^\circ N_I^I da = 0, \quad I = 1, \dots, N \quad (\text{S.35})$$

$$\sum_{J=1}^N \frac{d\bar{\rho}_J^{II}}{dt} \int_{\bar{\Omega}^{II}} N_J^{II} N_I^{II} dv - \int_{\bar{\Omega}^{II}} \bar{\mathbf{j}}_\rho^{II} \cdot \bar{\nabla} N_I^{II} dv - \int_{\bar{S}^{II}} \bar{j}^\circ N_I^{II} da = 0, \quad I = 1, \dots, N \quad (\text{S.36})$$

$$\sum_{J=1}^N \frac{d\bar{C}_J^{II}}{dt} \int_{\bar{\Omega}^{II}} N_J^{II} N_I^{II} dv - \int_{\bar{\Omega}^{II}} \bar{\mathbf{j}}_\rho^{II} \cdot \bar{\nabla} N_I^{II} dv - \int_{\bar{S}^{II}} \bar{j}^\circ N_I^{II} da = 0, \quad I = 1, \dots, N \quad (\text{S.37})$$

$$- \int_{\bar{\Omega}} \bar{\mathbf{D}} \cdot \bar{\nabla} P_I dv - \sum_{J=1}^N \left[ \bar{\rho}_J^I \int_{\bar{\Omega}^I} N_J^I P_I dv + \bar{\rho}_J^{II} \int_{\bar{\Omega}^{II}} N_J^{II} P_I dv \right] = 0, \quad I = 1, \dots, P \quad (\text{S.38})$$

which constitute a differential-algebraic system of equations (DAE) in terms of the  $4N + P$  time-dependent coefficients  $\bar{\rho}_I^\alpha$ ,  $\bar{C}_I^\alpha$ , and  $\bar{\phi}_I$ . Note that dependence on the values—not the derivatives—of the coefficients also enters through the constitutive laws for  $\bar{\mathbf{j}}_\rho^\alpha$ ,  $\bar{\mathbf{j}}_C^\alpha$ , and  $\bar{\mathbf{D}}$ . Moreover, the constitutive laws for  $\bar{\mathbf{j}}_\rho^\alpha$  and  $\bar{\mathbf{j}}_C^\alpha$  are nonlinear in nature, making this a nonlinear DAE system.

The nonlinear DAE system can be compactly represented. To that end, let us define our solution vector as

$$\mathbf{u} = [\bar{\rho}_I^I \quad \bar{C}_I^I \quad \bar{\rho}_I^{II} \quad \bar{C}_I^{II} \quad \bar{\phi}_I]^\top, \quad (\text{S.39})$$

which is a  $4N + P$  dimensional function in time. With this, Eqs. (S.34)-(S.38) can be rewritten compactly as

$$\mathbf{M}\dot{\mathbf{u}} + \mathbf{f}(\mathbf{u}) = \mathbf{0}, \quad (\text{S.40})$$

where  $\mathbf{f}$ , the *forcing vector*, is a nonlinear function of the coefficients  $\mathbf{u}$ , and  $\mathbf{M}$ , the *mass matrix*, is given by

$$\mathbf{M} = \begin{bmatrix} \mathbf{M}^I & & & \\ & \mathbf{M}^I & & \\ & & \mathbf{M}^{II} & \\ & & & \mathbf{M}^{II} \\ & & & & \mathbf{0} \end{bmatrix}, \quad (\text{S.41})$$

with  $\mathbf{M}^I, \mathbf{M}^{II} \in \mathbb{R}^{N \times N}$  and

$$M_{ij}^\alpha = \int_{\bar{\Omega}^\alpha} N_I^\alpha N_J^\alpha dv, \quad (\text{S.42})$$

for  $\alpha \in \{I, II\}$ . It can be seen that  $\mathbf{M}$  is not invertible since the potential has no explicit time dependence under the electrostatic approximation making implicit methods necessary for this DAE system. The forcing vector is

$$\mathbf{f}(\mathbf{u}) = \begin{bmatrix} -\int_{\Omega^I} \bar{\mathbf{j}}_\rho^I(\mathbf{u}) \cdot \bar{\nabla} N_I^I dv + \int_{\Gamma^I} \bar{j}^\circ N_I^I da \\ -\int_{\Omega^I} \bar{\mathbf{j}}_C^I(\mathbf{u}) \cdot \bar{\nabla} N_I^I dv + \int_{\Gamma^I} \bar{j}^\circ N_I^I da \\ -\int_{\Omega^{II}} \bar{\mathbf{j}}_\rho^{II}(\mathbf{u}) \cdot \bar{\nabla} N_I^{II} dv - \int_{\Gamma^{II}} \bar{j}^\circ N_I^{II} da \\ -\int_{\Omega^{II}} \bar{\mathbf{j}}_C^{II}(\mathbf{u}) \cdot \bar{\nabla} N_I^{II} dv - \int_{\Gamma^{II}} \bar{j}^\circ N_I^{II} da \\ -\int_{\Omega} \bar{\mathbf{D}}(\mathbf{u}) \cdot \bar{\nabla} P_I dv - \int_{\Omega^I} \bar{\rho}^I(\mathbf{u}) P_I dv - \int_{\Omega^{II}} \bar{\rho}^{II}(\mathbf{u}) P_I dv \end{bmatrix} = \begin{bmatrix} \mathbf{f}^{\rho^I} \\ \mathbf{f}^{C^I} \\ \mathbf{f}^{\rho^{II}} \\ \mathbf{f}^{C^{II}} \\ \mathbf{f}^\phi \end{bmatrix}, \quad (\text{S.43})$$

where the first four blocks are each of size  $N$ , corresponding to the charge density and salt concentration fields in domains I and II, and the fifth block is of size  $P$ , corresponding to the potential.

Estimation of the coefficients requires temporal integration of Eq. (S.40). Discretizing the time domain as  $t_0, t_1, \dots, t_K$  with time steps  $h_k = t_k - t_{k-1}$ , and denoting  $\mathbf{u}_h^k \equiv \mathbf{u}(t_k)$ , we approximate the time derivative using the backward Euler scheme:

$$\dot{\mathbf{u}}_h(t_k) \approx \frac{\mathbf{u}_h^k - \mathbf{u}_h^{k-1}}{h_k}, \quad (\text{S.44})$$

for time  $t_k$ . The time-discretized form of Eq. (S.40) is then

$$\mathbf{M} \left( \frac{\mathbf{u}_h^k - \mathbf{u}_h^{k-1}}{h_k} \right) + \mathbf{f}(\mathbf{u}_h^k) = \mathbf{0}, \quad (\text{S.45})$$

for each time step  $k = 1, \dots, K$ , with an initial condition  $\mathbf{u}_h^0$ . To solve, we use Newton's method by linearizing  $\mathbf{f}(\mathbf{u})$  around a point  $\mathbf{u}_0$ , yielding

$$\frac{1}{h_k} \mathbf{M}(\mathbf{u}_h^k - \mathbf{u}_h^{k-1}) + \mathbf{K}(\mathbf{u}_0)(\mathbf{u}_h^k - \mathbf{u}_0) + \mathbf{f}(\mathbf{u}_0) = \mathbf{0}, \quad (\text{S.46})$$

where  $\mathbf{K} \equiv \partial \mathbf{f} / \partial \mathbf{u}$  is the Jacobian matrix. Equation (S.46) is solved by iterating  $\mathbf{u}_0$  until the solution is reached (details provided below). The Jacobian matrix  $\mathbf{K}$  is given by

$$\mathbf{K} = \begin{bmatrix} \mathbf{K}^{\rho^I \rho^I} & \mathbf{K}^{\rho^I C^I} & \mathbf{0} & \mathbf{0} & \mathbf{K}^{\rho^I \phi} \\ \mathbf{K}^{C^I \rho^I} & \mathbf{K}^{C^I C^I} & \mathbf{0} & \mathbf{0} & \mathbf{K}^{C^I \phi} \\ \mathbf{0} & \mathbf{0} & \mathbf{K}^{\rho^{II} \rho^{II}} & \mathbf{K}^{\rho^{II} C^{II}} & \mathbf{K}^{\rho^{II} \phi} \\ \mathbf{0} & \mathbf{0} & \mathbf{K}^{C^{II} \rho^{II}} & \mathbf{K}^{C^{II} C^{II}} & \mathbf{K}^{C^{II} \phi} \\ \mathbf{K}^{\phi \rho^I} & \mathbf{0} & \mathbf{K}^{\phi \rho^{II}} & \mathbf{0} & \mathbf{K}^{\phi \phi} \end{bmatrix}, \quad (\text{S.47})$$

where we have decomposed  $\mathbf{K}$  into interacting block matrices  $\mathbf{K}^{XY}$ . Note that the charge density and concentration fields in one domain do not directly couple to the corresponding fields in the other domain. However, all fields interact with the potential field.

To compute the elements of the Jacobian matrix, we may observe from Eq. (S.26) that

$$\frac{\partial \bar{\rho}^\alpha}{\partial \bar{\rho}_I^\alpha} = N_I^\alpha, \quad \frac{\partial \bar{C}^\alpha}{\partial \bar{C}_I^\alpha} = N_I^\alpha, \quad \frac{\partial \bar{\phi}}{\partial \bar{\phi}_I} = P_I. \quad (\text{S.48})$$

Using the relations in Eq. (S.48), we can compute the components of the nonzero blocks of  $\mathbf{K}$  as

$$K_{IJ}^{\rho^\alpha \rho^\alpha} = -\frac{\partial}{\partial \bar{\rho}_J^\alpha} \int_{\Omega^\alpha} \bar{\mathbf{j}}_\rho^\alpha(\mathbf{u}) \cdot \bar{\nabla} N_I^\alpha dv = \int_{\Omega^\alpha} \bar{\nabla} N_J^\alpha \cdot \bar{\nabla} N_I^\alpha dv, \quad (\text{S.49})$$

$$K_{IJ}^{\rho^\alpha C^\alpha} = -\frac{\partial}{\partial \bar{C}_J^\alpha} \int_{\Omega^\alpha} \bar{\mathbf{j}}_\rho^\alpha(\mathbf{u}) \cdot \bar{\nabla} N_I^\alpha dv = \int_{\Omega^\alpha} N_J^\alpha \bar{\nabla} \bar{\phi} \cdot \bar{\nabla} N_I^\alpha dv, \quad (\text{S.50})$$

$$K_{IJ}^{\rho^\alpha \phi} = -\frac{\partial}{\partial \bar{\phi}_J} \int_{\Omega^\alpha} \bar{\mathbf{j}}_\rho^\alpha(\mathbf{u}) \cdot \bar{\nabla} N_I^\alpha dv = \int_{\Omega^\alpha} (1 + \bar{C}^\alpha) \bar{\nabla} P_J \cdot \bar{\nabla} N_I^\alpha dv, \quad (\text{S.51})$$

$$K_{IJ}^{C^\alpha \rho^\alpha} = -\frac{\partial}{\partial \bar{\rho}_J^\alpha} \int_{\Omega^\alpha} \bar{\mathbf{j}}_C^\alpha(\mathbf{u}) \cdot \bar{\nabla} N_I^\alpha dv = \int_{\Omega^\alpha} N_J^\alpha \bar{\nabla} \bar{\phi} \cdot \bar{\nabla} N_I^\alpha dv, \quad (\text{S.52})$$

$$K_{IJ}^{C^\alpha C^\alpha} = -\frac{\partial}{\partial \bar{C}_J^\alpha} \int_{\bar{\Omega}^\alpha} \bar{\mathbf{j}}_C^\alpha(\mathbf{u}) \cdot \bar{\nabla} N_I^\alpha dv = \int_{\bar{\Omega}^\alpha} \bar{\nabla} N_J^\alpha \cdot \bar{\nabla} N_I^\alpha dv, \quad (\text{S.53})$$

$$K_{IJ}^{C^\alpha \phi} = -\frac{\partial}{\partial \bar{\phi}_J} \int_{\bar{\Omega}^\alpha} \bar{\mathbf{j}}_C^\alpha(\mathbf{u}) \cdot \bar{\nabla} N_I^\alpha dv = \int_{\bar{\Omega}^\alpha} \bar{\rho}^\alpha \bar{\nabla} P_J \cdot \bar{\nabla} N_I^\alpha dv, \quad (\text{S.54})$$

$$K_{IJ}^{\phi \rho^\alpha} = -\frac{\partial}{\partial \bar{\rho}_J^\alpha} \int_{\bar{\Omega}^\alpha} \bar{\rho}^\alpha(\mathbf{u}) P_I dv = -\int_{\bar{\Omega}^\alpha} N_J^\alpha P_I dv, \quad (\text{S.55})$$

$$K_{IJ}^{\phi \phi} = -\frac{\partial}{\partial \bar{\phi}_J} \int_{\Omega} \bar{\mathbf{D}}(\mathbf{u}) \cdot \bar{\nabla} P_I dv = \int_{\Omega} \bar{\epsilon}(\bar{\mathbf{x}}) \bar{\nabla} P_J \cdot \bar{\nabla} P_I dv, \quad (\text{S.56})$$

for  $\alpha \in \{\text{I}, \text{II}\}$  where we define  $\bar{\epsilon}$  as the dimensionless permittivity, given by  $\bar{\epsilon}(\bar{\mathbf{x}}) = 1$  if  $\bar{\mathbf{x}} \in \bar{\Omega}^\alpha$  and  $\bar{\epsilon}(\bar{\mathbf{x}}) = 1/\bar{\Gamma}$  if  $\bar{\mathbf{x}} \in \bar{\Omega}^{\text{M}}$ . Note that  $\mathbf{K}$  is asymmetric due to the presence of  $\mathbf{K}^{C^\alpha \phi}$  and the absence of  $\mathbf{K}^{\phi C^\alpha}$  (as well as the fact that  $\mathbf{K}^{\rho^\alpha \phi} \neq (\mathbf{K}^{\phi \rho^\alpha})^\top$ ). Moreover, the nonlinearity of  $\mathbf{f}$  enters only into the blocks  $\mathbf{K}^{\rho^\alpha C^\alpha}$ ,  $\mathbf{K}^{\rho^\alpha \phi}$ ,  $\mathbf{K}^{C^\alpha \rho^\alpha}$ , and  $\mathbf{K}^{C^\alpha \phi}$ .

To perform the Newton iterations, we take our starting vector to be  $\mathbf{u}_0 = \mathbf{u}_h^{k-1}$ , the solution vector at the preceding time point. The solution for the next time point is found through an iterative procedure which is given by

$$\mathbf{u}_{l+1} = \mathbf{u}_l - \left( \frac{1}{h_k} \mathbf{M} + \mathbf{K}(\mathbf{u}_l) \right)^{-1} \left( \frac{1}{h_k} \mathbf{M} (\mathbf{u}_l - \mathbf{u}_h^{k-1}) + \mathbf{f}(\mathbf{u}_l) \right), \quad (\text{S.57})$$

for  $l \geq 0$ . We terminate the iterations when the residual  $\mathbf{r}(\mathbf{b})$  of Eq. (S.45) satisfies  $\|\mathbf{r}(\mathbf{u}_l)\| < \eta_1$  or  $\|\mathbf{u}_l - \mathbf{u}_{l-1}\| < \eta_2$ , with  $\eta_1 = 10^{-10}$  and  $\eta_2 = 0$  as specified tolerances. Here, we use only residual convergence since  $\eta_2 = 0$ . This process is repeated for each time step  $t_1, \dots, t_N$  to generate the complete trajectory  $\mathbf{u}(t_k)$ .

### 3. Finite element method implementation details

FEniCSx [2, 10, 11] is used to construct the basis functions, the residual, the Jacobian, and to solve the system of linear equations. The resulting linear system is solved using the direct solver MUMPS [3, 4]—any iterative methods did not show a performance improvement. Gmsh [6] is used for meshing. For all the numerical simulations,  $\bar{\delta}^{\text{M}} = 4$  and  $\bar{\Gamma} = 20$  are used. The following subsections describe the approach used to generate the meshes, convergence studies, and other details of the numerical implementations.

#### (a). Uniform pumping

The uniform pumping problem has a dependence on one spatial dimension,  $\bar{z}$ . Accordingly, a one-dimensional mesh is used. It is observed that variations in the solution fields are primarily limited to a length scale on the order of the Debye length ( $\lambda_D$ ) near the membrane surfaces, so a system size of  $\bar{L}_Z = 10^3$  is found to be sufficient to capture the behaviors of an infinite system.

**Meshing and time-stepping strategy:** The initial mesh is chosen to be very coarse starting with two elements within the membrane. In each electrolyte domain, the initial mesh had elements of size 2 in the first 10 Debye lengths from the membrane surface, one element for the next 20 Debye lengths, and one more element for the remaining  $(\bar{L}_Z - 30)$  Debye lengths, yielding a total of 16 overall elements. Mesh refinements are performed uniformly by subdividing each element from the initial mesh by a factor of 2. The final mesh has 7 spatial refinements, with a mesh size near the membrane of 0.01, sufficiently small to capture the variation of the fields with the Debye length. Linear elements were used for all field variables for the 1D problem.

Temporal refinement is performed similarly to the spatial one by halving the time step, with an initial time step of 10 and a total time of  $10^4$ . A total of 7 refinements are considered.

**Convergence study:** Numerical convergence studies of the fields are performed using the relative  $L_2$  errors based on the finest (mesh and time step) refinement solution given by

$$E_{\bar{\rho}} = \frac{\|\bar{\rho}_h - \bar{\rho}'_h\|_{\bar{\Omega}^{\text{I}} \cup \bar{\Omega}^{\text{II}}}}{\|\bar{\rho}'_h\|_{\bar{\Omega}^{\text{I}} \cup \bar{\Omega}^{\text{II}}}}, \quad E_{\bar{C}} = \frac{\|\bar{C}_h - \bar{C}'_h\|_{\bar{\Omega}^{\text{I}} \cup \bar{\Omega}^{\text{II}}}}{\|\bar{C}'_h\|_{\bar{\Omega}^{\text{I}} \cup \bar{\Omega}^{\text{II}}}}, \quad E_{\bar{\phi}} = \frac{\|\bar{\phi}_h - \bar{\phi}'_h\|_{\bar{\Omega}}}{\|\bar{\phi}'_h\|_{\bar{\Omega}}}, \quad (\text{S.58})$$

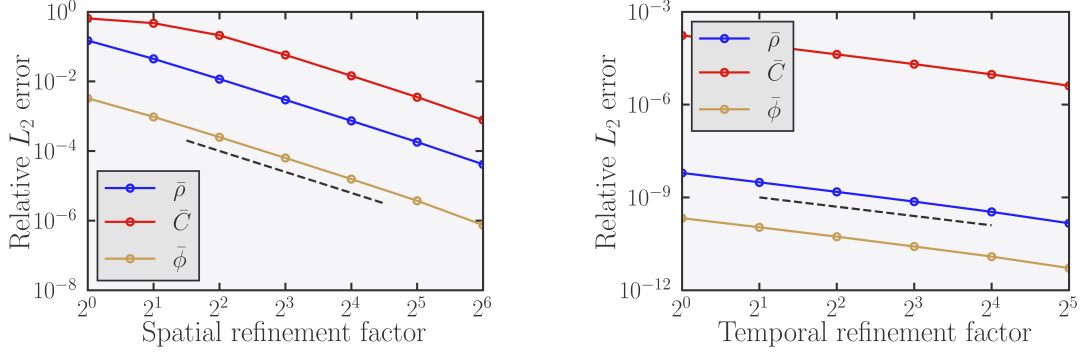

Figure S2: Left: the error metric at time  $\bar{t} = 10^4$  plotted for solutions computed with different spatial refinements. The dashed guideline shows second-order scaling. Right: the error metric at time  $\bar{t} = 10^4$  plotted for solutions computed with different temporal refinements. The dashed guideline shows first-order scaling.

with the  $L_2$  norm defined as

$$||u - v||_A = \sqrt{\int_A (u - v)^2 dA}, \quad (\text{S.59})$$

where  $u$  and  $v$  are any functions defined on a domain  $A$ . Here,  $(\cdot)'_h$  denotes the most refined numerical solution that is used as a reference, and  $(\cdot)_h$  is the corresponding less refined solution.

Figure S2 shows the error convergence plots, where we see a second-order convergence with the spatial refinement factor and a first-order convergence with the temporal refinement factor. Both of these are the expected rates of convergence for a linear problem solved with linear elements.

### (b). Localized pumping

The single transporter setup is shown in Fig. S1. Due to its axisymmetric nature, the numerical domain is considered to be two-dimensional in  $\bar{r}$  and  $\bar{z}$ . Given the long-range nature of electrostatic effects, a large system size is needed to achieve a system representative of the infinite system. From running numerical simulations of different system sizes, a radial size of  $L/\lambda_D = 10^6$  is found to be sufficient to capture the phenomena of the infinite system predicted from the analytical theory (see later sections). A system size of  $L_Z = 2L$  is maintained for all simulations. A pore radius of  $\bar{R}^P = 0.1$  is used throughout the article for numerical simulations.

**Meshing strategy:** As mentioned in the main text, a number of length and time scales arise when analyzing the single transporter. Relevant for numerical simulations are resolutions of the diffuse charge layers on either side of the membrane that span a Debye length, and the long-range effects that span the system size. The following describes the meshing strategy to resolve the behaviors over these multiple-length scales.

We use an overall anisotropic quadrilateral mesh given the asymmetric nature of the decay of the fields in the radial and axial directions. To resolve the decay of the fields in the diffuse charge layers, we divide the axial direction of the electrolyte domain into two regions, which consist of an anisotropic unstructured mesh within  $20 \lambda_D$  of the membrane and a largely isotropic unstructured mesh away from this region (see Fig. S3(a) and (c)). The mesh has a finer resolution close to the membrane and coarsens as we move outward from the transporter both axially and radially. The sizes of the elements are increased geometrically in both the radial and axial directions. The unstructured portion of the mesh in the electrolyte domain is constructed with quadrilateral elements using the software Gmsh and the Blossom-Quad algorithm [9] (see Fig. S3(e)). The Blossom-Quad algorithm produces approximately isotropic elements (avoiding highly stretched elements). The membrane portion consists of a structured mesh, with element sizes again increasing geometrically both in the radial direction and in the axial direction from the membrane-fluid interfaces to its center. A finer mesh at the membrane-fluid interfaces in the axial direction is required to satisfy the electric displacement field boundary conditions. Note that there exist highly anisotropic elements with large aspect ratios in the

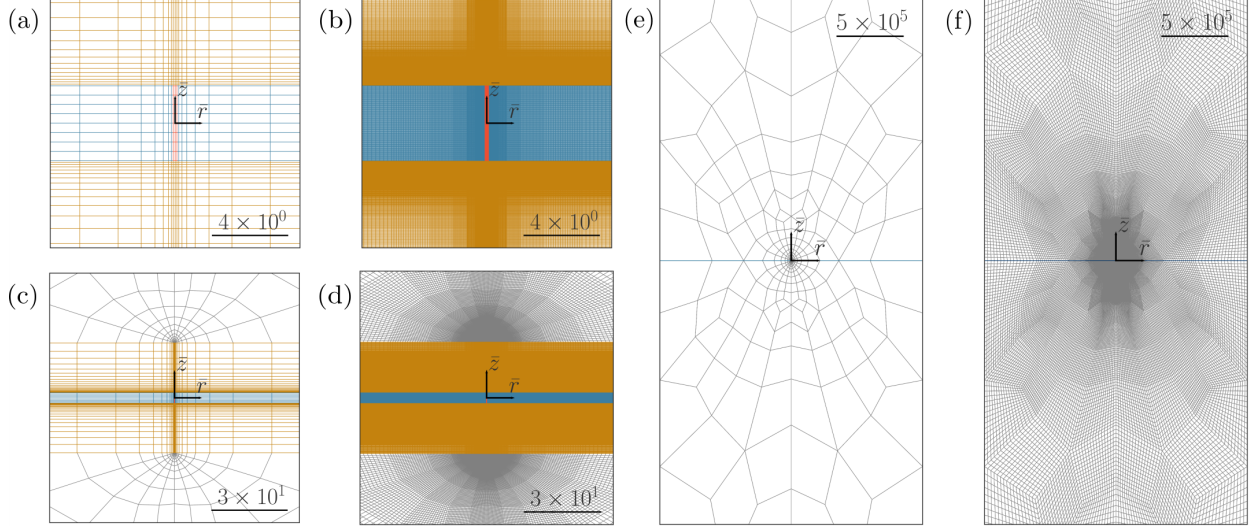

Figure S3: Cross-sections of the 3D mesh with axisymmetric elements in  $\bar{r}$  and  $\bar{z}$ . (a) and (b) A zoomed-in view of the mesh near the transporter showing the structured portion on the coarsest and finest refinements, respectively. In red, the location of the channel within the membrane centered at  $\bar{r} = 0$  with width  $\bar{R}^P = 0.1$ ; in blue, the membrane with thickness  $\bar{\delta}^M = 4$ ; and in gold, the structured portion of the interfacial electrolyte region with height 20. (c) and (d) A slightly zoomed-out view of the mesh, again on the coarsest and finest refinements, showing the transition to the unstructured portion of the mesh in the electrolyte domains (gray region). (e) and (f) show the entire mesh for a system size of  $\bar{L} = 10^6$ . On these scales, the membrane is rendered simply as a line—the channel and structured mesh in the interfacial region are not visible.

structured portion and at the structured-unstructured boundaries near the outer edges of the domains; they, nevertheless, did not pose any issues with convergence. Bilinear elements were used in all of the numerical simulations for the single transporter problem.

Mesh refinement for convergence studies is performed uniformly, by bisecting each edge in the mesh and adding a new node at the center point of each element, thus splitting each element in the coarser mesh into four new elements; see Figs. S3(b,d,f) for a refined mesh. A total of 4 mesh refinements are made, with the finest mesh resulting in approximately 1.6 million degrees of freedom.

Temporal refinement is performed similarly to the 1D problem by halving each time step. However, unlike in the uniform transport case, non-uniform time stepping is employed to resolve multiple time scales that arise in the problem, with an increasing time step size towards the final time. This is necessary to characterize the initial response of the fields within the Debye time ( $\tau_D$ ), and to analyze the late time propagation of the electric fields for the duration of the channel open times ( $\tau_o \gg \tau_D$ ). A total of 7 timestep refinements are made, with the lowest timestep ranging from 0.008 at early times to 8 at long times.

**Convergence study:** The error metric is exactly as described in the uniform transport section and given by Eq. (S.58). Figure S4 shows the error convergence plots, where we again see the expected second-order convergence in the spatial refinement factor and first-order convergence in the temporal refinement factor. Both of these are the expected rates of convergence for a linear problem solved with bilinear elements.

### III. Spatially uniform pumping

In this section, we derive analytical solutions to the linearized PNP equations for the case of spatially uniform pumping presented in Sec. III of the main text.

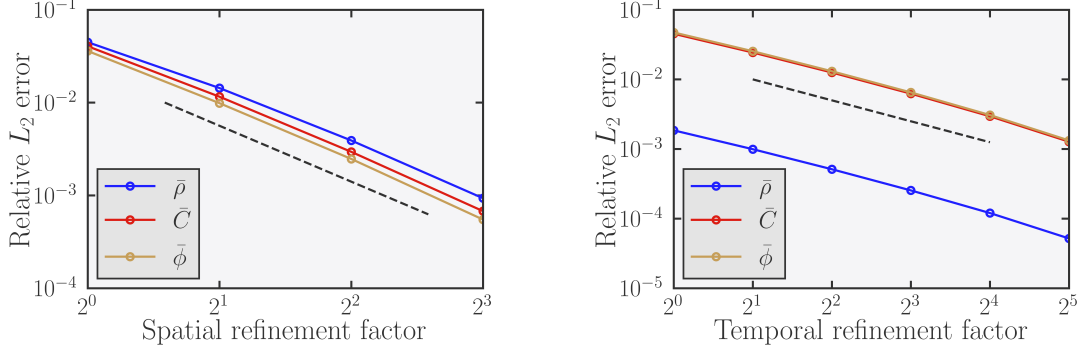

Figure S4: Left: the error metric at time  $\bar{t} = 10^3$  plotted for solutions computed with different spatial refinements. The guideline shows second-order scaling. Right: the error metric at time  $\bar{t} = 10^3$  plotted for solutions computed with different temporal refinements. The guideline shows first-order scaling.

## 1. Application of Gauss's law

For the case of uniform pumping the only relevant spatial dimension is the axial coordinate  $\bar{z}$ . Therefore, we can apply Gauss's law (integrating Poisson's equation) from  $\bar{z} \rightarrow -\infty$  to any  $\bar{z}^M \in (-\bar{\delta}^M/2, \bar{\delta}^M/2)$ . This gives

$$-\frac{1}{\bar{\Gamma}} \left. \frac{\partial \bar{\phi}^M}{\partial \bar{z}} \right|_{\bar{z}^M} + \lim_{\bar{z} \rightarrow -\infty} \frac{\partial \bar{\phi}^I}{\partial \bar{z}} = \bar{Q}_{\text{enc}} , \quad (\text{S.60})$$

where  $\bar{Q}_{\text{enc}}$  is the enclosed charge per area between  $-\infty$  and  $\bar{z}^M$ . We can write

$$\bar{Q}_{\text{enc}} = -\bar{Q}(\bar{t}) = -\bar{j}_0^o \min\{\bar{t}, \bar{\tau}^o\} , \quad (\text{S.61})$$

since the total enclosed charge is equal to the amount pumped across the membrane and the membrane is charge free. Using our boundary condition at infinity, i.e.  $\lim_{\bar{z} \rightarrow -\infty} \bar{\mathbf{D}}^I \cdot \mathbf{e}_z = 0$ , Eq. (S.60) yields

$$\frac{\partial \bar{\phi}^M}{\partial \bar{z}} = \bar{\Gamma} \bar{Q}(\bar{t}) , \quad (\text{S.62})$$

everywhere in the membrane. Thus, we find that the potential drop across the membrane is

$$\Delta \bar{V}^M = \int_{-\bar{\delta}^M/2}^{\bar{\delta}^M/2} \frac{\partial \bar{\phi}^M}{\partial \bar{z}} d\bar{z} = \bar{\Gamma} \bar{\delta}^M \bar{Q}(\bar{t}) , \quad (\text{S.63})$$

as given in the main text, with  $\bar{Q}(\bar{t})$  representing the total pumped charge.

## 2. Perturbation expansion

As stated in the main text, physiological transmembrane potential differences  $\Delta \bar{V}^M \sim 1$  are achieved by  $\bar{Q}^{\text{tot}} \ll 1$ . Since  $\bar{j}_0^o = \bar{Q}^{\text{tot}}/\bar{\tau}^o$  and  $\bar{\tau}^o \gg 1$ , we also conclude that  $\bar{j}_0^o \ll 1$ . This motivates a perturbation analysis for small  $\bar{j}_0^o$ . We begin the analysis by substituting the constitutive laws in Eqs. (S.5)-(S.8) into Eqs. (S.1)-(S.4), which yields

$$\frac{\partial \bar{\rho}^\alpha}{\partial \bar{t}} = \bar{\nabla}^2 \bar{\rho}^\alpha + \bar{\nabla} \cdot [(1 + \bar{C}^\alpha) \bar{\nabla} \bar{\phi}^\alpha] , \quad (\text{S.64})$$

$$\frac{\partial \bar{C}^\alpha}{\partial \bar{t}} = \bar{\nabla}^2 \bar{C}^\alpha + \bar{\nabla} \cdot [\bar{\rho}^\alpha \bar{\nabla} \bar{\phi}^\alpha] , \quad (\text{S.65})$$

$$\bar{\nabla}^2 \bar{\phi}^\alpha = -\bar{\rho}^\alpha , \quad (\text{S.66})$$

for  $\alpha \in \{\text{I}, \text{II}\}$  and

$$\bar{\nabla}^2 \bar{\phi}^{\text{M}} = 0 , \quad (\text{S.67})$$

inside the membrane. With the convention  $\mathbf{n}^{\text{I}} = \mathbf{e}_z$  and  $\mathbf{n}^{\text{II}} = -\mathbf{e}_z$  (Fig. S1, and Fig. 1 of the main text), the boundary conditions (S.9)-(S.12) become

$$\bar{\phi}^\alpha = \bar{\phi}^{\text{M}} , \quad (\text{S.68})$$

$$\frac{\partial \bar{\phi}^\alpha}{\partial \bar{z}} = \frac{1}{\bar{\Gamma}} \frac{\partial \bar{\phi}^{\text{M}}}{\partial \bar{z}} , \quad (\text{S.69})$$

$$\frac{\partial \bar{\rho}^\alpha}{\partial \bar{z}} + (1 + \bar{C}^\alpha) \frac{\partial \bar{\phi}^\alpha}{\partial \bar{z}} = -\bar{j}^\circ(\bar{x}, \bar{y}, \bar{t}) , \quad (\text{S.70})$$

$$\frac{\partial \bar{C}^\alpha}{\partial \bar{z}} + \bar{\rho}^\alpha \frac{\partial \bar{\phi}^\alpha}{\partial \bar{z}} = -\bar{j}^\circ(\bar{x}, \bar{y}, \bar{t}) , \quad (\text{S.71})$$

each on  $\bar{S}^\alpha$  for  $\alpha \in \{\text{I}, \text{II}\}$ . Note that the transmembrane flux  $\bar{j}^\circ$  is a function of the in-plane coordinates  $\bar{x}$  and  $\bar{y}$ , and time  $\bar{t}$ . Expanding out the divergence term in the charge balance, Eq. (S.64), gives

$$\frac{\partial \bar{\rho}^\alpha}{\partial \bar{t}} = \bar{\nabla}^2 \bar{\rho}^\alpha + \bar{\nabla}^2 \bar{\phi}^\alpha + \bar{\nabla} \cdot [\bar{C}^\alpha \bar{\nabla} \bar{\phi}^\alpha] , \quad (\text{S.72})$$

and using Poisson's equation (S.66) we obtain

$$\frac{\partial \bar{\rho}^\alpha}{\partial \bar{t}} = \bar{\nabla}^2 \bar{\rho}^\alpha - \bar{\rho}^\alpha + \bar{\nabla} \cdot [\bar{C}^\alpha \bar{\nabla} \bar{\phi}^\alpha] . \quad (\text{S.73})$$

We now perform a regular perturbation analysis for small imposed fluxes, i.e.  $\bar{j}^\circ(\bar{x}, \bar{y}, \bar{t}) = \epsilon \bar{f}^\circ(\bar{x}, \bar{y}, \bar{t})$  with  $\epsilon \ll 1$  and  $\bar{f}^\circ(\bar{x}, \bar{y}, \bar{t}) \sim \mathcal{O}(1)$ . Here,  $\bar{f}^\circ$  encodes the spatial and temporal dependence of the flux. We pose asymptotic expansions:

$$\bar{\rho}^\alpha(\mathbf{x}, t; \epsilon) = \sum_{i=0}^{\infty} \epsilon^i \bar{\rho}_i^\alpha(\mathbf{x}, t) , \quad (\text{S.74})$$

$$\bar{C}^\alpha(\mathbf{x}, t; \epsilon) = \sum_{i=0}^{\infty} \epsilon^i \bar{C}_i^\alpha(\mathbf{x}, t) , \quad (\text{S.75})$$

$$\bar{\phi}^\alpha(\mathbf{x}, t; \epsilon) = \sum_{i=0}^{\infty} \epsilon^i \bar{\phi}_i^\alpha(\mathbf{x}, t) , \quad (\text{S.76})$$

$$\bar{\phi}^{\text{M}}(\mathbf{x}, t; \epsilon) = \sum_{i=0}^{\infty} \epsilon^i \bar{\phi}_i^{\text{M}}(\mathbf{x}, t) . \quad (\text{S.77})$$

Substituting these expansions into Eqs. (S.73), (S.65), and (S.66), we collect the terms with the same orders of  $\epsilon$ . The zeroth order corresponds to the situation of  $\bar{j}_0 = 0$ , which gives  $\bar{\rho}_0^\alpha = \bar{C}_0^\alpha = \bar{\phi}_0^\alpha = \bar{\phi}_0^{\text{M}} = 0$ —nothing occurs without pumping cations. The first order equations form a closed set of coupled linear PDEs:

$$\frac{\partial \bar{\rho}_1^\alpha}{\partial \bar{t}} = \bar{\nabla}^2 \bar{\rho}_1^\alpha - \bar{\rho}_1^\alpha , \quad (\text{S.78})$$

$$\frac{\partial \bar{C}_1^\alpha}{\partial \bar{t}} = \bar{\nabla}^2 \bar{C}_1^\alpha , \quad (\text{S.79})$$

$$\bar{\nabla}^2 \bar{\phi}_1^\alpha = -\bar{\rho}_1^\alpha , \quad (\text{S.80})$$

$$\bar{\nabla}^2 \bar{\phi}_1^{\text{M}} = 0 . \quad (\text{S.81})$$

The corresponding  $\mathcal{O}(\epsilon)$  interfacial boundary conditions are

$$\bar{\phi}_1^\alpha = \bar{\phi}_1^{\text{M}} , \quad (\text{S.82})$$

$$\frac{\partial \bar{\phi}_1^\alpha}{\partial \bar{z}} = \frac{1}{\bar{\Gamma}} \frac{\partial \bar{\phi}_1^{\text{M}}}{\partial \bar{z}} , \quad (\text{S.83})$$

$$\frac{\partial \bar{\rho}_1^\alpha}{\partial \bar{z}} + \frac{\partial \bar{\phi}_1^\alpha}{\partial \bar{z}} = -\bar{f}^o(\bar{x}, \bar{y}, \bar{t}) , \quad (\text{S.84})$$

$$\frac{\partial \bar{C}_1^\alpha}{\partial \bar{z}} = -\bar{f}^o(\bar{x}, \bar{y}, \bar{t}) , \quad (\text{S.85})$$

on  $\bar{S}^\alpha$  for  $\alpha \in \{\text{I}, \text{II}\}$ . It is evident from Eqs. (S.78)-(S.85) that the concentration field  $\bar{C}_1^\alpha$  evolves as in bare diffusion of an uncharged solute, and is independent from the other fields,  $\bar{\rho}_1^\alpha$  and  $\bar{\phi}_1$ . The evolution of the charge density described by Eq. (S.78) represents a diffusion equation with a linear sink term. Unlike the concentration field,  $\bar{\rho}_1^\alpha$  and  $\bar{\phi}_1$  are coupled via Poisson's equation (S.80) and the no-flux boundary condition Eq. (S.83).

With  $\mathcal{O}(\epsilon)$  as the leading order, we have  $\bar{\rho}^\alpha = \epsilon \bar{\rho}_1^\alpha + \mathcal{O}(\epsilon^2)$ , and similarly for all the other fields. Consequently, we multiply the linearized equations (S.78)-(S.85) with  $\epsilon$  to obtain the leading order equations as

$$\frac{\partial \bar{\rho}^\alpha}{\partial \bar{t}} = \bar{\nabla}^2 \bar{\rho}^\alpha - \bar{\rho}^\alpha , \quad (\text{S.86})$$

$$\frac{\partial \bar{C}^\alpha}{\partial \bar{t}} = \bar{\nabla}^2 \bar{C}^\alpha , \quad (\text{S.87})$$

$$\bar{\nabla}^2 \bar{\phi}^\alpha = -\bar{\rho}^\alpha , \quad (\text{S.88})$$

$$\bar{\nabla}^2 \bar{\phi}^{\text{M}} = 0 , \quad (\text{S.89})$$

subject to the boundary conditions

$$\bar{\phi}^\alpha = \bar{\phi}^{\text{M}} , \quad (\text{S.90})$$

$$\frac{\partial \bar{\phi}^\alpha}{\partial \bar{z}} = \frac{1}{\bar{\Gamma}} \frac{\partial \bar{\phi}^{\text{M}}}{\partial \bar{z}} , \quad (\text{S.91})$$

$$\frac{\partial \bar{\rho}^\alpha}{\partial \bar{z}} + \frac{\partial \bar{\phi}^\alpha}{\partial \bar{z}} = -\bar{j}^o(\bar{x}, \bar{y}, \bar{t}) , \quad (\text{S.92})$$

$$\frac{\partial \bar{C}^\alpha}{\partial \bar{z}} = -\bar{j}^o(\bar{x}, \bar{y}, \bar{t}) . \quad (\text{S.93})$$

on  $\bar{S}^\alpha$  for  $\alpha \in \{\text{I}, \text{II}\}$ . This completes the derivation of the linearized problem statement. We note that the procedure can be continued for the higher order perturbations, but the leading order solutions predict the charge dynamics accurately with physiological settings as shown in the main text.

For the case of uniform pumping—which has variations only in the  $\bar{z}$  direction—the Laplacian operator  $\bar{\nabla}^2$  reduces to the second derivative in the axial coordinate  $\bar{z}$ . Therefore, we can write the linearized equations (S.86)-(S.88) as

$$\frac{\partial \bar{\rho}^\alpha}{\partial \bar{t}} = \frac{\partial^2 \bar{\rho}^\alpha}{\partial \bar{z}^2} - \bar{\rho}^\alpha , \quad (\text{S.94})$$

$$\frac{\partial \bar{C}^\alpha}{\partial \bar{t}} = \frac{\partial^2 \bar{C}^\alpha}{\partial \bar{z}^2} , \quad (\text{S.95})$$

$$\frac{\partial^2 \bar{\phi}^\alpha}{\partial \bar{z}^2} = -\bar{\rho}^\alpha , \quad (\text{S.96})$$

in the domain  $\alpha \in \{\text{I}, \text{II}\}$  and Poisson's equation (S.89) as

$$\frac{\partial^2 \bar{\phi}^{\text{M}}}{\partial \bar{z}^2} = 0 , \quad (\text{S.97})$$

inside the membrane. The corresponding boundary conditions Eqs. (S.90)-(S.93) are now written as

$$\bar{\phi}^\alpha = \bar{\phi}^{\text{M}} \quad \text{at } \bar{z} = \pm \frac{\bar{\delta}^{\text{M}}}{2} , \quad (\text{S.98})$$

$$\frac{\partial \bar{\phi}^\alpha}{\partial \bar{z}} = \frac{1}{\bar{\Gamma}} \frac{\partial \bar{\phi}^{\text{M}}}{\partial \bar{z}} \quad \text{at } \bar{z} = \pm \frac{\bar{\delta}^{\text{M}}}{2} , \quad (\text{S.99})$$

$$\frac{\partial \bar{\rho}^I}{\partial \bar{z}} + \frac{\partial \bar{\phi}^I}{\partial \bar{z}} = -\bar{j}_0^\circ [\Theta(\bar{t}) - \Theta(\bar{t} - \bar{\tau}^\circ)] \quad \text{at } \bar{z} = -\frac{\bar{\delta}^M}{2}, \quad (\text{S.100})$$

$$\frac{\partial \bar{C}^I}{\partial \bar{z}} = -\bar{j}_0^\circ [\Theta(\bar{t}) - \Theta(\bar{t} - \bar{\tau}^\circ)] \quad \text{at } \bar{z} = -\frac{\bar{\delta}^M}{2}, \quad (\text{S.101})$$

$$\frac{\partial \bar{\rho}^{II}}{\partial \bar{z}} + \frac{\partial \bar{\phi}^{II}}{\partial \bar{z}} = -\bar{j}_0^\circ [\Theta(\bar{t}) - \Theta(\bar{t} - \bar{\tau}^\circ)] \quad \text{at } \bar{z} = \frac{\bar{\delta}^M}{2}, \quad (\text{S.102})$$

$$\frac{\partial \bar{C}^{II}}{\partial \bar{z}} = -\bar{j}_0^\circ [\Theta(\bar{t}) - \Theta(\bar{t} - \bar{\tau}^\circ)] \quad \text{at } \bar{z} = \frac{\bar{\delta}^M}{2}, \quad (\text{S.103})$$

where  $\bar{j}_0^\circ$  is the constant rate of pumping and  $\bar{\tau}^\circ$  is the duration for which the pump is operated, with  $\Theta(\cdot)$  being the standard Heaviside function.

### 3. Derivation of analytical solutions

It is clearly seen that the linearized governing equations (S.94)-(S.97) and the boundary conditions Eqs. (S.98)-(S.103) are odd under the reflection  $\bar{z} \rightarrow -\bar{z}$ . Therefore we only need to compute the solution for  $\bar{z} \geq 0$  (domain II), and the solution for the other domain is simply its negative, i.e.  $\bar{\rho}^{II}(\bar{z}, \bar{t}) = -\bar{\rho}^I(-\bar{z}, \bar{t})$ ,  $\bar{C}^{II}(\bar{z}, \bar{t}) = -\bar{C}^I(-\bar{z}, \bar{t})$ , and  $\bar{\phi}^{II}(\bar{z}, \bar{t}) = -\bar{\phi}^I(-\bar{z}, \bar{t})$ .

A general solution for the charge density  $\bar{\rho}^{II}$  can be found by decoupling its dynamics from that of  $\bar{\phi}^{II}$ . From the continuity of the electric displacement Eq. (S.99) and potential gradient inside the membrane Eq. (S.62), we obtain

$$\left. \frac{\partial \bar{\phi}^{II}}{\partial \bar{z}} \right|_{\bar{z}=\bar{\delta}^M/2} = \frac{1}{\bar{\Gamma}} \left. \frac{\partial \bar{\phi}^{IM}}{\partial \bar{z}} \right|_{\bar{z}=\bar{\delta}^M/2} = \bar{Q}(\bar{t}) = \bar{j}_0^\circ \min\{\bar{t}, \bar{\tau}^\circ\}. \quad (\text{S.104})$$

This can be substituted into the no-flux boundary condition Eq. (S.102) to yield the fully separated boundary conditions for domain II at  $\bar{z} = \bar{\delta}^M/2$ :

$$\frac{\partial \bar{\phi}^{II}}{\partial \bar{z}} = \bar{Q}(\bar{t}), \quad (\text{S.105})$$

$$\frac{\partial \bar{\rho}^{II}}{\partial \bar{z}} = -\bar{Q}(\bar{t}) - \bar{j}_0^\circ [\Theta(\bar{t}) - \Theta(\bar{t} - \bar{\tau}^\circ)], \quad (\text{S.106})$$

$$\frac{\partial \bar{C}^{II}}{\partial \bar{z}} = -\bar{j}_0^\circ [\Theta(\bar{t}) - \Theta(\bar{t} - \bar{\tau}^\circ)]. \quad (\text{S.107})$$

Defining

$$\bar{f}(\bar{t}) = \bar{Q}(\bar{t}) + \bar{j}_0^\circ [\Theta(\bar{t}) - \Theta(\bar{t} - \bar{\tau}^\circ)] = \bar{j}_0^\circ [\min\{\bar{t}, \bar{\tau}^\circ\} + \Theta(\bar{t}) - \Theta(\bar{t} - \bar{\tau}^\circ)], \quad (\text{S.108})$$

as a “driving function”, the charge density in domain II (dropping the superscript) satisfies

$$\frac{\partial \bar{\rho}}{\partial \bar{t}} = \frac{\partial^2 \bar{\rho}}{\partial \bar{z}^2} - \bar{\rho}, \quad (\text{S.109})$$

subject to the boundary conditions

$$\frac{\partial \bar{\rho}}{\partial \bar{z}} = -\bar{f}(\bar{t}), \quad \text{at } \bar{z} = \frac{\bar{\delta}^M}{2}, \quad (\text{S.110})$$

$$\frac{\partial \bar{\rho}}{\partial \bar{z}} = 0, \quad \text{as } \bar{z} \rightarrow \infty, \quad (\text{S.111})$$

and the initial condition  $\bar{\rho}(\bar{z}, 0) = 0$ . Lastly, we introduce a change of variable  $\bar{z}' \equiv \bar{z} - \bar{\delta}^M/2$  such that domain II occupies  $0 < \bar{z}' < \infty$ .

Equations (S.109)-(S.111) can be solved by using the Fourier cosine transform, which is a standard solution method to solve differential equations in a semi-infinite domain with a Neumann boundary condition. The transform is defined by

$$\hat{\rho}(\hat{k}, \bar{t}) = \mathcal{C}(\bar{\rho}) = \sqrt{\frac{2}{\pi}} \int_0^\infty \bar{\rho}(\bar{z}', \bar{t}) \cos(\hat{k} \bar{z}') d\bar{z}', \quad (\text{S.112})$$

which satisfies

$$\bar{\rho} = \mathcal{C}(\mathcal{C}(\bar{\rho})) , \quad (\text{S.113})$$

implying the transform is self-inverse. It is useful to note

$$\mathcal{C}\left(\frac{\partial^2 \bar{\rho}}{\partial \bar{z}'^2}\right) = -\sqrt{\frac{2}{\pi}} \left(\frac{\partial \bar{\rho}}{\partial \bar{z}'}\right)_{\bar{z}'=0} - \hat{k}^2 \mathcal{C}(\bar{\rho}) , \quad (\text{S.114})$$

which can be shown by integrating by parts twice. Applying the cosine transform to Eq. (S.109) and the initial condition gives the ordinary differential equation

$$\frac{\partial \hat{\rho}}{\partial \bar{t}} = \sqrt{\frac{2}{\pi}} \bar{f}(\bar{t}) - (1 + \hat{k}^2) \hat{\rho} , \quad (\text{S.115})$$

subject to the condition  $\hat{\rho}(\hat{k}, 0) = 0$ . Equation (S.115) can be solved exactly to yield

$$\hat{\rho}(\hat{k}, \bar{t}) = \sqrt{\frac{2}{\pi}} \int_0^{\bar{t}} \bar{f}(\bar{t} - \bar{\tau}) e^{-(1+\hat{k}^2)\bar{\tau}} d\bar{\tau} . \quad (\text{S.116})$$

Applying the inverse cosine transform results in the real space solution

$$\bar{\rho}(\bar{z}', \bar{t}) = \frac{2}{\pi} \int_0^{\infty} \int_0^{\bar{t}} \bar{f}(\bar{t} - \bar{\tau}) e^{-(1+\hat{k}^2)\bar{\tau}} d\bar{\tau} \cos(\hat{k}\bar{z}') d\hat{k} . \quad (\text{S.117})$$

Swapping the order of integrations in Eq. (S.117), we rewrite it as

$$\bar{\rho}(\bar{z}', \bar{t}) = \frac{2}{\pi} \int_0^{\bar{t}} \bar{f}(\bar{t} - \bar{\tau}) e^{-\bar{\tau}} \int_0^{\infty} e^{-\hat{k}^2 \bar{\tau}} \cos(\hat{k}\bar{z}') d\hat{k} d\bar{\tau} . \quad (\text{S.118})$$

Here, the second integral is a Gaussian integral, and is evaluated as

$$\int_0^{\infty} e^{-\hat{k}^2 \bar{\tau}} \cos(\hat{k}\bar{z}') d\hat{k} = \frac{\sqrt{\pi}}{2} \frac{1}{\sqrt{\bar{\tau}}} e^{-\bar{z}'^2/4\bar{\tau}} . \quad (\text{S.119})$$

The real-space solution then is

$$\bar{\rho}(\bar{z}', \bar{t}) = \frac{1}{\sqrt{\pi}} \int_0^{\bar{t}} \bar{f}(\bar{t} - \bar{\tau}) e^{-\bar{\tau}} \frac{1}{\sqrt{\bar{\tau}}} e^{-\bar{z}'^2/4\bar{\tau}} d\bar{\tau} , \quad (\text{S.120})$$

for the driving function  $\bar{f}(\bar{t})$ . The real space solution can also be written as

$$\bar{\rho}(\bar{z}', \bar{t}) = \int_0^{\bar{t}} \bar{f}(\bar{t} - \bar{\tau}) \frac{e^{-\bar{\tau}}}{\sqrt{\pi\bar{\tau}}} e^{-\bar{z}'^2/4\bar{\tau}} d\bar{\tau} \equiv 2\bar{f} * \left( \frac{e^{-\bar{t}}}{\sqrt{4\pi\bar{t}}} e^{-\bar{z}'^2/4\bar{t}} \right) , \quad (\text{S.121})$$

where  $*$  denotes the convolution over the time domain from 0 to  $\bar{t}$ . The form of this solution follows from observing that  $\frac{e^{-\bar{t}}}{\sqrt{4\pi\bar{t}}} e^{-\bar{z}'^2/4\bar{t}}$  is the Green's function for the charge density equation for a point source in a one-dimensional infinite domain. The factor of 2 accounts for the flux being in only one direction due to the no-flux boundary condition at the membrane interface.

#### 4. The charging dynamics ( $0 < \bar{t} \leq \bar{\tau}^0$ )

The driving function in Eq. (S.108) is given by

$$\bar{f}(\bar{t}) = \bar{j}^0(\bar{t}) + \int_0^{\bar{t}} \bar{j}^0(\bar{\tau}) d\bar{\tau} = \begin{cases} 0 & \bar{t} \leq 0 \\ \bar{j}_0^0(1 + \bar{t}) & 0 < \bar{t} \leq \bar{\tau}^0 \\ \bar{j}_0^0 \bar{\tau}^0 & \bar{t} > \bar{\tau}^0 \end{cases} . \quad (\text{S.122})$$

Thus,  $\bar{f}(\bar{t}) = \bar{j}_0^\circ(1 + \bar{t})$  during the charging period  $0 < \bar{t} \leq \bar{\tau}^\circ$ . From Eq. (S.121), we obtain the analytical solution to the charge density during charging as

$$\begin{aligned}\bar{\rho}(\bar{t}, \bar{z}') &= 2\bar{j}_0^\circ(1 + \bar{t}) * \frac{e^{-\bar{t}}}{\sqrt{4\pi\bar{t}}} e^{-\bar{z}'^2/4\bar{t}} \\ &= \bar{j}_0^\circ \left[ \sqrt{\frac{\bar{t}}{\pi}} e^{-\bar{t}-\bar{z}'^2/4\bar{t}} + \frac{1}{4} e^{-\bar{z}'} (2\bar{t} - \bar{z}' + 1) \operatorname{erfc}\left(\frac{\bar{z}'}{2\sqrt{\bar{t}}} - \sqrt{\bar{t}}\right) - \frac{1}{4} e^{\bar{z}'} (2\bar{t} + \bar{z}' + 1) \operatorname{erfc}\left(\frac{\bar{z}'}{2\sqrt{\bar{t}}} + \sqrt{\bar{t}}\right) \right],\end{aligned}\quad (\text{S.123})$$

for  $0 < \bar{z}' < \infty$ . In the limit of large  $\bar{t} \gg 1$ , the first and third terms in the brackets decay as  $\sqrt{\bar{t}}e^{-\bar{t}}$  while the second term scales linearly with time. Thus, long-time asymptotic behavior is described by

$$\bar{\rho}(\bar{t}, \bar{z}') = \bar{j}_0^\circ \bar{t} e^{-\bar{z}'} \left(1 - \frac{\bar{z}' - 1}{2\bar{t}}\right) + \mathcal{O}\left(\sqrt{\bar{t}}e^{-\bar{t}}\right) \approx \bar{Q}(\bar{t})e^{-\bar{z}'}, \quad (\text{S.124})$$

where we leave only the leading order contribution in the final approximation. Equation (S.124) recovers the form presented in the main text and indicates the formation of a quasi-steady diffuse charge layer.

A quasi-steady state solution for the electric potential can be obtained by using Poisson's equation in domain II (again, dropping the superscripts)

$$-\frac{\partial^2 \bar{\phi}}{\partial \bar{z}'^2} = \bar{\rho}, \quad (\text{S.125})$$

subject to the boundary conditions

$$\frac{\partial \bar{\phi}}{\partial \bar{z}'} = \bar{Q}(\bar{t}), \quad \text{at } \bar{z}' = 0, \quad (\text{S.126})$$

$$\frac{\partial \bar{\phi}}{\partial \bar{z}'} = 0, \quad \text{as } \bar{z}' \rightarrow \infty. \quad (\text{S.127})$$

As both boundary conditions are Neumann, a reference of the potential is required. Here, we set it as infinity, i.e.  $\bar{\phi} \rightarrow 0$  as  $\bar{z}' \rightarrow \infty$ . Substitution of Eq. (S.123) into Eq. (S.125) followed by integration with respect to  $\bar{z}'$  twice yields

$$\begin{aligned}\bar{\phi}(\bar{t}, \bar{z}') &= -\bar{j}_0^\circ \left[ \sqrt{\frac{\bar{t}}{\pi}} e^{-\bar{t}-\bar{z}'^2/4\bar{t}} + \frac{1}{4} e^{-\bar{z}'} (2\bar{t} - \bar{z}' - 1) \operatorname{erfc}\left(\frac{\bar{z}'}{2\sqrt{\bar{t}}} - \sqrt{\bar{t}}\right) \right. \\ &\quad \left. - \frac{1}{4} e^{\bar{z}'} (2\bar{t} + \bar{z}' - 1) \operatorname{erfc}\left(\frac{\bar{z}'}{2\sqrt{\bar{t}}} + \sqrt{\bar{t}}\right) \right],\end{aligned}\quad (\text{S.128})$$

for  $0 < \bar{t} < \bar{\tau}^\circ$ , showing a similar structure as with the charge density in Eq. (S.123). Again, we consider long-time ( $\bar{t} \gg 1$ ) asymptotic behavior:

$$\bar{\phi}(\bar{t}, \bar{z}') = -\bar{j}_0^\circ \bar{t} e^{-\bar{z}'} \left(1 - \frac{\bar{z}' + 1}{2\bar{t}}\right) + \mathcal{O}\left(\sqrt{\bar{t}}e^{-\bar{t}}\right) \approx -\bar{Q}(\bar{t})e^{-\bar{z}'}, \quad (\text{S.129})$$

consistent with the development of a quasi-steady diffuse charge layer.

So far, we have omitted discussion of the excess salt concentration,  $\bar{C}^\alpha$ , since it is decoupled from  $\bar{\phi}^\alpha$  and  $\bar{\rho}^\alpha$  in the linearized equations. For completeness, we provide the solution for salt concentration. The salt concentration in either domain satisfies (dropping the subscript)

$$\frac{\partial \bar{C}}{\partial \bar{t}} = \frac{\partial^2 \bar{C}}{\partial \bar{z}'^2}, \quad (\text{S.130})$$

subject to the boundary conditions

$$\frac{\partial \bar{C}}{\partial \bar{z}'} = -\bar{j}_0^\circ [\Theta(\bar{t}) - \Theta(\bar{t} - \bar{\tau}^\circ)], \quad \text{at } \bar{z}' = 0, \quad (\text{S.131})$$

$$\frac{\partial \bar{C}}{\partial \bar{z}'} = 0, \quad \text{as } \bar{z}' \rightarrow \infty. \quad (\text{S.132})$$

This equation can be solved in multiple ways, e.g. the method of similarity solutions, which gives

$$\bar{C}(\bar{t}, \bar{z}') = 2\bar{j}_0^o \sqrt{\bar{t}} \left[ \frac{1}{\sqrt{\pi}} e^{-\bar{z}'^2/4\bar{t}} - \frac{\bar{z}'}{2\sqrt{\bar{t}}} \operatorname{erfc} \left( \frac{\bar{z}'}{2\sqrt{\bar{t}}} \right) \right], \quad (\text{S.133})$$

for  $0 < \bar{t} < \bar{\tau}^o$ .

## 5. Maximum pumping rate

In what follows, we consider the maximum pumping rate that is attainable for the uniform pumping case. Physically, we must have the dimensional concentrations of the cation and anion be positive for all points in space and time. Recall that

$$\frac{C_+}{C_0} = 1 + \bar{\rho} + \bar{C}, \quad \frac{C_-}{C_0} = 1 - \bar{\rho} + \bar{C}. \quad (\text{S.134})$$

For  $\bar{z} > 0$ , our analytical solutions yield  $\bar{\rho}, \bar{C} > 0$ , and by the oddness of the solution in  $\bar{z}$ , both are negative for  $\bar{z} < 0$ . Therefore, there is a possibility that  $C_+$  will take more extreme values. Moreover, both  $\bar{\rho}$  and  $\bar{C}$  are increasing functions of time and are extremized at the membrane surfaces  $\bar{z} = \pm \bar{\delta}^M/2$ . Therefore, we can conclude that if  $C_+ \geq 0$  at  $\bar{z} = -\bar{\delta}^M/2$  and time  $\bar{\tau}^o$ , then both these fields are everywhere nonnegative, for  $\bar{t} \leq \bar{\tau}^o$ . Thus, the maximum pumping rate that can be achieved for a given  $\bar{\tau}^o$  corresponds to the situation where  $C_+ = 0$  at  $\bar{t} = \bar{\tau}^o$  and  $\bar{z} = -\bar{\delta}^o/2$ . Using the analytical solutions, this condition yields

$$0 = 1 - \bar{j}_{\max}^o \left( \sqrt{\frac{\bar{\tau}^o}{\pi}} e^{-\bar{\tau}^o} + \frac{1}{2} (2\bar{\tau}^o + 1) \operatorname{erf} \left( \sqrt{\bar{\tau}^o} \right) \right) - 2\bar{j}_{\max}^o \sqrt{\frac{\bar{\tau}^o}{\pi}}, \quad (\text{S.135})$$

where  $\bar{j}_{\max}^o$  is the maximum flux. Equation (S.135) can be solved to obtain

$$\bar{j}_{\max}^o = \frac{1}{\sqrt{\frac{\bar{\tau}^o}{\pi}} (2 + e^{-\bar{\tau}^o}) + (\bar{\tau}^o + \frac{1}{2}) \operatorname{erf}(\sqrt{\bar{\tau}^o})}, \quad (\text{S.136})$$

which can be expanded for small  $\bar{\tau}^o$  to yield

$$\bar{j}_{\max}^o = \frac{\sqrt{\pi}}{4} \frac{1}{\sqrt{\bar{\tau}^o}} + \mathcal{O}(\sqrt{\bar{\tau}^o}). \quad (\text{S.137})$$

Expanding the solution for large  $\bar{\tau}^o$  is not appropriate, since, in the limit of large  $\bar{\tau}^o$ , the resulting value of  $\bar{j}_{\max}^o$  gives  $\bar{Q} \sim 1$ , making the perturbation expansion to be invalid. In the limit of large  $\bar{\tau}^o$ , we can only conclude that any  $\bar{j}_0^o$  that satisfies  $\bar{Q} \ll 1$  will satisfy non-negativity of concentrations. Lastly, we note a shortcoming of the linearized theory, wherein the above analysis predicts that achieving  $\bar{Q} > 1$  is not possible for any combination of open time and flux. This is untrue, since a steady-state with non-negative concentrations exists for any value of  $\bar{Q}$ , and for large  $\bar{Q}$ , it simply deviates from the linearized solution.

Equation (S.135) and the above analysis also indicates that for a given pumping rate  $\bar{j}^o$ , there exists a maximum open time at which the concentrations become negative, given by

$$\bar{\tau}_{\max}^o \approx \frac{\pi}{16} \left( \frac{1}{\bar{j}^o} \right)^2. \quad (\text{S.138})$$

## 6. The relaxation dynamics ( $\bar{t} > \bar{\tau}^o$ )

For  $\bar{t} > \bar{\tau}^o$ , the driving function based on Eq. (S.108) can be written as

$$\bar{f}(\bar{t}) = \bar{j}^o \bar{\tau}^o = \bar{j}^o (1 + \bar{t}) - \bar{j}^o (1 + (\bar{t} - \bar{\tau}^o)). \quad (\text{S.139})$$

Recall that for  $t < \bar{\tau}^0$ , the driving function was  $\bar{f}(\bar{t}) = \bar{j}^0(1 + \bar{t})$ . This immediately suggests that the solution for the relaxation dynamics can be written as the difference between two time-shifted solutions for the charging dynamics. Thus,

$$\bar{\rho}_{\text{rlx}}(\bar{t}, \bar{z}') = \bar{\rho}_{\text{chg}}(\bar{t}, \bar{z}') - \bar{\rho}_{\text{chg}}(\bar{t} - \bar{\tau}^0, \bar{z}') , \quad (\text{S.140})$$

$$\bar{\phi}_{\text{rlx}}(\bar{t}, \bar{z}') = \bar{\phi}_{\text{chg}}(\bar{t}, \bar{z}') - \bar{\phi}_{\text{chg}}(\bar{t} - \bar{\tau}^0, \bar{z}') , \quad (\text{S.141})$$

where subscripts “rlx” and “chg”, introduced temporarily for clarity, denote relaxation and charging, respectively. The charging solutions  $\bar{\rho}_{\text{chg}}$  and  $\bar{\phi}_{\text{chg}}$  are obtained from Eqs. (S.123) and (S.128), respectively. As before, we can find the long-time behavior ( $\bar{t} \gg \bar{\tau}^0$ ) relaxation behaviors to be

$$\bar{\rho}(\bar{t}, \bar{z}') = \bar{j}_0^0 \bar{\tau}^0 e^{-\bar{z}'} + \mathcal{O}\left(\sqrt{\bar{t} - \bar{\tau}^0} e^{-(\bar{t} - \bar{\tau}^0)}\right) \approx \bar{Q}(\bar{\tau}^0) e^{-\bar{z}'} , \quad (\text{S.142})$$

$$\bar{\phi}(\bar{t}, \bar{z}') = -\bar{j}_0^0 \bar{\tau}^0 e^{-\bar{z}'} + \mathcal{O}\left(\sqrt{\bar{t} - \bar{\tau}^0} e^{-(\bar{t} - \bar{\tau}^0)}\right) \approx -\bar{Q}(\bar{\tau}^0) e^{-\bar{z}'} , \quad (\text{S.143})$$

with  $\bar{Q}(\bar{\tau}^0) = \bar{j}_0^0 \bar{\tau}^0$  being the total pumped charge. The dynamics of both the charge density and electric potential reach the steady state on time scales  $\mathcal{O}(\tau_D)$  once pumping is deactivated.

Finally, the excess salt concentration can also be derived in the same manner as

$$\begin{aligned} \bar{C}(\bar{t}, \bar{z}') = 2\bar{j}_0^0 \sqrt{\bar{t}} \left[ \frac{1}{\sqrt{\pi}} e^{-\bar{z}'^2/4\bar{t}} - \frac{\bar{z}'}{2\sqrt{\bar{t}}} \text{erfc}\left(\frac{\bar{z}'}{2\sqrt{\bar{t}}}\right) \right] \\ - 2\bar{j}_0^0 \sqrt{\bar{t} - \bar{\tau}^0} \left[ \frac{1}{\sqrt{\pi}} e^{-\bar{z}'^2/4(\bar{t} - \bar{\tau}^0)} - \frac{\bar{z}'}{2\sqrt{\bar{t} - \bar{\tau}^0}} \text{erfc}\left(\frac{\bar{z}'}{2\sqrt{\bar{t} - \bar{\tau}^0}}\right) \right] , \end{aligned} \quad (\text{S.144})$$

For long times  $\bar{t}/\bar{\tau}^0 \gg 1$ , a Taylor series expansion yields

$$\bar{C}(\bar{t}, \bar{z}') = \frac{\bar{j}_0^0 \bar{\tau}^0}{\sqrt{\pi \bar{t}}} e^{-\bar{z}'^2/4\bar{t}} + \mathcal{O}\left(\left(\frac{\bar{\tau}^0}{\bar{t}}\right)^2\right) , \quad (\text{S.145})$$

which is the solution corresponding to the diffusive spreading of a point source. Due to the self-similar nature of the dynamics, the relaxation of the salt concentration is much slower than that of the charge density and electric potential. Comparison of the higher order terms suggests that the salt concentration relaxes to the self-similar solution on time scales of  $\mathcal{O}(\bar{\tau}^0)$ , while the charge density and electric potential relax to their steady-state solutions on time scales of  $\mathcal{O}(1)$ .

## IV. Spatially localized pumping

We now derive the theory underlying the spatiotemporal scaling behaviors that emerge in the localized pumping problem presented in Sec. IV of the main text. Results from the FEM simulations of the full PNP equations (Fig. 7, main text) indicate that the maximum value of the potential is  $\bar{\phi} \sim 0.1 \ll 1$ . Accordingly, our derivations are based on the linearized equations and boundary conditions presented in Eqs. (S.86)-(S.93), rather than the full nonlinear equations.

### 1. Point charge approximation

#### (a). Derivation of exact solution

In the point charge (pc) approximation, we assume that the pumped cationic charge is a point charge located at a distance  $\bar{d}$  from the  $\bar{z} = 0$  axis near the membrane surface  $\bar{S}^{\text{II}}$ . The corresponding anionic charge is located at a similar distance  $\bar{d}$  near the opposite surface  $\bar{S}^{\text{I}}$ , with  $0 < \bar{d} - \bar{\delta}^{\text{M}}/2 \ll 1$  (Figs. S5a,b). We also treat the electrolyte solutions as perfect dielectrics, with the membrane providing a dielectric discontinuity in the system. This results in an electrostatics problem with charge density given by

$$\bar{\rho}^{\text{pc}}(\bar{r}, \bar{z}, \bar{t}) = \frac{\bar{\delta}(\bar{r})}{2\pi\bar{r}} [\bar{\delta}(\bar{z} - \bar{d}) - \bar{\delta}(\bar{z} + \bar{d})] \bar{q}(\bar{t}) , \quad (\text{S.146})$$

where  $\bar{q}(\bar{t}) = \pi (\bar{R}^P)^2 \bar{j}_0^o \bar{t}$ , as noted in the main text. The corresponding electric potential satisfies Poisson's equation

$$\bar{\nabla}^2 \bar{\phi}^{\text{pc}} = -\frac{\bar{\delta}(\bar{r})}{2\pi\bar{r}} [\bar{\delta}(\bar{z} - \bar{d}) - \bar{\delta}(\bar{z} + \bar{d})] \bar{q}(\bar{t}) , \quad (\text{S.147})$$

subject to the boundary conditions

$$\bar{\phi}^\alpha = \bar{\phi}^{\text{M}} \quad \text{and} \quad \frac{\partial \bar{\phi}^\alpha}{\partial \bar{z}} = \frac{1}{\bar{\Gamma}} \frac{\partial \bar{\phi}^{\text{M}}}{\partial \bar{z}} \quad \text{on} \quad \bar{S}^\alpha , \quad (\text{S.148})$$

where  $\alpha \in \{\text{I}, \text{II}\}$ . It is implicit that  $\bar{\phi}^{\text{I}}$ ,  $\bar{\phi}^{\text{M}}$  and  $\bar{\phi}^{\text{II}}$  refer to a single continuous field  $\bar{\phi}^{\text{pc}}$  spanning the domains  $\bar{\Omega}^{\text{I}}$ ,  $\bar{\Omega}^{\text{M}}$  and  $\bar{\Omega}^{\text{II}}$ .

We introduce the Hankel transform

$$\hat{f}(\hat{k}) = \mathcal{H}[\bar{f}(\bar{r})](\hat{k}) = \int_0^\infty \bar{f}(\bar{r}) \bar{r} J_0(\bar{r}\hat{k}) d\bar{r} , \quad (\text{S.149})$$

where  $\bar{f}(\bar{r})$  is any function of the radial coordinate  $\bar{r}$  and  $J_\nu(\cdot)$  denotes the Bessel function of the first kind of order  $\nu$  [1]. We call  $\hat{f}(\hat{k})$  the Hankel transform of  $\bar{f}(\bar{r})$ , where  $\hat{k}$  is the wave number. The Hankel transform satisfies the property that its inverse is also the Hankel transform, namely

$$\bar{f}(\bar{r}) = \mathcal{H}^{-1}[\hat{f}(\hat{k})](\bar{r}) = \int_0^\infty \hat{f}(\hat{k}) \hat{k} J_0(\bar{r}\hat{k}) d\hat{k} . \quad (\text{S.150})$$

In what follows we will apply the Hankel transform to functions that may have other dependencies, such as in  $\bar{z}$  and  $\bar{t}$ , but the transform will have no effect on these variables.

The Hankel transform converts the radial Laplacian operator into a multiplicative factor

$$\mathcal{H} \left[ \frac{1}{\bar{r}} \left( \frac{\partial}{\partial \bar{r}} \left( \bar{r} \frac{\partial \bar{f}}{\partial \bar{r}} \right) \right) \right] (\hat{k}) = -\hat{k}^2 \mathcal{H}[\bar{f}(\bar{r})](\hat{k}) = -\hat{k}^2 \hat{f}(\hat{k}) . \quad (\text{S.151})$$

It is also easy to see that  $\mathcal{H}[\bar{\delta}(\bar{r})/2\pi\bar{r}] = 1/2\pi$ . Thus, taking the Hankel transform of Eq. (S.147), and dropping the superscript “pc” for the remainder of this section, we get

$$-\hat{k}^2 \hat{\phi} + \frac{\partial^2 \hat{\phi}}{\partial \bar{z}^2} = -\frac{\bar{q}}{2\pi} [\bar{\delta}(\bar{z} - \bar{d}) - \bar{\delta}(\bar{z} + \bar{d})] , \quad (\text{S.152})$$

with the boundary conditions (S.148) transforming as

$$\hat{\phi}^\alpha = \hat{\phi}^{\text{M}} \quad \text{and} \quad \frac{\partial \hat{\phi}^\alpha}{\partial \bar{z}} = \frac{1}{\bar{\Gamma}} \frac{\partial \hat{\phi}^{\text{M}}}{\partial \bar{z}} \quad \text{on} \quad \bar{S}^\alpha , \quad (\text{S.153})$$

for  $\alpha \in \{\text{I}, \text{II}\}$ .

Due to the nature of the pumping, the charge density is odd in  $\bar{z}$  so that  $\bar{\rho}(\bar{r}, -\bar{z}, t) = -\bar{\rho}(\bar{r}, \bar{z}, t)$ . This, combined with the linearity of Poisson's equation and the boundary conditions above, results in both  $\bar{\phi}$  and  $\hat{\phi}$  also being odd with respect to  $\bar{z}$ . We can therefore solve only on the domain  $\bar{z} \geq 0$  and use the symmetry condition  $\hat{\phi}(\bar{z} = 0) = 0$  to obtain the solution for  $\bar{z} \leq 0$ . For ease of notation, let us define  $\bar{h} = \bar{\delta}^{\text{M}}/2$ . Considering the different subdomains for  $\bar{z} \geq 0$  (Fig. S5), we then have

$$-\hat{k}^2 \hat{\phi}^{\text{M}} + \frac{\partial^2 \hat{\phi}^{\text{M}}}{\partial \bar{z}^2} = 0 , \quad 0 \leq \bar{z} < \bar{h} , \quad (\text{S.154})$$

$$-\hat{k}^2 \hat{\phi}^{\text{II}} + \frac{\partial^2 \hat{\phi}^{\text{II}}}{\partial \bar{z}^2} = 0 , \quad \bar{h} \leq \bar{z} < \bar{d} , \quad (\text{S.155})$$

$$-\hat{k}^2 \hat{\phi}^{\text{II}} + \frac{\partial^2 \hat{\phi}^{\text{II}}}{\partial \bar{z}^2} = 0 , \quad \bar{z} \geq \bar{d} , \quad (\text{S.156})$$

subject to the boundary conditions

$$\hat{\phi}^{\text{M}} \Big|_{\bar{z}=0} = 0 , \quad (\text{S.157})$$

$$\hat{\phi}^{\text{M}} \Big|_{\bar{z}=\bar{h}^-} = \hat{\phi}^{\text{II}} \Big|_{\bar{z}=\bar{h}^+} , \quad \frac{1}{\bar{\Gamma}} \frac{\partial \hat{\phi}^{\text{M}}}{\partial \bar{z}} \Big|_{\bar{z}=\bar{h}^-} = \frac{\partial \hat{\phi}^{\text{II}}}{\partial \bar{z}} \Big|_{\bar{z}=\bar{h}^+} , \quad (\text{S.158})$$

$$\hat{\phi}^{\text{II}} \Big|_{\bar{z}=\bar{d}^-} = \hat{\phi}^{\text{II}} \Big|_{\bar{z}=\bar{d}^+} , \quad \frac{\partial \hat{\phi}^{\text{II}}}{\partial \bar{z}} \Big|_{\bar{z}=\bar{d}^-} = \frac{\partial \hat{\phi}^{\text{II}}}{\partial \bar{z}} \Big|_{\bar{z}=\bar{d}^+} + \frac{\bar{q}}{2\pi} , \quad (\text{S.159})$$

$$\lim_{\bar{z} \rightarrow \infty} \hat{\phi}^{\text{II}} = 0 , \quad (\text{S.160})$$

where the boundary conditions at  $\bar{z} = \bar{d}$  arise from integrating Gauss's law in an axisymmetric pillbox around  $\bar{z} = \bar{d}$ , and enforcing the continuity of  $\hat{\phi}^{\text{II}}$ , respectively.

Solving the system of equations (S.156)-(S.160) yields the following solution for the potential in the transformed space

$$\hat{\phi}(\hat{k}, \bar{z}) = \bar{q} \frac{e^{-\hat{k}(\bar{d}-\bar{h})}}{2\pi\hat{k}} \begin{cases} \frac{\bar{\Gamma} \tanh(\hat{k}\bar{h})}{1 + \bar{\Gamma} \tanh(\hat{k}\bar{h})} \frac{\sinh(\hat{k}\bar{z})}{\sinh(\hat{k}\bar{h})} , & 0 \leq \bar{z} < \bar{h} , \\ \frac{\sinh(\hat{k}(\bar{z} - \bar{h})) + \bar{\Gamma} \tanh(\hat{k}\bar{h}) \cosh(\hat{k}(\bar{z} - \bar{h}))}{1 + \bar{\Gamma} \tanh(\hat{k}\bar{h})} , & \bar{h} \leq \bar{z} < \bar{d} , \\ \frac{\sinh(\hat{k}(\bar{d} - \bar{h})) + \bar{\Gamma} \tanh(\hat{k}\bar{h}) \cosh(\hat{k}(\bar{d} - \bar{h}))}{1 + \bar{\Gamma} \tanh(\hat{k}\bar{h})} e^{-\hat{k}(\bar{z}-\bar{d})} , & \bar{z} \geq \bar{d} . \end{cases} \quad (\text{S.161})$$

### (b). Image charge representation

We can expand the hyperbolic functions in Eq. (S.161) to explain the potential in terms of image charges. As a representative example, we consider the subdomain  $\bar{h} \leq \bar{z} < \bar{d}$  (i.e. close to the membrane surface), which, after some algebraic manipulations, yields

$$\hat{\phi}^{\text{II}} = \bar{q} \frac{e^{-\hat{k}(\bar{d}-\bar{h})}}{4\pi\hat{k}} \cdot \frac{\left(e^{\hat{k}(\bar{z}-\bar{h})} - e^{-\hat{k}(\bar{z}-\bar{h})}\right) \left(e^{\hat{k}\bar{h}} + e^{-\hat{k}\bar{h}}\right) + \bar{\Gamma} \left(e^{\hat{k}(\bar{z}-\bar{h})} + e^{-\hat{k}(\bar{z}-\bar{h})}\right) \left(e^{\hat{k}\bar{h}} - e^{-\hat{k}\bar{h}}\right)}{\left(e^{\hat{k}\bar{h}} + e^{-\hat{k}\bar{h}}\right) + \bar{\Gamma} \left(e^{\hat{k}\bar{h}} - e^{-\hat{k}\bar{h}}\right)} , \quad (\text{S.162})$$

$$= \frac{\bar{q}}{4\pi\hat{k}} \cdot \frac{e^{-\hat{k}(\bar{d}-\bar{z})} - \frac{\bar{\Gamma}-1}{\bar{\Gamma}+1} e^{-\hat{k}(\bar{d}-\bar{z}+2\bar{h})} - e^{-\hat{k}(\bar{d}+\bar{z})} + \frac{\bar{\Gamma}-1}{\bar{\Gamma}+1} e^{-\hat{k}(\bar{d}+\bar{z}-2\bar{h})}}{1 - \frac{\bar{\Gamma}-1}{\bar{\Gamma}+1} e^{-2\hat{k}\bar{h}}} . \quad (\text{S.163})$$

The denominator can be expanded as a geometric series, giving

$$\hat{\phi}^{\text{II}} = \frac{\bar{q}}{4\pi\hat{k}} \left( e^{-\hat{k}(\bar{d}-\bar{z})} - \frac{\bar{\Gamma}-1}{\bar{\Gamma}+1} e^{-\hat{k}(\bar{d}-\bar{z}+2\bar{h})} - e^{-\hat{k}(\bar{d}+\bar{z})} + \frac{\bar{\Gamma}-1}{\bar{\Gamma}+1} e^{-\hat{k}(\bar{d}+\bar{z}-2\bar{h})} \right) \sum_{i=0}^{\infty} \left( \frac{\bar{\Gamma}-1}{\bar{\Gamma}+1} \right)^i e^{-2\hat{k}\bar{h}i} . \quad (\text{S.164})$$

Next, we distribute the series term on the RHS over the terms inside the parentheses. Doing so, we find that the first two series telescope, giving

$$\hat{\phi}^{\text{II}} = \frac{\bar{q}}{4\pi\hat{k}} \left( e^{-\hat{k}(\bar{d}-\bar{z})} + \frac{\bar{\Gamma}-1}{\bar{\Gamma}+1} e^{-\hat{k}(\bar{z}-(2\bar{h}-\bar{d}))} - \frac{4\bar{\Gamma}}{(\bar{\Gamma}+1)^2} \sum_{i=0}^{\infty} \left( \frac{\bar{\Gamma}-1}{\bar{\Gamma}+1} \right)^i e^{-\hat{k}(\bar{z}-(-\bar{d}-2\bar{h}i))} \right) . \quad (\text{S.165})$$

Now, the Hankel transform of the potential of a point charge  $\bar{q}$  located at  $\bar{r} = 0$  and  $\bar{z} = \bar{z}_0$  is  $e^{-\hat{k}|\bar{z}-\bar{z}_0|}/4\pi\hat{k}$ . Therefore, it is immediately clear that Eq. (S.165) is the Hankel transformed potential in domain II due to an infinite number of charges at different locations (Fig. S5(c)). The charges include: a positive point charge of magnitude  $\bar{q}$  located at  $\bar{z} = \bar{d}$  (the original pumped charge), a positive image charge of magnitude  $\bar{q}(\bar{\Gamma}-1)/(\bar{\Gamma}+1)$  located at  $\bar{z} = 2\bar{h} - \bar{d}$  (the image of the former charge reflected across  $\bar{S}^{\text{II}}$ ), and an infinite series of negative image charges, with the first being  $-4\bar{q}\bar{\Gamma}/(\bar{\Gamma}+1)^2$  located at  $\bar{z} = -\bar{d}$  (the true location of the negative pumped charge). The remaining negative image charges are placed in steps of  $2\bar{h}$  away in the  $-\bar{z}$  direction, with the magnitude decreasing by a factor of  $(\bar{\Gamma}-1)/(\bar{\Gamma}+1) < 1$  for

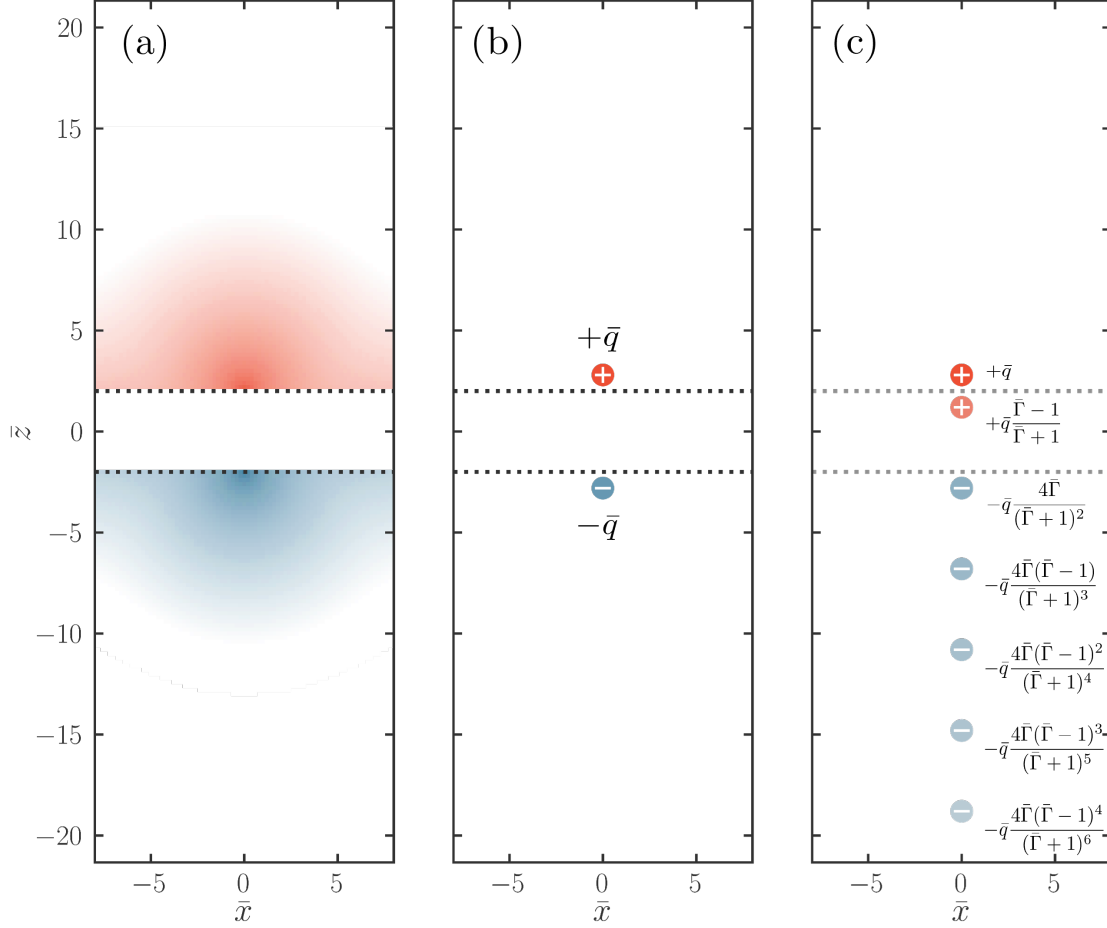

Figure S5: Image charge representation for the electrostatic potential in domain II based on the point charge approximation. (a) heatmap of the charge density fields, (b) the point charge approximation, (c) the image charge picture based on Eq. (S.166). The negative charge in domain I becomes an infinite series of negative charges and the positive charge in domain II has an image reflected across the membrane due to the dielectric mismatch.

each subsequent charge. Note that the total magnitude of all the negative charges is  $2\bar{\Gamma}/(\bar{\Gamma} + 1)$ , which, as expected, is equal to the sum of the two positive charges, given that our system is globally electroneutral. Inverting to real space we find

$$\bar{\phi}^{\text{pc},\text{II}}(\bar{r}, \bar{z}) = \frac{1}{4\pi} \left( \frac{\bar{q}}{\sqrt{\bar{r}^2 + (\bar{z} - \bar{d})^2}} + \frac{\bar{q} \left( \frac{\bar{\Gamma} - 1}{\bar{\Gamma} + 1} \right)}{\sqrt{\bar{r}^2 + (\bar{z} - (2\bar{h} - \bar{d}))^2}} - \sum_{i=0}^{\infty} \frac{\bar{q} \frac{4\bar{\Gamma}}{(\bar{\Gamma} + 1)^2} \left( \frac{\bar{\Gamma} - 1}{\bar{\Gamma} + 1} \right)^i}{\sqrt{\bar{r}^2 + (\bar{z} - (-\bar{d} - 2\bar{h}i))^2}} \right), \quad (\text{S.166})$$

for the potential in domain II for  $\bar{h} < \bar{z} < \bar{d}$ . Incidentally, it is easy to show that the same solution arises for the subdomain  $\bar{z} > \bar{d}$ .

### (c). Multipole expansion and asymptotic limits

We now obtain asymptotic expressions for the solution (S.166) considering the limits when the point  $\bar{\mathbf{x}} = (\bar{r}, \bar{z})$  is either far from or close to the pump patch, respectively. Throughout, we will assume that  $\bar{\Gamma} \gg 1$  as is the case in biological settings, and that the point charges are very close to the membrane surfaces, i.e.  $\bar{d} \approx \bar{\delta}^{\text{M}}/2$ . This is reasonable since the numerical solutions show that the “charge dome” is localized near the surface of the membrane.

We begin with the large distance limit by considering the multipole expansion of the potential [7]. Since all image charges are located on the  $\bar{z}$ -axis (i.e.  $\bar{r} = 0$ ), we center the expansion about the point  $(\bar{r}, \bar{z}) = (0, \bar{z}_0)$ , for some point  $\bar{z}_0$ , which shall be determined shortly. The terms of the multipole expansion upto quadrupole order are

$$\bar{\phi}^{\text{pc}, \text{II}}(\bar{r}, \bar{z}) = \frac{1}{4\pi} \left[ \frac{\bar{q}_{\text{tot}}}{(\bar{r}^2 + (\bar{z} - \bar{z}_0)^2)^{1/2}} + \frac{\bar{p}(\bar{z} - \bar{z}_0)}{(\bar{r}^2 + (\bar{z} - \bar{z}_0)^2)^{3/2}} + \frac{1}{2} \frac{\bar{Q} [2(\bar{z} - \bar{z}_0)^2 - \bar{r}^2]}{(\bar{r}^2 + (\bar{z} - \bar{z}_0)^2)^{5/2}} + \dots \right], \quad (\text{S.167})$$

where

$$\bar{q}_{\text{tot}} = \sum_i \bar{q}_i \text{ is the total charge,} \quad (\text{S.168})$$

$$\bar{p} = \sum_i \bar{q}_i (\bar{z}_i - \bar{z}_0) \text{ is the dipole moment,} \quad (\text{S.169})$$

$$\bar{Q} = \sum_i \bar{q}_i (\bar{z}_i - \bar{z}_0)^2 \text{ is the quadrupole moment.} \quad (\text{S.170})$$

Here  $\bar{q}_i$  is the  $i^{\text{th}}$  charge, and  $\bar{z}_i$  is its  $\bar{z}$ -position. Equation (S.166) gives the magnitudes and positions of all the charges in the system, including the image charges. Since the system is globally electroneutral, we find that  $\bar{q}_{\text{tot}} = 0$ , and the monopolar term vanishes. Thus, the leading order term in the multipole expansion is the dipolar term

$$\bar{p} = \sum_i \bar{q}_i \bar{z}_i - \bar{z}_0 \sum_i \bar{q}_i = \sum_i \bar{q}_i \bar{z}_i, \quad (\text{S.171})$$

which is independent of  $\bar{z}_0$ . Then, the quadrupole moment is related to the dipole moment as

$$\bar{Q} = \sum_i \bar{q}_i \bar{z}_i^2 - 2\bar{z}_0 \sum_i \bar{q}_i \bar{z}_i + \bar{z}_0^2 \sum_i \bar{q}_i = \sum_i \bar{q}_i \bar{z}_i^2 - 2\bar{z}_0 \bar{p}. \quad (\text{S.172})$$

Now, we choose  $\bar{z}_0$  such that the quadrupole term  $\bar{Q} = 0$ , and approximate the multipole expansion using the dipolar term. In this way, approximation error will be restricted to the octopole and higher terms, and  $\bar{z}_0$  can be estimated as

$$\bar{z}_0 = \frac{1}{2} \frac{\sum_i \bar{q}_i \bar{z}_i^2}{\sum_i \bar{q}_i \bar{z}_i}. \quad (\text{S.173})$$

Next, we compute  $\bar{p}$  and  $\bar{z}_0$  by substituting the values of  $\bar{q}_i$  and  $\bar{z}_i$  from Eq. (S.166) into Eqs. (S.171) and (S.173), which yields

$$\bar{p} = \bar{q} ((\bar{\Gamma} - 1)\bar{\delta}^{\text{M}} + 2\bar{d}) \approx \bar{q}\bar{\Gamma}\bar{\delta}^{\text{M}}, \quad (\text{S.174})$$

$$\bar{z}_0 = -\frac{1}{2}(\bar{\Gamma} - 1)\bar{\delta}^{\text{M}}, \quad (\text{S.175})$$

where we have used  $\bar{d} \approx \bar{\delta}^{\text{M}}/2$ . Substituting these expressions into the multipole expansion Eq. (S.167) we find

$$\bar{\phi}^{\text{pc}, \text{II}} = \frac{\bar{q}\bar{\Gamma}\bar{\delta}^{\text{M}}(\bar{z}' + \frac{1}{2}\bar{\Gamma}\bar{\delta}^{\text{M}})}{4\pi (\bar{r}^2 + (\bar{z}' + \frac{1}{2}\bar{\Gamma}\bar{\delta}^{\text{M}})^2)^{3/2}} + \mathcal{O} \left( \bar{r}^2 + (\bar{z}' + \frac{1}{2}\bar{\Gamma}\bar{\delta}^{\text{M}})^2 \right)^{-7/2}, \quad (\text{S.176})$$

where we have introduced  $\bar{z}' \equiv \bar{z} - \bar{\delta}^{\text{M}}/2$ . The error term on the RHS includes the octopole and higher terms.

We now use the multipole expansion to derive asymptotic expressions for the electric potential under the point charge approximation. We do so by identifying the locations where the dipolar term in Eq. (S.176) serves as a good approximation for the potential, with the higher order terms being negligible. Now, it's clear from the calculation above that  $\bar{z}_0$  is the center of this effective dipole. The positive charge  $\bar{q}$  is located at  $\bar{z}_+ = \bar{\delta}^{\text{M}}/2$ , and so the corresponding negative charge  $-\bar{q}$  is located at the mirror position relative to  $\bar{z}_0$ , i.e. at  $\bar{z}_- = -\bar{\delta}^{\text{M}}/2 - 2\bar{z}_0$ . Thus, the separation of the charges in the dipole is  $\bar{z}_+ - \bar{z}_- = \bar{\Gamma}\bar{\delta}^{\text{M}}$  (using Eq. (S.175)). Now, we use the fact that a dipolar approximation is more accurate in locations where the

distance to the nearest charge, which in domain II is the positive charge  $\bar{q}$ , is much greater than the dipole separation, yielding

$$\sqrt{\bar{r}^2 + \bar{z}'^2} \gg \bar{\Gamma} \bar{\delta}^M, \quad (\text{S.177})$$

as the condition for the approximation Eq. (S.176) to hold. Note that  $\bar{r}' = \sqrt{\bar{r}^2 + \bar{z}'^2}$  is the distance from a point  $(\bar{r}, \bar{z})$  to the point  $(0, \bar{\delta}^M/2)$  on the membrane surface.

We now consider the opposite limit  $\sqrt{\bar{r}^2 + \bar{z}'^2} \ll \bar{\Gamma} \bar{\delta}^M$ . In this limit, based on Eq. (S.166), the distances to the positive charge and its image are much less than the distance to the position of the negative image charges. To leading order, we can therefore consider only the monopolar contributions of the two positive charges, yielding

$$\bar{\phi}^{\text{pc,II}}(\bar{r}, \bar{z}) = \frac{2\bar{\Gamma}}{1 + \bar{\Gamma}} \frac{\bar{q}}{4\pi\sqrt{\bar{r}^2 + \bar{z}'^2}}, \quad (\text{S.178})$$

where we have assumed  $\bar{d} \approx \bar{h} = \bar{\delta}^M/2$ . Taken together, this yields asymptotic expressions for the potential in the point charge approximation

$$\bar{\phi}^{\text{pc,II}}(\bar{r}, \bar{z}) = \begin{cases} \frac{2\bar{\Gamma}}{1 + \bar{\Gamma}} \frac{\bar{q}}{4\pi\sqrt{\bar{r}^2 + \bar{z}'^2}} & \sqrt{\bar{r}^2 + \bar{z}'^2} \ll \bar{\Gamma} \bar{\delta}^M, \\ \frac{\bar{\Gamma} \bar{\delta}^M \bar{q}(\bar{z}' + \frac{1}{2}\bar{\Gamma} \bar{\delta}^M)}{4\pi(\bar{r}^2 + (\bar{z}' + \frac{1}{2}\bar{\Gamma} \bar{\delta}^M)^2)^{3/2}} & \sqrt{\bar{r}^2 + \bar{z}'^2} \gg \bar{\Gamma} \bar{\delta}^M, \end{cases} \quad (\text{S.179})$$

with a transition region for  $\sqrt{\bar{r}^2 + \bar{z}'^2} \sim \bar{\Gamma} \bar{\delta}^M$ . This form indicates that in the region  $\sqrt{\bar{r}^2 + \bar{z}'^2} \ll \bar{\Gamma} \bar{\delta}^M$ , the potential will be that of a charge monopole of magnitude  $2\bar{q}\bar{\Gamma}/(1 + \bar{\Gamma})$  located at the source of flux. Conversely, for  $\sqrt{\bar{r}^2 + \bar{z}'^2} \gg \bar{\Gamma} \bar{\delta}^M$  the potential will be that of a charge dipole centered at  $\bar{z} = -(\bar{\Gamma} - 1)\bar{\delta}^M/2$  with dipole moment  $\bar{\Gamma} \bar{\delta}^M \bar{q}$ .

#### (d). Solution for charge density at early times

Next, we leverage the point charge approximation to understand the reorganization of charge density at early times. Far from the channel, it is reasonable to assume that the diffusion of the pumped charge near the transporter will not matter, and that the local reorganization is due solely to long-ranged electric fields induced by pumping. Since the point charge approximation for the potential shows good agreement with the numerical FEM at early times (Fig. 8, main text), we will also use this approximate picture to understand the evolution of charge density profiles. Let us suppose that at early times, the potential is given by

$$\bar{\phi}^{\text{II}}(\bar{r}, \bar{z}, \bar{t}) = \bar{\phi}^{\text{pc,II}}(\bar{r}, \bar{z}) + \bar{\phi}^*(\bar{r}, \bar{z}, \bar{t}), \quad (\text{S.180})$$

where  $\bar{\phi}^{\text{pc,II}}$  is from the point-charge approximation given by Eq. (S.166) and  $\bar{\phi}^*$  is the field due to reorganization. This decomposition is exact, since we simply define  $\bar{\phi}^*$  as the difference between the true electric potential and that due to the point charge approximation.

Let us consider the behavior of the charge density for  $\bar{r} \gg 1$  at early times. Assuming linearity, the governing equation for the charge density is

$$\frac{\partial \bar{\rho}^{\text{II}}}{\partial \bar{t}} = \bar{\nabla}^2 \bar{\rho}^{\text{II}} - \bar{\rho}^{\text{II}}, \quad (\text{S.181})$$

subject to the boundary condition (S.92)

$$\frac{\partial \bar{\rho}^{\text{II}}}{\partial \bar{z}} + \frac{\partial \bar{\phi}^{\text{II}}}{\partial \bar{z}} = 0, \quad (\text{S.182})$$

at  $\bar{z} = \bar{\delta}^M/2$ . Using our representation of the electric potential in Eq. (S.180), we can write

$$\frac{\partial \bar{\rho}^{\text{II}}}{\partial \bar{z}} + \frac{\partial \bar{\phi}^{\text{pc,II}}}{\partial \bar{z}} + \frac{\partial \bar{\phi}^*}{\partial \bar{z}} = 0. \quad (\text{S.183})$$

For sufficiently early times  $\bar{t} \lesssim 1$  we expect that the dominant contribution will be the electrostatic one, as the charge density will not yet have reorganized. This motivates our approximation

$$\frac{\partial \bar{\rho}^{\text{II}}}{\partial \bar{z}} \approx -\frac{\partial \bar{\phi}^{\text{pc,II}}}{\partial \bar{z}}, \quad (\text{S.184})$$

at  $\bar{z} = \bar{\delta}^{\text{M}}/2$ . Next, we write the Laplacian of  $\bar{\rho}^{\text{II}}$  in Eq. (S.181)

$$\bar{\nabla}^2 \bar{\rho}^{\text{II}} = \frac{1}{\bar{r}} \frac{\partial}{\partial \bar{r}} \left( \bar{r} \frac{\partial \bar{\rho}^{\text{II}}}{\partial \bar{r}} \right) + \frac{\partial^2 \bar{\rho}^{\text{II}}}{\partial \bar{z}^2}. \quad (\text{S.185})$$

In the above equation, the radial and the axial terms will scale as  $\bar{\rho}^{\text{II}}/\bar{l}_r^2$  and  $\bar{\rho}^{\text{II}}/\bar{l}_z^2$ , where  $\bar{l}_r$  and  $\bar{l}_z$  are radial and axial length scales over which the field varies. From the uniform transport problem (Sec. III), we expect  $\bar{l}_z \sim 1$ , corresponding to the dimensionless Debye length. Since the charge density in this approximation is related to  $\bar{\phi}^{\text{pc,II}}$  at the surface using Poisson's equation, we expect  $\bar{\rho}^{\text{II}}$  to vary at the surface in  $\bar{r}$  the same way that  $\bar{\phi}^{\text{pc,II}}$  does. As  $\bar{\phi}^{\text{pc,II}}$  varies as a power law based on the previous section,  $\bar{l}_r \sim \bar{r}$ . Since we are considering  $\bar{r} \gg 1$ , this suggests that we can ignore the radial contribution to the Laplacian in Eq. (S.185), with the axial component dominating. Thus, we can write Eq. (S.181) as

$$\frac{\partial \bar{\rho}^{\text{II}}}{\partial \bar{t}} = \frac{\partial^2 \bar{\rho}^{\text{II}}}{\partial \bar{z}^2} - \bar{\rho}^{\text{II}}, \quad (\text{S.186})$$

subject to the boundary condition

$$\frac{\partial \bar{\rho}^{\text{II}}}{\partial \bar{z}} + \frac{\partial \bar{\phi}^{\text{pc,II}}}{\partial \bar{z}} = 0, \quad (\text{S.187})$$

at  $\bar{z} = \bar{\delta}^{\text{M}}/2$ . Note that  $\bar{E}_z^{\text{pc,II}} \equiv -\partial \bar{\phi}^{\text{pc,II}}/\partial \bar{z}$  is the  $\bar{z}$ -component of the electric field in the point charge approximation. Moreover, despite the  $\bar{r}$  dependence of  $\bar{E}_z^{\text{pc,II}}$ , we have no derivatives in  $\bar{r}$  in our equation and boundary condition in the above approximation. Therefore, we can solve the problem as if it were one-dimensional, with radial dependence entering only through  $\bar{E}_z^{\text{pc,II}}$ . This is the quasi-1D analysis mentioned in Sec. IVB of the main text.

In addition, the structure of this problem is equivalent to the problem solved in section III.4, with  $\bar{f}(\bar{t}) = -\bar{E}_z^{\text{pc,II}}$ . By analogy, we can readily write down the solution as

$$\bar{\rho}^{\text{II}}(\bar{r}, \bar{z}, \bar{t}) = -2 \bar{E}_z^{\text{pc,II}}|_{\bar{z}=\bar{\delta}^{\text{M}}/2} * \frac{e^{-\bar{t}}}{\sqrt{4\pi\bar{t}}} e^{-(\bar{z}-\bar{\delta}^{\text{M}}/2)^2/4\bar{t}}, \quad (\text{S.188})$$

where we explicitly note that  $\bar{E}_z^{\text{pc,II}}$  is evaluated on the membrane surface. Note that  $\bar{E}_z^{\text{pc,II}} \propto \bar{q} = \bar{I}\bar{t}$  scales linearly with time. Computing the convolution gives

$$\begin{aligned} \bar{\rho}^{\text{II}}(\bar{r}, \bar{z}, \bar{t}) = & -\frac{\bar{E}_z^{\text{pc,II}}|_{\bar{z}'=0}}{\bar{t}} \cdot \\ & \left( \sqrt{\frac{\bar{t}}{\pi}} e^{-\bar{t}-\bar{z}'^2/4\bar{t}} + \frac{1}{4} e^{-\bar{z}'} (2\bar{t} - \bar{z}' - 1) \operatorname{erfc} \left( \frac{\bar{z}'}{2\sqrt{\bar{t}}} - \sqrt{\bar{t}} \right) - \frac{1}{4} e^{\bar{z}'} (2\bar{t} + \bar{z}' - 1) \operatorname{erfc} \left( \frac{\bar{z}'}{2\sqrt{\bar{t}}} + \sqrt{\bar{t}} \right) \right), \end{aligned} \quad (\text{S.189})$$

for  $\bar{r} \gg 1$  and  $\bar{t} \lesssim 1$ . Near the surface  $\bar{z}' \approx 0$  and we can expand under the limit of  $\bar{t} \ll 1$  obtaining

$$\bar{\rho}^{\text{II}}(\bar{r}, \bar{t}) = -\frac{4}{3} \bar{E}_z^{\text{pc,II}}|_{\bar{z}'=0} \sqrt{\frac{\bar{t}}{\pi}}. \quad (\text{S.190})$$

It is now evident that the charge density on the surface is proportional to the  $\bar{z}$ -component of the local electric field. But because  $\bar{E}_z^{\text{pc,II}}$  scales linearly with  $\bar{t}$ , the charge density grows superlinearly during the early time period. To understand this result further, we can evaluate  $\bar{E}_z^{\text{pc,II}}$  on the surface. By taking the gradient of  $\bar{\phi}^{\text{pc,II}}$  in Eq. (S.166), we find

$$\bar{E}_z^{\text{pc,II}} = \frac{1}{4\pi} \left( \frac{\bar{q}(\bar{z} - \bar{d})}{(\bar{r}^2 + (\bar{z} - \bar{d})^2)^{\frac{3}{2}}} + \frac{\bar{q} \left( \frac{\bar{\Gamma}-1}{\bar{\Gamma}+1} \right) (\bar{z} - (\bar{\delta}^{\text{M}} - \bar{d}))}{(\bar{r}^2 + (\bar{z} - (\bar{\delta}^{\text{M}} - \bar{d}))^2)^{\frac{3}{2}}} - \sum_{i=0}^{\infty} \frac{\bar{q} \frac{4\bar{\Gamma}}{(\bar{\Gamma}+1)^2} \left( \frac{\bar{\Gamma}-1}{\bar{\Gamma}+1} \right)^i (\bar{z} - (-\bar{d} - \bar{\delta}^{\text{M}} i))}{(\bar{r}^2 + (\bar{z} - (-\bar{d} - \bar{\delta}^{\text{M}} i))^2)^{\frac{3}{2}}} \right). \quad (\text{S.191})$$

Substituting  $\bar{z} = \bar{\delta}^M/2$  and  $\bar{d} \approx \bar{\delta}^M/2$ , we see that the two positive charge contributions vanish on the surface, yielding

$$\bar{E}_z^{\text{pc},\text{II}}|_{\bar{z}'=0} = -\frac{1}{4\pi} \sum_{i=0}^{\infty} \frac{\bar{q} \frac{4\bar{\Gamma}}{(\bar{\Gamma}+1)^2} \left(\frac{\bar{\Gamma}-1}{\bar{\Gamma}+1}\right)^i \bar{\delta}^M(i+1)}{(\bar{r}^2 + (\bar{\delta}^M(i+1)))^2}^{\frac{3}{2}}, \quad (\text{S.192})$$

Next, we simplify this expression in the small and large limits of  $\bar{r}$ . First, when  $\bar{r} \ll \bar{\delta}^M$ , we have that  $\bar{r} \ll \bar{\delta}^M(i+1)$  for all  $i \geq 0$ . Therefore,

$$\bar{E}_z^{\text{pc},\text{II}}|_{\bar{z}'=0} \approx -\frac{1}{4\pi} \sum_{i=0}^{\infty} \frac{\bar{q} \frac{4\bar{\Gamma}}{(\bar{\Gamma}+1)^2} \left(\frac{\bar{\Gamma}-1}{\bar{\Gamma}+1}\right)^i}{(\bar{\delta}^M(i+1))^2} = -\frac{1}{4\pi} \frac{\bar{q} \frac{4\bar{\Gamma}}{(\bar{\Gamma}^2-1)} \text{Li}_2\left(\frac{\bar{\Gamma}-1}{\bar{\Gamma}+1}\right)}{(\bar{\delta}^M)^2}, \quad (\text{S.193})$$

where  $\text{Li}_2$  is the polylogarithm [1]. Since  $\bar{\Gamma} \gg 1$ , we have  $(\bar{\Gamma}-1)/(\bar{\Gamma}+1) \rightarrow 1$  and  $\text{Li}_2(1) = \pi^2/6$ , so we can approximate

$$\bar{E}_z^{\text{pc},\text{II}}|_{\bar{z}'=0} \approx -\frac{1}{4\pi} \frac{\bar{q} \frac{4\bar{\Gamma}}{(\bar{\Gamma}^2-1)} \pi^2}{(\bar{\delta}^M)^2}, \quad (\text{S.194})$$

for small  $\bar{r}$ . For  $\bar{r} \gg \bar{\Gamma}\bar{\delta}^M$ , the multipole expansion is valid. Differentiating Eq. (S.176) with respect to  $\bar{z}$ , we get

$$\bar{E}_z^{\text{pc},\text{II}}|_{\bar{z}'=0} = \frac{\bar{\Gamma}\bar{\delta}^M\bar{q}}{4\pi(\bar{r}^2 + (\bar{z}' + \frac{1}{2}\bar{\Gamma}\bar{\delta}^M)^2)^{3/2}}, \quad (\text{S.195})$$

where we have neglected the  $1/\bar{r}^5$  term since  $\bar{r} \gg 1$ . Taken together, the asymptotic forms for the electric field are

$$\bar{E}_z^{\text{pc},\text{II}}|_{\bar{z}'=0} = \begin{cases} -\frac{1}{4\pi} \frac{4\bar{\Gamma}}{\bar{\Gamma}^2-1} \frac{\bar{q}(\bar{t})}{(\bar{\delta}^M)^2} \frac{\pi^2}{6} & \bar{r} \ll \bar{\delta}^M, \\ -\frac{1}{4\pi} \frac{\bar{\Gamma}\bar{\delta}^M\bar{q}(\bar{t})}{(\bar{r}^2 + (\frac{1}{2}\bar{\Gamma}\bar{\delta}^M)^2)^{3/2}} & \bar{r} \gg \bar{\Gamma}\bar{\delta}^M, \end{cases}, \quad (\text{S.196})$$

where we now have a transition region  $\bar{\delta}^M \lesssim \bar{r} \lesssim \bar{\Gamma}\bar{\delta}^M$  between the two scaling regions. Over these length scales, there is a complex dependence on the negative image charges. For  $\bar{r} \ll \bar{\delta}^M$ , the point charge approximation predicts a constant electric field and for  $\bar{r} \gg \bar{\Gamma}\bar{\delta}^M$ , it predicts a  $1/\bar{r}^3$  (dipolar) electric field.

Our simulations (Fig. 8, main text) suggest that the point charge approximation is relatively robust for  $\bar{r} \gtrsim 1$  and small  $\bar{t}$ . The approximation breaks down for small  $\bar{r}$  for two reasons. First, the diffusive spreading of the pumped charge contributes significantly to the profile. Second, the radial portion of the Laplacian cannot be neglected, since  $\bar{l}_r$  is comparable to  $\bar{l}_z$  in this region. The approximation also breaks down for large  $\bar{t}$ , as charges reorganize along the membrane surface and the point charge picture is inaccurate. Over long times, the correction  $\bar{\phi}^*$  in Eq. (S.180) becomes comparable in magnitude with  $\bar{\phi}^{\text{pc}}$ , leading to a contribution to the boundary condition (S.183) that couples all three domains. The next sections address these gaps by building a more comprehensive theory.

## 2. Near-field approximation

This section derives the results presented in section IV.C of the main text.

### (a). Point charge spreading

We begin by considering the diffusive spreading of a point charge source within an electrolyte in a spherically symmetric setting. Suppose we have an infinite electrolyte domain in 3D, where a point charge of magnitude  $\bar{q} \ll 1$  is placed at the origin at  $\bar{t} = 0$ . Thus, the initial condition is  $\bar{\rho}(0) = \bar{q}\bar{\delta}(\bar{r})/(2\pi\bar{r}^2)$  where  $\bar{r}$  is the spherical radial coordinate. We will assume that the charge density and its gradient decay to zero as  $\bar{r} \rightarrow \infty$ .

We will now analyze the spreading of this charge by solving the linearized Eq. (S.181) with this initial condition, noting that the equation breaks down for very early times and short length scales when the  $\delta$  function may be expected to introduce singular behavior. The next section uses the solution to this problem as Green's function, which helps us obtain the near-field dynamics for the spatially localized pumping problem.

The governing equation for the charge density is

$$\frac{\partial \bar{\rho}}{\partial \bar{t}} = \bar{\nabla}^2 \bar{\rho} - \bar{\rho} = \frac{1}{\bar{r}^2} \frac{\partial}{\partial \bar{r}} \left( \bar{r}^2 \frac{\partial \bar{\rho}}{\partial \bar{r}} \right) - \bar{\rho} \quad (\text{S.197})$$

where the first term on the RHS is the radial Laplacian. Using the transformation

$$\bar{\nu} = \bar{\rho} e^{\bar{t}}, \quad (\text{S.198})$$

our governing equation becomes

$$\frac{\partial \bar{\nu}}{\partial \bar{t}} = \bar{\nabla}^2 \bar{\nu}. \quad (\text{S.199})$$

and we have eliminated the decay term, resulting in a simple diffusion equation. The initial condition will be unchanged, since for  $\bar{t} = 0$ ,  $\bar{\nu}(0) = \bar{\rho}(0)$ . Note that this transformation could be applied to the first-order perturbation theory of the PNP equations for any geometry and boundary conditions. However, in many cases, it will be less useful, since the boundary condition for  $\bar{\nu}$  will itself scale exponentially in time.

The solution to Eq. (S.199) is [5]

$$\bar{\nu} = \frac{1}{(4\pi\bar{t})^{3/2}} e^{-\bar{r}^2/4\bar{t}} \quad (\text{S.200})$$

which satisfies the governing equation, boundary conditions, and initial condition. Taking the inverse transform we find that the charge density satisfies

$$\bar{\rho}(\bar{r}, \bar{t}) = \frac{e^{-t}}{(4\pi\bar{t})^{3/2}} e^{-\bar{r}^2/4\bar{t}}. \quad (\text{S.201})$$

This analysis indicates that the spreading of a point charge in an electrolyte in the first-order perturbation theory is like 3D solute diffusion [5], with the multiplication of an exponential-in-time decay.

## (b). Application to channel problem

The solution (S.201) can be utilized to obtain a solution for the near-field, short-time dynamics of the spatially localized pumping problem. This is because, for short times and distances, we expect the pumped charge to spread like a point charge in the electrolyte, with the membrane insulating the pumped cations from the anions on the other side of the membrane, and vice versa. It is easy to see this by recalling the true boundary condition at the interface (Eq. (S.69))

$$\frac{\partial \bar{\phi}^\alpha}{\partial \bar{z}} = \frac{1}{\bar{\Gamma}} \frac{\partial \bar{\phi}^\text{M}}{\partial \bar{z}},$$

which, for  $\bar{\Gamma} \gg 1$ , can be approximated as,  $\partial \bar{\phi}^\alpha / \partial \bar{z} \approx 0$ . A physical way to understand this boundary condition is to recall the image charge picture of the potential under the point charge approximation (Fig. (S5)(c)). Based on this picture, a unit point positive charge located near the interface  $\bar{S}^\text{II}$  will have its first image charge located at the reflection point across the membrane interface. This image charge will also be positive but with a magnitude  $(\bar{\Gamma} - 1)/(\bar{\Gamma} + 1)$ , which for  $\bar{\Gamma} \gg 1$ , will be approximately equal to 1, the magnitude of the original charge. The electric field in the near field will be a superposition of these two charges; the other image charges, which have a negative sign, are located much further away, and will therefore make a negligible contribution to the field in this region. However, by the equality of magnitude and the symmetry of the location, the  $\bar{z}$ -component of the electric field due to the two positive charges will cancel, leading to  $\partial \bar{\phi}^\alpha / \partial \bar{z} \approx 0$  in the near field. However, such a simplification is not possible in the far-field, because the electric field contribution from the negative image charges will no longer be insubstantial in these regions.

With this justification, it is easy to see how the three domains  $\Omega^\text{I}$ ,  $\Omega^\text{II}$ , and  $\Omega^\text{M}$  become effectively decoupled in the near field. Therefore, we can solve the linearized problem on the infinite half-domain of  $\bar{z}' > 0$  with the boundary conditions  $\partial \bar{\phi}^\text{II} / \partial \bar{z} = 0$  and  $\bar{j}_\rho^\text{II} = \bar{j}^\circ$  at  $\bar{z}' = 0$ . Now, consider a point flux on the membrane at  $\bar{r} = 0$  given by

$$\bar{j}_\text{pt}^\circ(\bar{r}, \bar{t}) = \bar{I}(\bar{t}) \frac{\bar{\delta}(\bar{r})}{2\pi\bar{r}}, \quad (\text{S.202})$$

Here,  $\bar{I}$  can be considered as the dimensionless flux, which is a function of time. The solution for this point-wise flux can be expressed as a convolution of the point charge spreading solution (S.201)

$$\bar{\rho}_{\text{pt}}^{\text{II}}(\bar{r}', \bar{t}) = \bar{I}(\bar{t}) * 2 \frac{e^{-t}}{(4\pi\bar{t})^{3/2}} e^{-\bar{r}'^2/4\bar{t}} = 2 \int_0^{\bar{t}} \bar{I}(\bar{t} - \bar{\tau}) \frac{e^{-t}}{(4\pi\bar{t})^{3/2}} e^{-\bar{r}'^2/4\bar{t}} d\bar{\tau}, \quad (\text{S.203})$$

where we observe that the charge density will be radially symmetric in the total radial coordinate,  $\bar{r}' = \sqrt{\bar{r}^2 + \bar{z}'^2}$ . Moreover, since the current  $\bar{I}(\bar{t}) = \bar{I}$  is constant in this problem, we can perform the convolutional integral to obtain

$$\bar{\rho}_{\text{pt}}^{\text{II}}(\bar{r}', \bar{t}) = \frac{\bar{I}}{4\pi\bar{r}'} \left( e^{-\bar{r}'} \operatorname{erfc} \left( \frac{\bar{r}'}{2\sqrt{\bar{t}}} - \sqrt{\bar{t}} \right) + e^{\bar{r}'} \operatorname{erfc} \left( \frac{\bar{r}'}{2\sqrt{\bar{t}}} + \sqrt{\bar{t}} \right) \right), \quad (\text{S.204})$$

as the charge density in the near-field due to a point source. We can then integrate Poisson's equation to find the corresponding electric potential in the near field, using the boundary conditions  $\bar{\phi} \rightarrow 0$  as  $\bar{r}' \rightarrow \infty$  and  $\bar{\phi} < \infty$  at  $\bar{r}' = 0$ . This gives

$$\bar{\phi}_{\text{pt}}^{\text{II}}(\bar{r}', \bar{t}) = \frac{\bar{I}}{4\pi\bar{r}'} \left( 2 - 2e^{-\bar{t}} \operatorname{erf} \left( \frac{\bar{r}'}{2\sqrt{\bar{t}}} \right) - e^{-\bar{r}'} \operatorname{erfc} \left( \frac{\bar{r}'}{2\sqrt{\bar{t}}} - \sqrt{\bar{t}} \right) - e^{\bar{r}'} \operatorname{erfc} \left( \frac{\bar{r}'}{2\sqrt{\bar{t}}} + \sqrt{\bar{t}} \right) \right). \quad (\text{S.205})$$

We can observe that when  $\bar{t} \gg 1$ , both Eqs. (S.204) and (S.205) reach a steady-state given by

$$\bar{\rho}_{\text{SS}}^{\text{II}}(\bar{r}') = \frac{\bar{I}}{2\pi\bar{r}'} e^{-\bar{r}'}, \quad (\text{S.206})$$

$$\bar{\phi}_{\text{SS}}^{\text{II}}(\bar{r}') = \frac{\bar{I}}{2\pi\bar{r}'} (1 - e^{-\bar{r}'}), \quad (\text{S.207})$$

as advertised in the main text. The solution is that of a spherical “dome” of charge centered at the pump and its associated monopole-like potential.

To obtain the near-field solution for a patch of size  $\bar{R}^{\text{P}}$ , the point source solution Eq. (S.204) can be used as a Green's function and integrated over the patch. This gives the near-field approximation for the charge density as

$$\bar{\rho}_{\text{near}}^{\text{II}}(\bar{r}, \bar{z}', \bar{t}) = \int_0^{\bar{R}^{\text{P}}} d\bar{l} \int_0^{2\pi} d\theta \bar{l} \bar{\rho}_{\text{pt}}^{\text{II}} \left( \sqrt{\bar{r}^2 + \bar{l}^2 - 2\bar{r}\bar{l} \cos(\theta) + \bar{z}'^2}, \bar{t} \right), \quad (\text{S.208})$$

where we take  $\bar{I} = \bar{j}_0^{\text{O}}$  and the argument of the point-charge solution comes from applying the law of cosines. We can write an identical expression where we replace  $\bar{\rho}$  with  $\bar{\phi}$  for the potential.

In Fig. 9 of the main text, we compare the solution (S.208) for the charge density and the corresponding solution for the transmembrane potential  $\Delta V^{\text{M}}$  with the FEM simulations. For short times and short distances, the approximate near-field solution agrees well with the numerical simulations. The disagreement at large distances and longer times is due to the failure of the near-field approximation to capture the effects of double-layer reorganization due to the electric field, which results in a power-law scaling.

### (c). Maximal pumping rate and potential difference

The expression in Eq. (S.208) is not analytically tractable for arbitrary  $\bar{r}$  and  $\bar{z}'$ , but we can obtain exact results for  $\bar{r} = 0$  and  $\bar{z}' = 0$ . This is a point on the membrane surface at the center of the pumping patch. Furthermore, it is at this location that both the surface charge and the electric potential will attain their largest magnitude. We have

$$\bar{\rho}_{\text{near}}^{\text{II}}(0, 0, \bar{t}) = 2\pi \int_0^{\bar{R}^{\text{P}}} d\bar{l} \bar{l} \bar{\rho}_{\text{pt}}^{\text{II}}(\bar{l}, \bar{t}), \quad (\text{S.209})$$

which, with Eq. (S.204), gives

$$\bar{\rho}_{\text{near}}^{\text{II}}(0, 0, \bar{t}) = \frac{\bar{j}_0^{\text{O}}}{2} \int_0^{\bar{R}^{\text{P}}} d\bar{l} \left[ e^{-\bar{l}} \operatorname{erfc} \left( \frac{\bar{l}}{2\sqrt{\bar{t}}} - \sqrt{\bar{t}} \right) + e^{\bar{l}} \operatorname{erfc} \left( \frac{\bar{l}}{2\sqrt{\bar{t}}} + \sqrt{\bar{t}} \right) \right]. \quad (\text{S.210})$$

Evaluating this integral gives

$$\bar{\rho}_{\text{near}}^{\text{II}}(0, 0, \bar{t}) = \frac{\bar{j}_0^{\circ}}{2} \left[ 2 \operatorname{erf}(\sqrt{\bar{t}}) - e^{-\bar{R}^{\text{P}}} \operatorname{erfc}\left(\frac{\bar{R}^{\text{P}}}{2\sqrt{\bar{t}}} - \sqrt{\bar{t}}\right) + e^{\bar{R}^{\text{P}}} \operatorname{erfc}\left(\frac{\bar{R}^{\text{P}}}{2\sqrt{\bar{t}}} + \sqrt{\bar{t}}\right) \right]. \quad (\text{S.211})$$

Similarly, for the electric potential, we find that

$$\begin{aligned} \bar{\phi}_{\text{near}}^{\text{II}}(0, 0, \bar{t}) = \frac{\bar{j}_0^{\circ}}{2} & \left[ 2\bar{R}^{\text{P}} - 2\bar{R}^{\text{P}} e^{-\bar{t}} \left[ \operatorname{erf}\left(\frac{\bar{R}^{\text{P}}}{2\sqrt{\bar{t}}}\right) - \frac{1}{\sqrt{\pi}} \frac{2\sqrt{\bar{t}}}{\bar{R}^{\text{P}}} \left(1 - e^{-\frac{(\bar{R}^{\text{P})^2}{4\bar{t}}}\right) \right] \right. \\ & \left. - 2 \operatorname{erf}(\sqrt{\bar{t}}) + e^{-\bar{R}^{\text{P}}} \operatorname{erfc}\left(\frac{\bar{t}}{2\sqrt{\bar{t}}} - \sqrt{\bar{t}}\right) - e^{\bar{R}^{\text{P}}} \operatorname{erfc}\left(\frac{\bar{t}}{2\sqrt{\bar{t}}} + \sqrt{\bar{t}}\right) \right]. \quad (\text{S.212}) \end{aligned}$$

Thus far, we have not considered  $\bar{C}$  for the case of spatially localized pumping. The dynamics of  $\bar{C}$  follows a diffusion equation, based on Eq. (S.87). The corresponding point source solution can be written as

$$\bar{C}_{\text{pt}}^{\text{II}}(\bar{r}', \bar{t}) = \bar{I}(\bar{t}) * 2 \frac{1}{(4\pi\bar{t})^{3/2}} e^{-\bar{r}'^2/4\bar{t}} = 2 \int_0^{\bar{t}} \bar{I}(\bar{t} - \bar{\tau}) \frac{1}{(4\pi\bar{t})^{3/2}} e^{-\bar{r}'^2/4\bar{t}} d\bar{\tau}, \quad (\text{S.213})$$

where  $\bar{I}(\bar{t}) = \bar{I}$ . Moreover, within the linear theory, this solution holds not just in the near field, but in all space. Evaluating the integral in Eq. (S.213) yields

$$\bar{C}_{\text{pt}}^{\text{II}}(\bar{r}', \bar{t}) = \frac{\bar{I}}{2\pi\bar{r}'} \operatorname{erfc}\left(\frac{\bar{r}'}{2\sqrt{\bar{t}}}\right), \quad (\text{S.214})$$

from which we can compute a solution to  $\bar{C}$  for the case of a pumping from a finite patch of size  $\bar{R}^{\text{P}}$ , analogous to the charge density and potential. Similar to Eq. (S.208) we have

$$\bar{C}^{\text{II}}(\bar{r}, \bar{z}', \bar{t}) = \int_0^{\bar{R}^{\text{P}}} d\bar{l} \int_0^{2\pi} d\theta \bar{l} \bar{C}_{\text{pt}}^{\text{II}}\left(\sqrt{\bar{r}^2 + \bar{l}^2 - 2\bar{r}\bar{l}\cos(\theta)} + \bar{z}'^2, \bar{t}\right), \quad (\text{S.215})$$

which holds for all  $\bar{r}$ ,  $\bar{z}'$  and  $\bar{t}$  where the linearization is valid. Evaluating the integral for the case of  $\bar{r} = \bar{z}' = 0$ , we obtain

$$\bar{C}^{\text{II}}(0, 0, \bar{t}) = \bar{j}_0^{\circ} \bar{R}^{\text{P}} \left[ \operatorname{erfc}\left(\frac{\bar{R}^{\text{P}}}{2\sqrt{\bar{t}}}\right) + \frac{1}{\sqrt{\pi}} \frac{2\sqrt{\bar{t}}}{\bar{R}^{\text{P}}} \left(1 - e^{-\frac{(\bar{R}^{\text{P})^2}{4\bar{t}}}\right) \right]. \quad (\text{S.216})$$

We now follow the approach presented earlier in Sec. III.5 to derive bounds on the maximal pumping rate, but as we shall shortly see, end up with a result that is different from the spatially uniform pumping scenario. Recall that for the dimensional cation concentration  $C_{+} = C_0(\bar{\rho} + \bar{C} + 1)$  to be non-negative, we must have  $\bar{\rho} + \bar{C} \geq -1$ . Now, for the case of cation pumping  $\bar{j}_0^{\circ} > 0$ , which results in both  $\bar{\rho}^{\text{I}}, \bar{C}^{\text{I}} < 0$ . Because the solution is odd in  $\bar{z}$ , it must be that  $\bar{\rho}^{\text{II}}, \bar{C}^{\text{II}} > 0$ . Therefore, because the location of the greatest deviation in  $C_{+}$  occurs at the center of the transporter, we must satisfy

$$\bar{C}^{\text{II}}(0, 0, \bar{t}) + \bar{\rho}^{\text{II}}(0, 0, \bar{t}) \leq 1, \quad (\text{S.217})$$

for all times  $\bar{t} \leq \bar{\tau}^{\circ}$ , so that  $\bar{C}^{\text{I}}(0, 0, \bar{t}) + \bar{\rho}^{\text{I}}(0, 0, \bar{t}) \geq -1$  is automatically satisfied. This implies that both  $\bar{C}^{\text{II}}(0, 0, \bar{t})$  and  $\bar{\rho}^{\text{II}}(0, 0, \bar{t})$  must saturate to a steady state if  $\bar{\tau}^{\circ} \gg 1$ . Substituting Eqs. (S.211) and (S.216) in Eq. (S.217) yields

$$1 \geq \frac{\bar{j}_0^{\circ}}{2} \left[ 2 - 2e^{-\bar{R}^{\text{P}}} \right] + \bar{j}_0^{\circ} \bar{R}^{\text{P}} [1 + 0] = \bar{j}_0^{\circ} \left[ 1 - e^{-\bar{R}^{\text{P}}} + \bar{R}^{\text{P}} \right]. \quad (\text{S.218})$$

Thus, for concentrations to remain nonnegative we must have  $\bar{j}_0^{\circ} \leq \left[ 1 - e^{-\bar{R}^{\text{P}}} + \bar{R}^{\text{P}} \right]^{-1}$ . This is an upper bound on the flux as a function of the pore radius that must be satisfied for long pumping times  $\bar{\tau}^{\circ} \gg 1$ . Under this constraint, the pump can be operated indefinitely without achieving negative concentrations,

which is distinct from the case of the spatially uniform pumping problem. There, indefinite pumping is not possible because for any value of the pumping rate, however small, there always exists a maximum time beyond which concentrations become negative.

Now, let us consider the maximum achievable potential difference across the membrane. From Eq. (S.212) for  $\bar{t} \gg 1$ , the transmembrane potential at  $\bar{r} = 0$  is

$$\Delta \bar{V}^M(0, \bar{t}) = \lim_{\bar{t} \rightarrow \infty} 2\bar{\phi}_{\text{near}}^{\text{II}}(0, 0, \bar{t}) = 2\bar{j}_0^o \left( \bar{R}^P - 1 + e^{-\bar{R}^P} \right). \quad (\text{S.219})$$

Combining this result with our constraint on  $\bar{j}_0^o$  from Eq. (S.218), we find that

$$\Delta \bar{V}^M(0, \bar{t}) \leq 2 \frac{\bar{R}^P - 1 + e^{-\bar{R}^P}}{\bar{R}^P + 1 - e^{-\bar{R}^P}}, \quad (\text{S.220})$$

is the maximum achievable transmembrane potential difference at the center of a pumping patch of radius  $\bar{R}^P$ . For any  $\bar{r} > 0$ , we expect that  $\bar{V}^M(\bar{r}, \bar{t}) \leq \bar{V}^M(0, \bar{t})$ . Therefore, we can see using Taylor expansion that when  $\bar{R}^P \ll 1$ , the maximum potential difference that can locally be achieved by a single channel is  $\Delta \bar{V}^M \lesssim \bar{R}^P$  and when  $\bar{R}^P \gg 1$ , it is  $\Delta \bar{V}^M \lesssim 2$ . Since the potential is nondimensionalized by the thermal voltage  $\phi_T \sim 25$  mV, the above constraint suggests that the transmembrane potential difference achievable by a single pump can be at most 50 mV. For  $\bar{R}^P = 1$ , corresponding to a transported opening of  $\sim 1$  nm, we calculate  $\Delta \bar{V}^M \leq 11$  mV. Alternatively, for  $\bar{R}^P = 1$ , corresponding to a opening of  $\sim 2\text{\AA}$ , we find that  $\Delta \bar{V}^M \leq 2.5$  mV. This indicates that to achieve larger transmembrane potential differences, systems of transporters may be necessary.

### 3. Long-time asymptotics

We now derive asymptotic solutions for times  $t \gg \tau_D$ , i.e.  $\bar{t} \gg 1$ , presented in Sec. IVC of the main text. We obtain the exact solution in the Hankel-Laplace transformed space and then consider the asymptotic limits of the transformed solution. Then, the real space solution is found by inverting the asymptotic limit in the transformed space.

#### (a). Derivation of transformed solution

To find an exact solution, we introduce the Laplace transform. We will consider the Laplace transform of a function that has already been Hankel transformed. Accordingly, we denote

$$\check{f}(\hat{k}, \bar{z}, \check{s}) = \int_0^\infty \hat{f}(\hat{k}, \bar{z}, \bar{t}) e^{-\check{s}\bar{t}} d\bar{t}, \quad (\text{S.221})$$

as the Laplace transform of the Hankel-transform  $\hat{f}(\cdot)$  with  $\check{s}$  being the conjugate variable to time. Once again, the linearized governing equations state

$$\frac{\partial \bar{\rho}^\alpha}{\partial \bar{t}} = \bar{\nabla}^2 \bar{\rho}^\alpha - \bar{\rho}^\alpha, \quad (\text{S.222})$$

$$\bar{\nabla}^2 \bar{\phi}^\alpha = -\bar{\rho}^\alpha, \quad (\text{S.223})$$

$$\bar{\nabla}^2 \bar{\phi}^M = 0, \quad (\text{S.224})$$

for  $\alpha \in \{\text{I}, \text{II}\}$ . This is subject to the boundary conditions

$$\frac{\partial \bar{\rho}^\alpha}{\partial \bar{z}} + \frac{\partial \bar{\phi}^\alpha}{\partial \bar{z}} = -\bar{j}^o(\bar{r}, \bar{t}), \quad \text{on } \bar{S}^\alpha, \quad (\text{S.225})$$

$$\frac{\partial \bar{\phi}^\alpha}{\partial \bar{z}} - \frac{1}{\bar{\Gamma}} \frac{\partial \bar{\phi}^M}{\partial \bar{z}} = 0, \quad \text{on } \bar{S}^\alpha, \quad (\text{S.226})$$

$$\bar{\phi}^\alpha - \bar{\phi}^M = 0, \quad \text{on } \bar{S}^\alpha, \quad (\text{S.227})$$

for  $\alpha \in \{I, II\}$ . The initial conditions are  $\bar{\rho}^\alpha = 0$ ,  $\bar{\phi}^\alpha = 0$ , and  $\bar{\rho}^M = 0$  at  $\bar{t} = 0$ . Due to the system being odd in  $\bar{z}$ , we can equivalently solve only in the half-domain  $\bar{z} \geq 0$  using the boundary condition  $\bar{\phi}^M = 0$  at  $\bar{z} = 0$ . The solution for  $\bar{z} < 0$  can then simply be found as  $\check{f}(\hat{k}, -\bar{z}, \check{s}) = -\check{f}(\hat{k}, \bar{z}, \check{s})$ .

Applying the Hankel and Laplace transforms to the governing equations gives

$$\check{s}\check{\rho}^{II} = -\hat{k}^2\check{\rho}^{II} + \frac{\partial^2\check{\rho}^{II}}{\partial\bar{z}^2} - \check{\rho}^{II} , \quad (S.228)$$

$$-\hat{k}^2\check{\phi}^{II} + \frac{\partial^2\check{\phi}^{II}}{\partial\bar{z}^2} = -\check{\rho}^{II} , \quad (S.229)$$

$$-\hat{k}^2\check{\phi}^M + \frac{\partial^2\check{\phi}^M}{\partial\bar{z}^2} = 0 , \quad (S.230)$$

subject to the boundary conditions

$$\frac{\partial\check{\rho}^{II}}{\partial\bar{z}} + \frac{\partial\check{\phi}^{II}}{\partial\bar{z}} = -\check{j}^\circ(\hat{k}, \check{s}) , \quad \text{for } \bar{z} = \frac{\bar{\delta}^M}{2} , \quad (S.231)$$

$$\frac{\partial\check{\phi}^{II}}{\partial\bar{z}} - \frac{1}{\bar{\Gamma}} \frac{\partial\check{\phi}^M}{\partial\bar{z}} = 0 , \quad \text{for } \bar{z} = \frac{\bar{\delta}^M}{2} , \quad (S.232)$$

$$\check{\phi}^{II} - \check{\phi}^M = 0 , \quad \text{for } \bar{z} = \frac{\bar{\delta}^M}{2} , \quad (S.233)$$

$$\check{\phi}^M = 0 , \quad \text{for } \bar{z} = 0 . \quad (S.234)$$

This system of differential equations now only contains derivatives in  $\bar{z}$ , so we can find the solution using standard techniques of ordinary differential equations. The solution is

$$\check{\rho}^{II}(\hat{k}, \bar{z}, \check{s}) = \check{j}^\circ(\hat{k}, \check{s}) \frac{(1 + \check{s})(1 + \bar{\Gamma} \tanh(\hat{k}\bar{h}))e^{-\sqrt{1+\hat{k}^2+\check{s}}(\bar{z}-\bar{h})}}{\hat{k} + (\check{s} + (1 + \check{s})\bar{\Gamma} \tanh(\hat{k}\bar{h}))\sqrt{1+\hat{k}^2+\check{s}}} , \quad (S.235)$$

$$\check{\phi}^{II}(\hat{k}, \bar{z}, \check{s}) = \check{j}^\circ(\hat{k}, \check{s}) \frac{\left(1 + \frac{\bar{\Gamma}}{\hat{k}} \tanh(\hat{k}\bar{h})\sqrt{1+\hat{k}^2+\check{s}}\right)e^{-\hat{k}(\bar{z}-\bar{h})} - (1 + \bar{\Gamma} \tanh(\hat{k}\bar{h}))e^{-\sqrt{1+\hat{k}^2+\check{s}}(\bar{z}-\bar{h})}}{\hat{k} + (\check{s} + (1 + \check{s})\bar{\Gamma} \tanh(\hat{k}\bar{h}))\sqrt{1+\hat{k}^2+\check{s}}} , \quad (S.236)$$

$$\check{\phi}^M(\hat{k}, \bar{z}, \check{s}) = \check{j}^\circ(\hat{k}, \check{s}) \frac{\bar{\Gamma} \tanh(\hat{k}\bar{h}) \left(\frac{1}{\hat{k}}\sqrt{1+\hat{k}^2+\check{s}} - 1\right)}{\hat{k} + (\check{s} + (1 + \check{s})\bar{\Gamma} \tanh(\hat{k}\bar{h}))\sqrt{1+\hat{k}^2+\check{s}}} \frac{\sinh(\hat{k}\bar{z})}{\sinh(\hat{k}\bar{h})} , \quad (S.237)$$

where  $\bar{h} = \bar{\delta}^M/2$ , as before. For the imposed flux function in this problem

$$\bar{j}^\circ(\bar{r}, \bar{t}) = \bar{j}_0^\circ \Theta(\bar{R}^P - \bar{r}) , \quad (S.238)$$

the Hankel-Laplace transform is

$$\check{j}^\circ(\hat{k}, \check{s}) = \frac{\bar{j}_0^\circ}{\check{s}} \frac{\bar{R}^P J_1(\bar{R}^P \hat{k})}{\hat{k}} , \quad (S.239)$$

where  $J_1$  is the Bessel function of the first kind of order one [1]. If we consider  $\bar{R}^P \ll \bar{r}$ , equivalent to  $\bar{R}^P \hat{k} \ll 1$ , we can then approximate

$$\check{j}^\circ(\hat{k}, \check{s}) \approx \frac{\bar{j}_0^\circ}{\check{s}} \frac{\bar{R}^P (\bar{R}^P \hat{k})/2}{\hat{k}} = \frac{\bar{I}}{2\pi\check{s}} , \quad (S.240)$$

where  $\bar{I} = \pi(\bar{R}^P)^2 \bar{j}_0^\circ$  is now the *total* flow rate of ions through the patch.

## (b). Expansion for large distances and times

We take asymptotic expansions of the above solution to find analytical solutions in real space. First, we observe from the numerical results that for large values of  $\bar{r}$  and  $\bar{t}$ , the solution appears self-similar in  $\bar{r}/\bar{t}$ , as

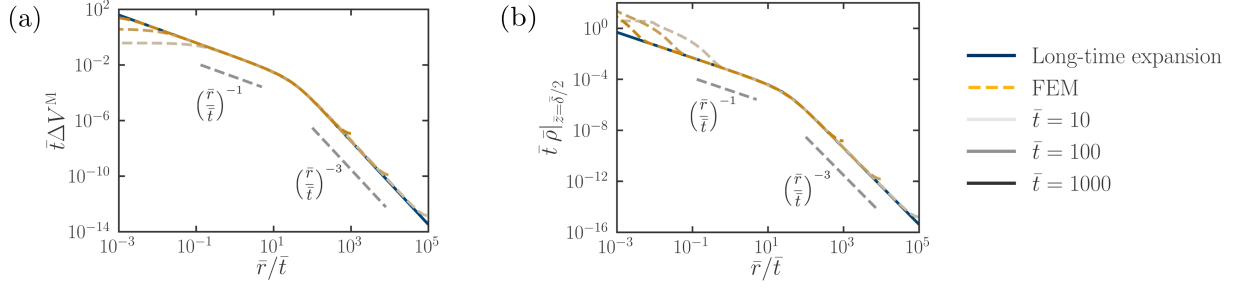

Figure S6: Rescaling of (a) transmembrane potential and (b) charge density at the surface by  $\bar{t}$  plotted against  $\bar{r}/\bar{t}$  to show the collapse that occurs for large values of  $\bar{r}$  and  $\bar{t}$ , in a manner reminiscent of self-similar solutions.

shown in Fig. S6. In the transformed space, this corresponds to  $\bar{s}/\hat{k}$ . Accordingly, we consider the asymptotic expansion for large  $\bar{r}$  and large  $\bar{t}$  simultaneously by taking the limit for small  $\hat{k}$  and small  $\bar{s}$  with  $\bar{s}/\hat{k}$  fixed. In this limit, we also approximate  $\hat{j}^o(\hat{k}, \bar{s}) = \bar{I}/2\pi\bar{s}$  based on Eq. (S.240).

Introducing the variable  $\bar{\psi} = \bar{s}/\hat{k}$ , and applying the limit  $\hat{k}, \bar{s} \rightarrow 0$  with  $\bar{\psi}$  fixed to Eqs. (S.235)-(S.237), yields

$$\hat{\rho}^{\text{II}}(\hat{k}, \bar{z}, \bar{\psi}) \approx \frac{\bar{I}}{2\pi \hat{k}^2} \frac{e^{-(\bar{z}-\bar{h})}}{(\bar{\psi}(1 + \bar{\Gamma}\bar{h}) + \bar{\psi}^2)}, \quad (\text{S.241})$$

$$\hat{\phi}^{\text{II}}(\hat{k}, \bar{z}, \bar{\psi}) \approx \frac{\bar{I}}{2\pi} \frac{(1 + \bar{\Gamma}\bar{h})e^{-\hat{k}(\bar{z}-\bar{h})} - e^{-(\bar{z}-\bar{h})}}{\hat{k}^2 (\bar{\psi}(1 + \bar{\Gamma}\bar{h}) + \bar{\psi}^2)}, \quad (\text{S.242})$$

$$\hat{\phi}^{\text{M}}(\hat{k}, \bar{z}, \bar{\psi}) \approx \frac{\bar{I}}{2\pi \hat{k}^2} \frac{\bar{\Gamma}\bar{h}}{(\bar{\psi}(1 + \bar{\Gamma}\bar{h}) + \bar{\psi}^2)} \frac{\bar{z}}{\bar{h}}, \quad (\text{S.243})$$

for  $\hat{k} \ll 1$ . We now define the dimensionless velocity  $\bar{v} \equiv 1 + \bar{\Gamma}\bar{h} = 1 + \bar{\Gamma}\bar{\delta}^{\text{M}}/2$ . Resubstituting  $\bar{\psi} = \bar{s}/\hat{k}$  and simplifying, we have

$$\hat{\rho}^{\text{II}}(\hat{k}, \bar{z}, \bar{s}) \approx \frac{\bar{I}}{2\pi} \frac{e^{-(\bar{z}-\bar{h})}}{\bar{v}\hat{s}\hat{k} + \bar{s}^2}, \quad (\text{S.244})$$

$$\hat{\phi}^{\text{II}}(\hat{k}, \bar{z}, \bar{s}) \approx \frac{\bar{I}}{2\pi} \frac{\bar{v}e^{-\hat{k}(\bar{z}-\bar{h})} - e^{-(\bar{z}-\bar{h})}}{\bar{v}\hat{s}\hat{k} + \bar{s}^2}, \quad (\text{S.245})$$

$$\hat{\phi}^{\text{M}}(\hat{k}, \bar{z}, \bar{s}) \approx \frac{\bar{I}}{2\pi} \frac{\bar{v} - 1}{\bar{v}\hat{s}\hat{k} + \bar{s}^2} \frac{\bar{z}}{\bar{h}}. \quad (\text{S.246})$$

Computing the exact inverse Laplace transform and inverse Hankel transform of these asymptotic forms gives

$$\bar{\rho}^{\text{II}}(\bar{r}, \bar{z}, \bar{t}) \approx \frac{\bar{I}}{2\pi} \frac{e^{-\bar{z}'}}{\bar{v}\bar{r}} \left[ 1 - \frac{1}{\sqrt{1 + (\bar{v}\bar{t}/\bar{r})^2}} \right], \quad (\text{S.247})$$

$$\bar{\phi}^{\text{II}}(\bar{r}, \bar{z}, \bar{t}) \approx \frac{\bar{I}}{2\pi} \left( \left[ \frac{1}{\sqrt{\bar{r}^2 + \bar{z}'^2}} - \frac{1}{\sqrt{\bar{r}^2 + (\bar{v}\bar{t} + \bar{z}')^2}} \right] - \frac{e^{-\bar{z}'}}{\bar{v}\bar{r}} \left[ 1 - \frac{1}{\sqrt{1 + (\bar{v}\bar{t}/\bar{r})^2}} \right] \right), \quad (\text{S.248})$$

$$\bar{\phi}^{\text{M}}(\bar{r}, \bar{z}, \bar{t}) \approx \frac{\bar{I}}{2\pi} \left( 1 - \frac{1}{\bar{v}} \right) \frac{1}{\bar{r}} \left[ 1 - \frac{1}{\sqrt{1 + (\bar{v}\bar{t}/\bar{r})^2}} \right] \frac{\bar{z}}{\bar{h}}. \quad (\text{S.249})$$

We see that the charge density decays in  $\bar{z}'$  exponentially, as in a one-dimensional double layer, with radial dependence following a monopole for  $\bar{r} \ll \bar{v}\bar{t}$  and a dipole for  $\bar{r} \gg \bar{v}\bar{t}$ . The potential also follows decays as a monopole for  $\bar{r} \ll \bar{v}\bar{t}$  and a dipole for  $\bar{r} \gg \bar{v}\bar{t}$ . The potential has two contributions, one corresponding

to the effective point charges on either side of the membrane, as well as a second term that represents the adjustment of the electrical potential by the diffuse charge layer. For the transmembrane potential, we find

$$\Delta \bar{V}^M(\bar{r}, \bar{t}) \approx \frac{\bar{I}}{\pi} \left(1 - \frac{1}{\bar{v}}\right) \frac{1}{\bar{r}} \left[1 - \frac{1}{\sqrt{1 + (\bar{v}\bar{t}/\bar{r})^2}}\right], \quad (\text{S.250})$$

which is linearly proportional to the surface charge density solution, but differs by a factor of  $2(\bar{v} - 1) = \bar{\Gamma}\bar{\delta}^M$ . This is nothing but the per-area capacitance of the membrane, which is consistent with a local circuit model.

## 4. Analysis of second moments

We now use the results from the previous sections to discuss both the radial and axial second moments of the charge density, which are compared with the numerical results in the main text.

### (a). Early times

We first present computations of the second moments at early times. The axial second moment of the charge density is defined by

$$\langle \bar{z}'^2 \rangle_{\bar{\rho}}(\bar{t}) = \frac{\int_{\bar{\Omega}^{\text{II}}} \bar{z}'^2 \bar{\rho} d\bar{\Omega}}{\int_{\bar{\Omega}^{\text{II}}} \bar{\rho} d\bar{\Omega}}, \quad (\text{S.251})$$

where  $\bar{z}' = \bar{z} - \bar{\delta}^M/2$ . To evaluate the above, we first note that the integral of charge density in the denominator is simply the total pumped charge,  $\bar{I}\bar{t}$ . On the other hand, the integral in the numerator can be broken as

$$\int_{\bar{\Omega}^{\text{II}}} \bar{z}'^2 \bar{\rho} d\bar{\Omega} = \int_0^{\bar{R}} 2\pi\bar{r} d\bar{r} \int_0^\infty d\bar{z}' \left[ \bar{z}'^2 \bar{\rho}_{\text{pt}}^{\text{II}} \right] + \int_{\bar{R}}^{\bar{L}} 2\pi\bar{r} d\bar{r} \int_0^\infty d\bar{z}' \left[ \bar{z}'^2 \bar{\rho}_{\text{pc}}^{\text{II}} \right], \quad (\text{S.252})$$

where the first and second integrals on the right-hand side are contributions from the near-field and the other regions, respectively. Here,  $\bar{R} \sim \mathcal{O}(1)$  is the transition location between the near-field and intermediate regimes,  $\bar{\rho}_{\text{pt}}^{\text{II}}$  is the point source solution in Eq. (S.204), and  $\bar{\rho}_{\text{pc}}^{\text{II}}$  is the charge density obtained by the point charge approximation in Eq. (S.190). Since the point source solution decays rapidly with  $\bar{r}$ , we can extend the upper limit from  $\bar{R}$  to  $\infty$  to approximate the first integral on the right-hand side, which makes the integration domain becomes semi-infinite ( $\bar{z}' > 0$ ). By using the spherical symmetry of  $\bar{\rho}_{\text{pt}}^{\text{II}}$ , we rewrite the integral

$$\int_0^{\bar{R}} 2\pi\bar{r} d\bar{r} \int_0^\infty d\bar{z}' \left[ \bar{z}'^2 \bar{\rho}_{\text{pt}}^{\text{II}} \right] \approx \int_0^\infty 2\pi\bar{r} d\bar{r} \int_0^\infty d\bar{z}' \left[ \bar{z}'^2 \bar{\rho}_{\text{pt}}^{\text{II}} \right] = \int_0^\infty 2\pi\bar{r}'^2 d\bar{r}'^2 \left[ \bar{z}'^2 \bar{\rho}_{\text{pt}}^{\text{II}} \right], \quad (\text{S.253})$$

where  $\bar{r}' = \sqrt{\bar{r}^2 + (\bar{z}')^2} = \sqrt{\bar{x}^2 + \bar{y}^2 + (\bar{z}')^2}$  is the total radial coordinate. The spherical symmetry also implies that the second moments in  $\bar{x}$ ,  $\bar{y}$ , and  $\bar{z}'$  are all equal. Now, we substitute the point source solution from Eq. (S.204) to obtain

$$\int_0^\infty 2\pi\bar{r}'^2 d\bar{r}'^2 \left[ \bar{z}'^2 \bar{\rho}_{\text{pt}}^{\text{II}} \right] \approx \frac{1}{3} \int_0^\infty 2\pi\bar{r}'^2 d\bar{r}'^2 \left[ \bar{r}'^2 \bar{\rho}_{\text{pt}}^{\text{II}} \right] = \bar{I} \left( 2 - 2(1 + \bar{t})e^{-\bar{t}} \right). \quad (\text{S.254})$$

It is easy to see that the leading order behavior at early times  $\bar{t} \ll 1$  is  $\bar{I}\bar{t}^2$ .

Now we compute contributions from the intermediate and far-field regions. Direct integration upon substitution of Eq. (S.190) yields

$$\int_{\bar{R}}^{\bar{L}} 2\pi\bar{r} d\bar{r} \int_0^\infty d\bar{z}' \left[ \bar{z}'^2 \bar{\rho}_{\text{pc}}^{\text{II}} \right] = -2 \left( -2 + \bar{t} + (2 + \bar{t})e^{-\bar{t}} \right) \int_{\bar{R}}^{\bar{L}} 2\pi\bar{r} d\bar{r} \left[ \frac{\bar{E}_z^{\text{pc,II}}|_{\bar{z}'=0}}{\bar{t}} \right], \quad (\text{S.255})$$

where  $\bar{E}_z^{\text{pc,II}}|_{\bar{z}'=0}$  is a function of  $\bar{r}$  and  $\bar{t}$  given by Eq. (S.196). Note that  $\bar{E}_z^{\text{pc,II}}$  is proportional to the pumped charge  $\bar{I}\bar{t}$ , and therefore the last integrand  $\bar{E}_z^{\text{pc,II}}/\bar{t}$  is constant in time. Also, Taylor expansion of the expression in the parentheses identifies  $\bar{t}^3/6$  as its leading order behavior at early times  $\bar{t} \ll 1$ . Therefore,

$$\int_{\bar{R}}^{\bar{L}} 2\pi\bar{r} d\bar{r} \int_0^\infty d\bar{z}' \left[ \bar{z}'^2 \bar{\rho}_{\text{pc}}^{\text{II}} \right] \approx -\frac{1}{3}\bar{t}^3 \int_{\bar{R}}^{\bar{L}} 2\pi\bar{r} d\bar{r} \left[ \frac{\bar{E}_z^{\text{pc,II}}|_{\bar{z}'=0}}{\bar{t}} \right]. \quad (\text{S.256})$$

We now substitute expression for  $\bar{E}_z^{\text{pc},\text{II}}|_{\bar{z}=0}$  from Eq. (S.196). Since the integral is dominated by contribution from  $\bar{r} \gg \bar{R} \sim \bar{\delta}^{\text{M}}/2$ , we use the expression for the far field to obtain

$$\int_{\bar{R}}^{\bar{L}} 2\pi\bar{r} d\bar{r} \left[ \frac{\bar{E}_z^{\text{pc},\text{II}}|_{\bar{z}=0}}{\bar{t}} \right] \approx \int_{\bar{R}}^{\bar{L}} 2\pi\bar{r} d\bar{r} \left[ -\frac{\bar{\Gamma}\bar{\delta}^{\text{M}}\bar{I}}{4\pi\bar{r}^3} \right] = -\frac{1}{2}\bar{I}\bar{\Gamma}\bar{\delta}^{\text{M}} \left[ \frac{1}{\bar{R}} - \frac{1}{\bar{L}} \right]. \quad (\text{S.257})$$

Therefore, the far-field contribution to the second moment is

$$\int_{\bar{R}}^{\bar{L}} 2\pi\bar{r} d\bar{r} \int_0^\infty d\bar{z}' \left[ \bar{z}'^2 \bar{\rho}_{\text{pc}}^{\text{II}} \right] \approx \frac{1}{6} \bar{I}\bar{\Gamma}\bar{\delta}^{\text{M}}\bar{t}^3 \frac{1}{\bar{R}}, \quad (\text{S.258})$$

where we use  $\bar{L} \gg \bar{R}$ . At early times,  $\mathcal{O}(\bar{t}^2)$  contribution from the near field dominates the  $\mathcal{O}(\bar{t}^3)$  contribution from the others. Therefore, to leading order early-time behavior is given by

$$\langle \bar{z}'^2 \rangle_{\bar{\rho}}(\bar{t}) \approx \frac{\bar{I}\bar{t}^2}{\bar{I}\bar{t}} = \bar{t}, \quad (\text{S.259})$$

which agrees well with the numerical result as shown in the main text and is also equal to the result expected from bare diffusion [5].

We follow the same procedure for the radial moment by dividing the integral between the near-field and intermediate/far-field regions and calculating the contributions from each. We have

$$\int_{\bar{\Omega}^{\text{II}}} \bar{r}^2 \bar{\rho} d\bar{\Omega} = \int_0^{\bar{R}} 2\pi\bar{r} d\bar{r} \int_0^\infty d\bar{z}' \left[ \bar{r}^2 \bar{\rho}_{\text{pt}}^{\text{II}} \right] + \int_{\bar{R}}^{\bar{L}} 2\pi\bar{r} d\bar{r} \int_0^\infty d\bar{z}' \left[ \bar{r}^2 \bar{\rho}_{\text{pc}}^{\text{II}} \right]. \quad (\text{S.260})$$

For the near-field contribution,  $\bar{r}^2 = \bar{x}^2 + \bar{y}^2$ , so by the symmetry arguments  $\langle \bar{r}^2 \rangle = 2\langle \bar{r}'^2 \rangle/3$ , giving

$$\int_0^{\bar{R}} 2\pi\bar{r} d\bar{r} \int_0^\infty d\bar{z}' \left[ \bar{r}^2 \bar{\rho}_{\text{pt}}^{\text{II}} \right] \approx 2\bar{I} \left( 2 - 2(1 + \bar{t})e^{-\bar{t}} \right) \approx 2\bar{I}\bar{t}^2, \quad (\text{S.261})$$

to leading order at early time  $\bar{t} \ll 1$ .

For the intermediate and far-field contributions, we have

$$\int_{\bar{R}}^{\bar{L}} 2\pi\bar{r} d\bar{r} \int_0^\infty d\bar{z}' \left[ \bar{r}^2 \bar{\rho}_{\text{pc}}^{\text{II}} \right] = - \left( -1 + \bar{t} + e^{-\bar{t}} \right) \int_{\bar{R}}^{\bar{L}} 2\pi\bar{r} d\bar{r} \left[ \bar{r}^2 \frac{\bar{E}_z^{\text{pc},\text{II}}}{\bar{t}} \right]. \quad (\text{S.262})$$

To the leading order, the time-dependent term in the parentheses behaves as  $\bar{t}^2/2$  for  $\bar{t} \ll 1$ , yielding

$$\int_{\bar{R}}^{\bar{L}} 2\pi\bar{r} d\bar{r} \int_0^\infty d\bar{z}' \left[ \bar{r}^2 \bar{\rho}_{\text{pc}}^{\text{II}} \right] \approx -\frac{1}{2}\bar{t}^2 \int_{\bar{R}}^{\bar{L}} 2\pi\bar{r} d\bar{r} \left[ \bar{r}^2 \frac{\bar{E}_z^{\text{pc},\text{II}}}{\bar{t}} \right]. \quad (\text{S.263})$$

Again, by using exclusively the far-field expression for  $\bar{E}_z^{\text{pc},\text{II}}|_{\bar{z}=0}$  in Eq. (S.196), we find

$$\int_{\bar{R}}^{\bar{L}} 2\pi\bar{r} d\bar{r} \left[ \bar{r}^2 \frac{\bar{E}_z^{\text{pc},\text{II}}}{\bar{t}} \right] \approx - \int_{\bar{R}}^{\bar{L}} d\bar{r} \left[ \frac{1}{2} \bar{\Gamma} \bar{\delta}^{\text{M}} \bar{I} \right] = -\frac{1}{2} \bar{I} \bar{\Gamma} \bar{\delta}^{\text{M}} (\bar{L} - \bar{R}). \quad (\text{S.264})$$

Therefore, the far-field contribution to the second moment is

$$\int_{\bar{R}}^{\bar{L}} 2\pi\bar{r} d\bar{r} \int_0^\infty d\bar{z}' \left[ \bar{r}^2 \bar{\rho}_{\text{pc}}^{\text{II}} \right] \approx \frac{1}{4} \bar{I} \bar{\Gamma} \bar{\delta}^{\text{M}} \bar{t}^2 \bar{L}, \quad (\text{S.265})$$

where we use  $\bar{L} \gg \bar{R}$ . Since  $\bar{\Gamma}, \bar{L} \gg 1$ , the intermediate and far-field contribution dominates the  $2\bar{I}\bar{t}^2$  contribution from the near field. Therefore, the radial second moment is given by

$$\langle \bar{r}^2 \rangle_{\bar{\rho}}(\bar{t}) \approx \frac{1}{4} \bar{\Gamma} \bar{\delta}^{\text{M}} \bar{L} \bar{t}, \quad (\text{S.266})$$

to leading order in short time and large system size. The effective diffusivity is therefore  $\bar{\Gamma}\bar{\delta}^{\text{M}}\bar{L}/8$ , which scales linearly with the system size  $\bar{L}$ , as observed from numerical simulations. We note that this is much faster than bare diffusive process and the effective diffusivity would diverge in the limit of an infinite system size.

### (b). Late times

We use the same strategy to obtain the second moments for late times. The main difference is the usage of the long-time asymptotic expression for charge density given by Eq. (S.247) instead of the point charge solution.

For the axial moment, we begin with

$$\int_{\bar{\Omega}^{\text{II}}} \bar{z}'^2 \bar{\rho} d\bar{\Omega} = \int_0^{\bar{R}} 2\pi\bar{r} d\bar{r} \int_0^\infty d\bar{z}' \left[ \bar{z}'^2 \bar{\rho}_{\text{pt}}^{\text{II}} \right] + \int_{\bar{R}}^{\bar{L}} 2\pi\bar{r} d\bar{r} \int_0^\infty d\bar{z}' \left[ \bar{z}'^2 \bar{\rho}^{\text{II}} \right]. \quad (\text{S.267})$$

The near-field contribution is unchanged from the early-time calculations, except we now consider the other limit  $\bar{t} \gg 1$ , which gives

$$\int_0^{\bar{R}} 2\pi\bar{r} d\bar{r} \int_0^\infty d\bar{z}' \left[ \bar{z}'^2 \bar{\rho}_{\text{pt}}^{\text{II}} \right] \approx 2\bar{I}. \quad (\text{S.268})$$

This is a constant in time since the near field reaches a steady state within a few Debye times. For the far-field contribution, we use the long-time asymptotic solution in Eq. (S.247) to write

$$\int_{\bar{R}}^{\bar{L}} 2\pi\bar{r} d\bar{r} \int_0^\infty d\bar{z}' \left[ \bar{z}'^2 \bar{\rho}^{\text{II}} \right] = \int_{\bar{R}}^{\bar{L}} 2\pi\bar{r} d\bar{r} \int_0^\infty d\bar{z}' \left[ \bar{z}'^2 \frac{\bar{I} e^{-\bar{z}'}}{2\pi\bar{v}\bar{r}} \left[ 1 - \left( 1 + \left( \frac{\bar{v}\bar{t}}{\bar{r}} \right)^2 \right)^{-\frac{1}{2}} \right] \right]. \quad (\text{S.269})$$

Separating the integrals in  $\bar{r}$  and  $\bar{z}'$ ,

$$\int_{\bar{R}}^{\bar{L}} 2\pi\bar{r} d\bar{r} \int_0^\infty d\bar{z}' \left[ \bar{z}'^2 \bar{\rho}^{\text{II}} \right] = \int_{\bar{R}}^{\bar{L}} 2\pi\bar{r} d\bar{r} \left[ \frac{\bar{I}}{2\pi\bar{v}\bar{r}} \left[ 1 - \left( 1 + \left( \frac{\bar{v}\bar{t}}{\bar{r}} \right)^2 \right)^{-\frac{1}{2}} \right] \right] \int_0^\infty d\bar{z}' \left[ \bar{z}'^2 e^{-\bar{z}'} \right]. \quad (\text{S.270})$$

The leading order behavior of the above expression at late times  $\bar{t} \gg 1$  is clearly revealed by considering the total charge in the intermediate and far-field regions:

$$\int_{\bar{R}}^{\bar{L}} 2\pi\bar{r} d\bar{r} \int_0^\infty d\bar{z}' \bar{\rho}^{\text{II}} = \int_{\bar{R}}^{\bar{L}} 2\pi\bar{r} d\bar{r} \left[ \frac{\bar{I}}{2\pi\bar{v}\bar{r}} \left[ 1 - \left( 1 + \left( \frac{\bar{v}\bar{t}}{\bar{r}} \right)^2 \right)^{-\frac{1}{2}} \right] \right] \int_0^\infty d\bar{z}' e^{-\bar{z}'} . \quad (\text{S.271})$$

Once the near field reaches a steady state, all the extra pumped charges are distributed outside it. Thus, the above expression converges to the total pumped charge  $\bar{I}\bar{t}$  in the limit of  $\bar{t} \rightarrow \infty$ . Now, comparing Eqs. (S.270) and (S.271), the second moment is given by the ratio of the above two expressions:

$$\langle \bar{z}'^2 \rangle_{\bar{\rho}(\bar{t})} \approx \frac{\int_0^\infty d\bar{z}' \left[ \bar{z}'^2 e^{-\bar{z}'} \right]}{\int_0^\infty d\bar{z}' e^{-\bar{z}'}} = 2, \quad (\text{S.272})$$

which is exactly the expression for the second moment of the exponential distribution. This arises because at long times, the diffuse charge layer reaches a quasi-steady state at all positions, with net charge organized as  $e^{-\bar{z}'}$  from the surface. Thus, the second moment of this distribution will be the second moment of the exponential distribution. This constant limiting value implies that the net charge is confined to the diffuse charge layer even at long times  $\bar{t} \gg 1$ .

For the radial moment at long times, we begin with

$$\int_{\bar{\Omega}^{\text{II}}} \bar{r}^2 \bar{\rho} d\bar{\Omega} = \int_0^{\bar{R}} 2\pi\bar{r} d\bar{r} \int_0^\infty d\bar{z}' \left[ \bar{r}^2 \bar{\rho}_{\text{pt}}^{\text{II}} \right] + \int_{\bar{R}}^{\bar{L}} 2\pi\bar{r} d\bar{r} \int_0^\infty d\bar{z}' \left[ \bar{r}^2 \bar{\rho}^{\text{II}} \right]. \quad (\text{S.273})$$

As with the axial moment, we consider the long-time limit of the near-field contribution, which gives

$$\int_0^{\bar{R}} 2\pi\bar{r} d\bar{r} \int_0^\infty d\bar{z}' \left[ \bar{r}^2 \bar{\rho}_{\text{pt}}^{\text{II}} \right] \approx 4\bar{I}. \quad (\text{S.274})$$

Again, since the near-field reaches a steady state, the contribution from this region to the total integral is constant. For the far-field contribution, we have

$$\int_{\bar{R}}^{\bar{L}} 2\pi\bar{r} d\bar{r} \int_0^\infty d\bar{z}' \left[ \bar{r}^2 \bar{\rho}^{\text{II}} \right] = \int_{\bar{R}}^{\bar{L}} 2\pi\bar{r} d\bar{r} \int_0^\infty d\bar{z}' \left[ \bar{r}^2 \frac{\bar{I} e^{-\bar{z}'}}{2\pi\bar{v}\bar{r}} \left[ 1 - \left( 1 + \left( \frac{\bar{v}\bar{t}}{\bar{r}} \right)^2 \right)^{-\frac{1}{2}} \right] \right], \quad (\text{S.275})$$

where we substituted the long-time solution for the charge density in Eq. (S.247). As with the axial moment, we can separate the integral

$$\int_{\bar{R}}^{\bar{L}} 2\pi\bar{r} d\bar{r} \int_0^\infty d\bar{z}' \left[ \bar{r}^2 \bar{\rho}^{\text{II}} \right] = \int_{\bar{R}}^{\bar{L}} 2\pi\bar{r} d\bar{r} \left[ \bar{r}^2 \frac{\bar{I}}{2\pi\bar{v}\bar{r}} \left[ 1 - \left( 1 + \left( \frac{\bar{v}\bar{t}}{\bar{r}} \right)^2 \right)^{-\frac{1}{2}} \right] \right] \int_0^\infty d\bar{z}' e^{-\bar{z}'}. \quad (\text{S.276})$$

The integral in  $\bar{z}'$  has value 1. In the far field,  $\bar{\rho}$  scales as  $1/\bar{r}^3$ . Since the integrand has factors of the Jacobian  $\bar{r}$  and the second moment  $\bar{r}^2$ , the radial dependency vanishes at large  $\bar{r}$ . Namely, the whole integrand approaches

$$\frac{1}{2} \bar{I} \bar{v} \bar{t}^2, \quad (\text{S.277})$$

for  $\bar{r} \gg \bar{\Gamma} \bar{\delta}^{\text{M}}$ . With our choice of sufficiently large system size  $\bar{L} \gg \bar{\Gamma} \bar{\delta}^{\text{M}}$ , we can approximate the integral as

$$\int_{\bar{R}}^{\bar{L}} 2\pi\bar{r} d\bar{r} \left[ \bar{r}^2 \frac{\bar{I}}{2\pi\bar{v}\bar{r}} \left[ 1 - \left( 1 + \left( \frac{\bar{v}\bar{t}}{\bar{r}} \right)^2 \right)^{-\frac{1}{2}} \right] \right] \approx \int_{\bar{R}}^{\bar{L}} d\bar{r} \left[ \frac{1}{2} \bar{I} \bar{v} \bar{t}^2 \right] \approx \frac{1}{2} \bar{I} \bar{v} \bar{t}^2 \bar{L}, \quad (\text{S.278})$$

where we use  $\bar{L} \gg \bar{R}$ . Since this term scales as  $\bar{t}^2$  at late times, it dominates the contribution from the near field that is constant in time. Accordingly, for  $\bar{t} \gg 1$ , the leading order behavior of the radial second moment is given by

$$\langle \bar{r}^2 \rangle_{\bar{\rho}}(\bar{t}) = \frac{1}{2} \bar{v} \bar{L} \bar{t}, \quad (\text{S.279})$$

for large values of  $\bar{t}$ . Substituting the value of  $\bar{v} = 1 + \bar{\Gamma} \bar{\delta}^{\text{M}}/2$ , we have

$$\langle \bar{r}^2 \rangle_{\bar{\rho}}(\bar{t}) = \frac{1}{4} \bar{\Gamma} \bar{\delta}^{\text{M}} \bar{L} \left( 1 + \frac{2}{\bar{\Gamma} \bar{\delta}^{\text{M}}} \right) \bar{t}. \quad (\text{S.280})$$

When  $\bar{\Gamma} \bar{\delta}^{\text{M}} \gg 1$ , as is the case in biological settings, the early-time and late-time behaviors of the second radial moment coincide. In addition, we note the linear scaling of the radial second moment with the system size  $\bar{L}$ .

## 5. Relaxation dynamics

We can describe relaxation dynamics as the superposition of two charging dynamics solutions, in an analogous manner to the uniform transport case. Suppose that we denote the charging dynamics solution by  $\bar{\rho}_{\text{chg}}(\bar{\mathbf{x}}, \bar{t})$  where  $\bar{\mathbf{x}}$  is the dimensionless position, and  $\bar{t}$  is time from opening. Then, given an open time  $\bar{\tau}^0$ , for times  $\bar{t} > \bar{\tau}^0$ , the charge density during relaxation is given by

$$\bar{\rho}_{\text{rlx}}(\bar{\mathbf{x}}, \bar{t}) = \bar{\rho}_{\text{chg}}(\bar{\mathbf{x}}, \bar{t}) - \bar{\rho}_{\text{chg}}(\bar{\mathbf{x}}, \bar{t} - \bar{\tau}^0). \quad (\text{S.281})$$

For  $\bar{t} \gg \bar{\tau}^0$ , we can perform a Taylor expansion obtaining

$$\bar{\rho}_{\text{rlx}}(\bar{\mathbf{x}}, \bar{t}) = \bar{\tau}^0 \frac{\bar{\rho}_{\text{chg}}(\bar{\mathbf{x}}, \bar{t}) - \bar{\rho}_{\text{chg}}(\bar{\mathbf{x}}, \bar{t} - \bar{\tau}^0)}{\bar{\tau}^0} \approx \bar{\tau}^0 \frac{\partial \bar{\rho}_{\text{chg}}(\bar{\mathbf{x}}, \bar{t})}{\partial \bar{t}}, \quad (\text{S.282})$$

such that the relaxation solution is related to the derivative of the charging solution. One way to interpret this result is that, for times much longer than the open time, the relaxation solution is the response to an impulse pumping. Conversely, the charging solution would be the integral of this Green's function over the open time.

By substituting  $\bar{\rho}_{\text{chg}}$  based on the asymptotic charging solution in the far field (Eq. (S.247)) we find the relaxation solution in domain II to be

$$\bar{\rho}^{\text{II}}(\bar{r}, \bar{z}, \bar{t}) = \frac{\bar{I}\bar{\tau}^{\text{o}}}{2\pi} e^{-\bar{z}} \frac{\bar{v}\bar{t}}{(\bar{r}^2 + (\bar{v}\bar{t})^2)^{\frac{3}{2}}} . \quad (\text{S.283})$$

It is clear that the relaxation solution scales linearly with the total transported charge,  $\bar{q} = \bar{I}\bar{\tau}^{\text{o}}$ . Further, there is a near-field/intermediate regime  $\bar{r} \ll \bar{v}\bar{t}$  where  $\bar{\rho} \sim 1/(\bar{v}\bar{t})^2$  and a far-field regime  $\bar{r} \gg \bar{v}\bar{t}$  where  $\bar{\rho} \sim \bar{v}\bar{t}/\bar{r}^3$ , recovering the plateau and the dipolar regions as noted in the main text.

For the electric potential, we have

$$\bar{\phi}^{\text{II}}(\bar{r}, \bar{z}, \bar{t}) = \frac{\bar{I}\bar{\tau}^{\text{o}}}{2\pi} \left[ \frac{\bar{v}(\bar{v}\bar{t} + \bar{z}')}{(\bar{r}^2 + (\bar{v}\bar{t} + \bar{z}')^2)^{\frac{3}{2}}} - e^{-\bar{z}} \frac{\bar{v}\bar{t}}{(\bar{r}^2 + (\bar{v}\bar{t})^2)^{\frac{3}{2}}} \right] . \quad (\text{S.284})$$

The transmembrane potential then follows

$$\Delta\bar{V}^{\text{M}}(\bar{r}, \bar{t}) = \frac{\bar{I}\bar{\tau}^{\text{o}}}{\pi} \frac{(\bar{v} - 1)\bar{v}\bar{t}}{(\bar{r}^2 + (\bar{v}\bar{t})^2)^{\frac{3}{2}}} , \quad (\text{S.285})$$

which is again related to the surface charge density by a factor of  $2(\bar{v} - 1)$ , as we saw in Eq. (S.250).

The steady-state condition in response to the impulse of charge is the entire system decaying to an equilibrium solution  $\Delta\bar{V}^{\text{M}} = \text{const}$  and  $\bar{\rho} = \text{const}$ —the finite amount of pumped charge ultimately spreads uniformly over the membrane's surface area. However, we see from the form of the charge density and the potential that the transient behavior is governed by the length scale  $\bar{R}^*(\bar{t}) = \bar{v}\bar{t}$ . When  $\bar{r} \ll \bar{R}^*$ , the charge density and transmembrane potential scale as  $1/\bar{t}^2$  and when  $\bar{r} \gg \bar{R}^*$ , they scale as  $\bar{t}/\bar{r}^3$ , consistent with the numerical results presented in Fig. 11 of the main text.

## V. Supplementary Movies

Here, we provide links and descriptions for movies referred to in the main text.

- Movie S1: <https://youtube.com/shorts/QFAwuHB3ACk>. A video of the mesh (unrefined), originally zoomed in with a length scale of  $\sim 10^{-1}$  centered at the transporter. In time, the video zooms out demonstrating the length scales involved in the problem and ends with the entire mesh shown on a length scale of  $\sim 10^6$ . The transporter is depicted in red, the membrane in blue, the structured interfacial region in gold, and the unstructured electrolyte solution in gray.
- Movie S2: <https://youtu.be/3kZTz5cyNl4>. A video depicting the charging dynamics for the salt concentration in the region  $|\bar{z}| \leq 15$  and  $\bar{r} \leq 20$  for time  $\bar{t} \leq 5$ , for the localized pumping problem. Parameters as in Fig. 5.
- Movie S3: <https://youtu.be/AVHCSiPRsUQ>. A video depicting the charging dynamics for the charge density in the region  $|\bar{z}| \leq 15$  and  $\bar{r} \leq 20$  for time  $\bar{t} \leq 5$ , for the localized pumping problem. Parameters as in Fig. 5.
- Movie S4: [https://youtu.be/u4\\_8NKB-Hzw](https://youtu.be/u4_8NKB-Hzw). A video depicting the charging dynamics for the electric potential in the region  $|\bar{z}| \leq 15$  and  $\bar{r} \leq 20$  for time  $\bar{t} \leq 5$ , for the localized pumping problem. Parameters as in Fig. 5.

## References

- [1] Milton Abramowitz and Irene A. Stegun. *Handbook of Mathematical Functions with Formulas, Graphs, and Mathematical Tables*. US Government Printing Office, 1968.

- [2] Martin S. Alnæs, Anders Logg, Kristian B. Ølgaard, Marie E. Rognes, and Garth N. Wells. Unified form language: A domain-specific language for weak formulations of partial differential equations. *ACM Transactions on Mathematical Software*, 40(2):1–37, 2014.
- [3] Patrick R. Amestoy, Alfredo Buttari, Jean-Yves L’excellent, and Theo Mary. Performance and scalability of the block low-rank multifrontal factorization on multicore architectures. *ACM Transactions on Mathematical Software*, 45(1):1–26, 2019.
- [4] Patrick R. Amestoy, Iain S. Duff, Jean-Yves L’Excellent, and Jacko Koster. A fully asynchronous multifrontal solver using distributed dynamic scheduling. *SIAM Journal on Matrix Analysis and Applications*, 23(1):15–41, 2001.
- [5] Howard C. Berg. *Random Walks in Biology*. Princeton University Press, 1993.
- [6] Christophe Geuzaine and Jean-François Remacle. Gmsh: A 3-d finite element mesh generator with built-in pre- and post-processing facilities. *International Journal for Numerical Methods in Engineering*, 79(11):1309–1331, 2009.
- [7] John D. Jackson. *Classical Electrodynamics*. John Wiley & Sons, 1999.
- [8] Panayiotis Papadopoulos. *Introduction to the Finite Element Method*. University of California, Berkeley, 2015.
- [9] J-F Remacle, Jonathan Lambrechts, Bruno Seny, Emilie Marchandise, Amaury Johnen, and C Geuzainet. Blossom-quad: A non-uniform quadrilateral mesh generator using a minimum-cost perfect-matching algorithm. *International Journal for Numerical Methods in Engineering*, 89(9):1102–1119, 2012.
- [10] Matthew W. Scroggs, Igor A. Baratta, Chris N. Richardson, and Garth N. Wells. Basix: a runtime finite element basis evaluation library. *Journal of Open Source Software*, 7(73):3982, 2022.
- [11] Matthew W. Scroggs, Jørgen S. Dokken, Chris N. Richardson, and Garth N. Wells. Construction of arbitrary order finite element degree-of-freedom maps on polygonal and polyhedral cell meshes. *ACM Transactions on Mathematical Software*, 48(2):1–23, 2022.
